# Supplementary material for: Almost complex structures in 6D with nondegenerate Nijenhuis tensors and large symmetry groups
Source: arXiv:1512.07161 ancillary file (2015-12-22)
Supplement: Supplementary file 1 [file All_Cohomology.pdf]

```
> restart:with(DifferentialGeometry):with(LieAlgebras):with(Tensor)
:with(Tools):
```

In this file we compute the cohomology  $H^*(g, m^* \otimes g)$  of solvable Lie subalgebras  $g$  of  $su(2,1)$ . The existence of nontrivial cohomology would indicate the existence of non-reductive homogeneous spaces which are Lie algebra extensions of  $(g,h)$ , i.e. without an invariant complement to  $h$ . When the cohomology is non-trivial, we also produce a matrix representation of the isotropy on the indecomposable module  $g$  by taking representatives of cohomology classes.

```
> RData:=SimpleLieAlgebraData("su(2,1)",R):DGsetup(RData):rho:=
StandardRepresentation(R);
```

$$\rho := \begin{bmatrix} \begin{bmatrix} I & 0 & 0 \\ 0 & I & 0 \\ 0 & 0 & -2I \end{bmatrix}, \begin{bmatrix} 1 & 0 & 0 \\ 0 & -1 & 0 \\ 0 & 0 & 0 \end{bmatrix}, \begin{bmatrix} 0 & 0 & 0 \\ 0 & 0 & 1 \\ -1 & 0 & 0 \end{bmatrix}, \begin{bmatrix} 0 & 0 & 1 \\ 0 & 0 & 0 \\ 0 & -1 & 0 \end{bmatrix}, \begin{bmatrix} 0 & 0 & 0 \\ I & 0 & 0 \\ 0 & 0 & 0 \end{bmatrix}, \begin{bmatrix} 0 & I & 0 \\ 0 & 0 & 0 \\ 0 & 0 & 0 \end{bmatrix}, \\ \begin{bmatrix} 0 & 0 & 0 \\ 0 & 0 & I \\ I & 0 & 0 \end{bmatrix}, \begin{bmatrix} 0 & 0 & I \\ 0 & 0 & 0 \\ 0 & I & 0 \end{bmatrix} \end{bmatrix} \quad (1)$$

These matrices give the tautological representation of  $su(2,1)$  on  $C^3$ .

```
> realify:=proc(In)
local n,N0,i,j,N;
n := LinearAlgebra[RowDimension](In):
N0 := Matrix(2*n):
for i to n do for j to n do N0[2*i, 2*j] := Re(In[i, j]) end do
end do; for i to n do for j to n do N0[2*i-1, 2*j] := -Im(In[i,
j]) end do end do; for i to n do for j to n do N0[2*i, 2*j-1] :=
Im(In[i, j]) end do end do; for i to n do for j to n do N0[2*i-1,
2*j-1] := Re(In[i, j]) end do end do:
N := RealDomain:-simplify(N0):
N
end proc:
```

This procedure takes a  $n \times n$  complex matrix and replaces all complex numbers with  $2 \times 2$  block matrices, yielding a  $2n \times 2n$  real matrix.

```
Cspace > R6Hook:=proc(In,k)
subs({seq(dx | i=0,i=1..6)},subs(dx | k=1,In));
end proc:
```

```
> DGsetup([seq(x | i,i=1..6)],R6);DGsetup([seq(r30_ | i,i=1..30)],
R30);DGsetup([seq(r24_ | i,i=1..24)],R24);DGsetup([seq(r18_ | i,i=
1..18)],R18);DGsetup([seq(v | i,i=1..10)],R10);DGsetup([seq
(r9_ | i,i=1..9)],R9);
```

*frame name: R6*

*frame name: R30*

*frame name: R24*

*frame name: R18*

*frame name: R10*

*frame name: R9*

(2)

## Part 1:

Isotropy algebra  $\mathfrak{h}$  of dimension 5. There is a unique choice of  $\mathfrak{h}$ .

```
> P:=MinimalSubalgebra([rho[1],rho[2],rho[3]]);
```

$$P := \left[ \begin{bmatrix} I & 0 & 0 \\ 0 & I & 0 \\ 0 & 0 & -2I \end{bmatrix}, \begin{bmatrix} 1 & 0 & 0 \\ 0 & -1 & 0 \\ 0 & 0 & 0 \end{bmatrix}, \begin{bmatrix} 0 & 0 & 0 \\ 0 & 0 & 1 \\ -1 & 0 & 0 \end{bmatrix}, \begin{bmatrix} 0 & 0 & 0 \\ 0 & 0 & 3I \\ 3I & 0 & 0 \end{bmatrix}, \begin{bmatrix} 0 & 0 & 0 \\ 6I & 0 & 0 \\ 0 & 0 & 0 \end{bmatrix} \right] \quad (3)$$

```
> pData:=LieAlgebraData(P,p):DGsetup(pData);
```

*Lie algebra: p*

(4)

```
> P_real:=map(realify,P):m_p:=Representation(p,R6,P_real):dm_p:=
TensorProductOfRepresentations(m_p,DGinfo(R6,"FrameBaseForms"),
R6);
```

$$dm_p := \left[ \begin{matrix} e1, \\ \begin{bmatrix} 0 & -1 & 0 & 0 & 0 & 0 \\ 1 & 0 & 0 & 0 & 0 & 0 \\ 0 & 0 & 0 & -1 & 0 & 0 \\ 0 & 0 & 1 & 0 & 0 & 0 \\ 0 & 0 & 0 & 0 & 0 & 2 \\ 0 & 0 & 0 & 0 & -2 & 0 \end{bmatrix} \end{matrix}, e2, \begin{bmatrix} -1 & 0 & 0 & 0 & 0 & 0 \\ 0 & -1 & 0 & 0 & 0 & 0 \\ 0 & 0 & 1 & 0 & 0 & 0 \\ 0 & 0 & 0 & 1 & 0 & 0 \\ 0 & 0 & 0 & 0 & 0 & 0 \\ 0 & 0 & 0 & 0 & 0 & 0 \end{bmatrix}, e3, \right. \quad (5)$$

$$\left. \begin{bmatrix} 0 & 0 & 0 & 0 & 1 & 0 \\ 0 & 0 & 0 & 0 & 0 & 1 \\ 0 & 0 & 0 & 0 & 0 & 0 \\ 0 & 0 & 0 & 0 & 0 & 0 \\ 0 & 0 & -1 & 0 & 0 & 0 \\ 0 & 0 & 0 & -1 & 0 & 0 \end{bmatrix}, e4, \begin{bmatrix} 0 & 0 & 0 & 0 & 0 & -3 \\ 0 & 0 & 0 & 0 & 3 & 0 \\ 0 & 0 & 0 & 0 & 0 & 0 \\ 0 & 0 & 0 & 0 & 0 & 0 \\ 0 & 0 & 0 & -3 & 0 & 0 \\ 0 & 0 & 3 & 0 & 0 & 0 \end{bmatrix}, e5, \begin{bmatrix} 0 & 0 & 0 & -6 & 0 & 0 \\ 0 & 0 & 6 & 0 & 0 & 0 \\ 0 & 0 & 0 & 0 & 0 & 0 \\ 0 & 0 & 0 & 0 & 0 & 0 \\ 0 & 0 & 0 & 0 & 0 & 0 \\ 0 & 0 & 0 & 0 & 0 & 0 \end{bmatrix} \right]$$

```
> ad_p:=Adjoint(p,representationspace=p);
```

$$ad_p := \left[ \begin{matrix} e1, \\ \begin{bmatrix} 0 & 0 & 0 & 0 & 0 \\ 0 & 0 & 0 & 0 & 0 \\ 0 & 0 & 0 & -9 & 0 \\ 0 & 0 & 1 & 0 & 0 \\ 0 & 0 & 0 & 0 & 0 \end{bmatrix} \end{matrix}, e2, \begin{bmatrix} 0 & 0 & 0 & 0 & 0 \\ 0 & 0 & 0 & 0 & 0 \\ 0 & 0 & -1 & 0 & 0 \\ 0 & 0 & 0 & -1 & 0 \\ 0 & 0 & 0 & 0 & -2 \end{bmatrix}, e3, \begin{bmatrix} 0 & 0 & 0 & 0 & 0 \\ 0 & 0 & 0 & 0 & 0 \\ 0 & 1 & 0 & 0 & 0 \\ -1 & 0 & 0 & 0 & 0 \\ 0 & 0 & 0 & 1 & 0 \end{bmatrix}, \right. \quad (6)$$

$$\left. e4, \begin{bmatrix} 0 & 0 & 0 & 0 & 0 \\ 0 & 0 & 0 & 0 & 0 \\ 9 & 0 & 0 & 0 & 0 \\ 0 & 1 & 0 & 0 & 0 \\ 0 & 0 & -1 & 0 & 0 \end{bmatrix}, e5, \begin{bmatrix} 0 & 0 & 0 & 0 & 0 \\ 0 & 0 & 0 & 0 & 0 \\ 0 & 0 & 0 & 0 & 0 \\ 0 & 0 & 0 & 0 & 0 \\ 0 & 2 & 0 & 0 & 0 \end{bmatrix} \right],$$

```
> dmtad_p:=TensorProductOfRepresentations([dm_p,ad_p],R30):
```

This tensor product is the coefficient space for our cohomology. The first factor is the realification of the restriction of the tautological representation, the second is the adjoint representation of P.

```
> DGsetup(p,dmtad_p,Cspace);
```

*Lie algebra with coefficients: Cspace*

(7)

```
> Chains:=RelativeChains([ ]):Cohomology(Chains[1..3]);
```

[[ ]]

(8)

The cohomology calculations are automatically understood to refer to the initialized Lie algebra and coefficient space. In this case the cohomology is trivial (the output is a basis consisting of representatives).

## Part 2:

Isotropy h of dimension 4. There is a one dimensional family of 4D subalgebras h of P. First we treat two special cases, then we check that there is no additional cohomology for generic parameter.

```
> R:=MinimalSubalgebra([P[2],P[3],P[4]]);
```

$$R := \left[ \begin{bmatrix} 1 & 0 & 0 \\ 0 & -1 & 0 \\ 0 & 0 & 0 \end{bmatrix}, \begin{bmatrix} 0 & 0 & 0 \\ 0 & 0 & 1 \\ -1 & 0 & 0 \end{bmatrix}, \begin{bmatrix} 0 & 0 & 0 \\ 0 & 0 & 3I \\ 3I & 0 & 0 \end{bmatrix}, \begin{bmatrix} 0 & 0 & 0 \\ 6I & 0 & 0 \\ 0 & 0 & 0 \end{bmatrix} \right]$$

(9)

**Part 2.1:** The 4D subalgebra which includes a diagonal matrix.

```
> rData:=LieAlgebraData(R,r):DGsetup(rData);
```

*Lie algebra: r*

(10)

```
> R_real:=map(realify,R):m_r:=Representation(r,R6,R_real):dm_r:=
TensorProductOfRepresentations(m_r,DGinfo(R6,"FrameBaseForms"),
R6);
```

$$dm_r := \left[ \begin{bmatrix} -1 & 0 & 0 & 0 & 0 & 0 \\ 0 & -1 & 0 & 0 & 0 & 0 \\ 0 & 0 & 1 & 0 & 0 & 0 \\ 0 & 0 & 0 & 1 & 0 & 0 \\ 0 & 0 & 0 & 0 & 0 & 0 \\ 0 & 0 & 0 & 0 & 0 & 0 \end{bmatrix}, \begin{bmatrix} 0 & 0 & 0 & 0 & 1 & 0 \\ 0 & 0 & 0 & 0 & 0 & 1 \\ 0 & 0 & 0 & 0 & 0 & 0 \\ 0 & 0 & 0 & 0 & 0 & 0 \\ 0 & 0 & -1 & 0 & 0 & 0 \\ 0 & 0 & 0 & -1 & 0 & 0 \end{bmatrix}, \begin{bmatrix} 0 & 0 & 0 & 0 & 0 & -3 \\ 0 & 0 & 0 & 0 & 3 & 0 \\ 0 & 0 & 0 & 0 & 0 & 0 \\ 0 & 0 & 0 & 0 & 0 & 0 \\ 0 & 0 & 0 & -3 & 0 & 0 \\ 0 & 0 & 3 & 0 & 0 & 0 \end{bmatrix}, \begin{bmatrix} 0 & 0 & 0 & -6 & 0 & 0 \\ 0 & 0 & 6 & 0 & 0 & 0 \\ 0 & 0 & 0 & 0 & 0 & 0 \\ 0 & 0 & 0 & 0 & 0 & 0 \\ 0 & 0 & 0 & 0 & 0 & 0 \\ 0 & 0 & 0 & 0 & 0 & 0 \end{bmatrix} \right],$$

(11)

```
> ad_r:=Adjoint(r,representationSpace=r);
```

$$ad_r := \left[ \begin{bmatrix} 0 & 0 & 0 & 0 \\ 0 & -1 & 0 & 0 \\ 0 & 0 & -1 & 0 \\ 0 & 0 & 0 & -2 \end{bmatrix}, \begin{bmatrix} 0 & 0 & 0 & 0 \\ 1 & 0 & 0 & 0 \\ 0 & 0 & 0 & 0 \\ 0 & 0 & 1 & 0 \end{bmatrix}, \begin{bmatrix} 0 & 0 & 0 & 0 \\ 0 & 0 & 0 & 0 \\ 1 & 0 & 0 & 0 \\ 0 & -1 & 0 & 0 \end{bmatrix}, \begin{bmatrix} 0 & 0 & 0 & 0 \\ 0 & 0 & 0 & 0 \\ 0 & 0 & 0 & 0 \\ 2 & 0 & 0 & 0 \end{bmatrix} \right] \quad (12)$$

```
> dmtad_r:=TensorProductOfRepresentations([dm_r,ad_r],R24):
```

This coefficient space is the tensor product of the realification of the restriction of the tautological representation and the adjoint representation of r.

```
> DGsetup(r,dmtad_r,Cspace);
```

*Lie algebra with coefficients: Cspace*

(13)

```
> Chains:=RelativeChains([ ]):H:=Cohomology(Chains[1..3]);
```

$$H := \left[ \left( \frac{4741 r_{24\_23}}{3877} + r_{24\_16} + \frac{14367 r_{24\_1}}{3877} \right) \theta_2 + \left( \frac{6357 r_{24\_22}}{3877} + \frac{6015 r_{24\_12}}{3877} - \frac{8533 r_{24\_5}}{3877} \right) \theta_3 + \left( \frac{5616 r_{24\_20}}{3877} - \frac{2176 r_{24\_6}}{3877} - \frac{144 r_{24\_3}}{3877} \right) \theta_4, \right. \\ \left. - \left( \frac{2671 r_{24\_22}}{5167} + \frac{2409 r_{24\_12}}{5167} - \frac{8627 r_{24\_5}}{5167} \right) \theta_2 + \left( \frac{6019 r_{24\_23}}{5167} + r_{24\_16} + \frac{7597 r_{24\_1}}{5167} \right) \theta_3 - \left( -\frac{5408 r_{24\_24}}{5167} + \frac{2608 r_{24\_7}}{5167} + \frac{416 r_{24\_2}}{5167} \right) \theta_4, \right. \\ \left( \frac{240 r_{24\_23}}{3877} + r_{24\_18} + \frac{760 r_{24\_1}}{3877} \right) \theta_2 + \left( \frac{10166 r_{24\_22}}{3877} + \frac{2317 r_{24\_12}}{3877} - \frac{7757 r_{24\_5}}{11631} \right) \theta_3 + \left( \frac{1560 r_{24\_20}}{3877} - \frac{12152 r_{24\_6}}{11631} - \frac{40 r_{24\_3}}{3877} \right) \theta_4, \\ \left. - \left( \frac{2581 r_{24\_22}}{5167} + \frac{1191 r_{24\_12}}{10334} - \frac{3493 r_{24\_5}}{10334} \right) \theta_2 + \left( \frac{2461 r_{24\_23}}{10334} + r_{24\_18} + \frac{1268 r_{24\_1}}{15501} \right) \theta_3 - \left( -\frac{436 r_{24\_24}}{5167} + \frac{516 r_{24\_7}}{5167} + \frac{6460 r_{24\_2}}{15501} \right) \theta_4, \right. \\ \left( \frac{72 r_{24\_22}}{5167} + r_{24\_19} + \frac{3935 r_{24\_12}}{10334} - \frac{14109 r_{24\_5}}{10334} \right) \theta_2 - \left( -\frac{11973 r_{24\_23}}{10334} + \frac{228 r_{24\_1}}{5167} \right) \theta_3 \\ \left. - \left( -\frac{156 r_{24\_24}}{5167} + \frac{2460 r_{24\_7}}{5167} + \frac{12 r_{24\_2}}{5167} \right) \theta_4, \left( -\frac{1791 r_{24\_23}}{3877} + \frac{144 r_{24\_1}}{3877} \right) \theta_2 + \left( \frac{1967 r_{24\_22}}{3877} + r_{24\_19} + \frac{1949 r_{24\_12}}{3877} - \frac{7877 r_{24\_5}}{11631} \right) \theta_3 \right. \\ \left. + \left( \frac{1928 r_{24\_20}}{3877} - \frac{1976 r_{24\_6}}{11631} - \frac{1640 r_{24\_3}}{3877} \right) \theta_4 \right] \quad (14)$$

```
Cspace > nops(H[1]);
```

(15)

We get a 6D cohomology. This is given in terms of abstract representatives, but we really need the representation matrices for the corresponding module. The following code produces such matrices.

```
Cspace > srule:=seq(r24_| |i=dx| |(ceil(i/4))*e| |(i-1 mod 4
+1),i=1..24):
Cspace > H_r:=[seq(subs(srule,H[1][i]),i=1..6)]:H_r:
r > mu:=add(u| |i*H_r[i],i=1..6):
Cspace > C:=(i,j,k)->Hook(evalDG(Hook(R6Hook(mu,j),e| |k)),
theta| |i):
Cspace > uMat:=DGinfo(DirectSumOfRepresentations([ad_r,m_r],
R10),"RepresentationMatrices"):
Cspace > for i to 4 do for j to 6 do for k to 4 do try uMat
[k][i,j+4]:=C(i,j,k) catch: end try end do end do
end do;
Cspace > uMat;
```

$$\begin{bmatrix} 0 & 0 & 0 & 0 & 0 & 0 & 0 & 0 & 0 & 0 \\ 0 & -1 & 0 & 0 & 0 & 0 & 0 & 0 & 0 & 0 \\ 0 & 0 & -1 & 0 & 0 & 0 & 0 & 0 & 0 & 0 \\ 0 & 0 & 0 & -2 & 0 & 0 & 0 & 0 & 0 & 0 \\ 0 & 0 & 0 & 0 & 1 & 0 & 0 & 0 & 0 & 0 \\ 0 & 0 & 0 & 0 & 0 & 1 & 0 & 0 & 0 & 0 \\ 0 & 0 & 0 & 0 & 0 & 0 & -1 & 0 & 0 & 0 \\ 0 & 0 & 0 & 0 & 0 & 0 & 0 & -1 & 0 & 0 \\ 0 & 0 & 0 & 0 & 0 & 0 & 0 & 0 & 0 & 0 \\ 0 & 0 & 0 & 0 & 0 & 0 & 0 & 0 & 0 & 0 \end{bmatrix}, \left[ \left[ 0, 0, 0, 0, \frac{14367}{3877} u_1 + \frac{760}{3877} u_3 + \frac{144}{3877} u_6, \right. \right. \quad (16)$$

$$\left. \frac{8627}{5167} u_2 + \frac{3493}{10334} u_4 - \frac{14109}{10334} u_5, 0, 0, 0, 0 \right],$$

$$\left[1, 0, 0, 0, 0, 0, 0, 0, 0, u_3, -\frac{2671}{5167} u_2 - \frac{2581}{5167} u_4 + \frac{72}{5167} u_5\right],$$

$$\left[0, 0, 0, 0, 0, 0, 0, 0, 0, u_5, \frac{4741}{3877} u_1 + \frac{240}{3877} u_3 - \frac{1791}{3877} u_6\right],$$

$$\left[0, 0, 1, 0, 0, 0, -\frac{2409}{5167} \, u2 - \frac{1191}{10334} \, u4 + \frac{3935}{10334} \, u5, uI, 0, 0\right],$$

$$\left[0, 0, 0, 0, 0, 0, 0, 0, 0, 0\right],$$

---


$$\left[ 0, 0, 0, 0, 0, 0, 0, 0, 0, 0, 0 \right],$$

$$\left[ 0, 0, 0, 0, 0, 0, 0, 0, 0, 1, 0 \right],$$



$$\left[0, 0, 0, 0, 0, 0, 0, 0, 0, 0, 1\right],$$

$$\left[0, 0, 0, 0, 0, -1, 0, 0, 0, 0, 0\right],$$

$$\left[0, 0, 0, 0, 0, -1, 0, 0, 0, 0\right]\Big], \left[\left[0, 0, 0, 0, \frac{7597}{5167} \, u2 + \frac{1268}{15501} \, u4 - \frac{228}{5167} \, u5, \right.\right. \\ \left.\left.- \frac{8533}{3877} \, u1 - \frac{7757}{11631} \, u3 - \frac{7877}{11631} \, u6, 0, 0, 0, 0\right]\right],$$

$$\left[0, 0, 0, 0, 0, 0, 0, 0, u_4, \frac{6357}{3877} u_1 + \frac{10166}{3877} u_3 + \frac{1967}{3877} u_6\right],$$

$$\left[1, 0, 0, 0, 0, 0, 0, 0, u_6, \frac{6019}{5167} u_2 + \frac{2461}{10334} u_4 + \frac{11973}{10334} u_5\right],$$

$$\left[0, -1, 0, 0, 0, 0, \frac{6015}{3877} \, u1 + \frac{2317}{3877} \, u3 + \frac{1949}{3877} \, u6, u2, 0, 0\right],$$

$$\left[0, 0, 0, 0, 0, 0, 0, 0, 0, 0\right],$$

---


$$\begin{bmatrix} 0, 0, 0, 0, 0, 0, 0, 0, 0, 0 \end{bmatrix},$$

$$\begin{bmatrix} 0, 0, 0, 0, 0, 0, 0, 0, 0, -3 \end{bmatrix},$$

$$\left[ 0, 0, 0, 0, 0, 0, 0, 0, 3, 0 \right],$$

$$\left[ 0, 0, 0, 0, 0, -3, 0, 0, 0, 0 \right],$$

$$\left[ 0, 0, 0, 0, 3, 0, 0, 0, 0, 0 \right] \Big], \left[ \left[ 0, 0, 0, 0, 0, 0, 0, 0, 0, 0 \right], \right. \\ \left[ 0, 0, 0, 0, -\frac{416}{5167} u_2 - \frac{6460}{15501} u_4 - \frac{12}{5167} u_5, -\frac{2176}{3877} u_1 - \frac{12152}{11631} u_3 - \frac{1976}{11631} u_6, \right. \\ \left. 0, 0, 0, 0 \right], \\ \left[ 0, 0, 0, 0, -\frac{144}{3877} u_1 - \frac{40}{3877} u_3 - \frac{1640}{3877} u_6, -\frac{2608}{5167} u_2 - \frac{516}{5167} u_4 - \frac{2460}{5167} u_5, 0, \right. \\ \left. 0, 0, 0 \right], \\ \left[ 2, 0, 0, 0, 0, 0, 0, 0, \frac{5616}{3877} u_1 + \frac{1560}{3877} u_3 + \frac{1928}{3877} u_6, \frac{5408}{5167} u_2 + \frac{436}{5167} u_4 \right.$$

$$\begin{aligned}
& + \frac{156}{5167} u_5 \Big], \\
& \begin{bmatrix} 0, 0, 0, 0, 0, 0, 0, 0, 0, 0 \end{bmatrix}, \\
& \begin{bmatrix} 0, 0, 0, 0, 0, 0, 0, 0, 0, 0 \end{bmatrix}, \\
& \begin{bmatrix} 0, 0, 0, 0, 0, -6, 0, 0, 0, 0 \end{bmatrix}, \\
& \begin{bmatrix} 0, 0, 0, 0, 6, 0, 0, 0, 0, 0 \end{bmatrix}, \\
& \begin{bmatrix} 0, 0, 0, 0, 0, 0, 0, 0, 0, 0 \end{bmatrix}, \\
& \begin{bmatrix} 0, 0, 0, 0, 0, 0, 0, 0, 0, 0 \end{bmatrix} \Big] \Big] \Big]
\end{aligned}$$

These matrices represent the most general r-module g with g/r=m and g indecomposable, up to change of basis. The parameters  $u_i$  give the cohomology class, with  $u_i=0$  corresponding to the decomposable case (the matrices are visibly block diagonal in this case). We export the matrices to another file to look for Lie algebra structures on the module g.

```
> R:=MinimalSubalgebra([P[1],P[3],P[4]]);
```

$$R := \left[ \begin{bmatrix} I & 0 & 0 \\ 0 & I & 0 \\ 0 & 0 & -2I \end{bmatrix}, \begin{bmatrix} 0 & 0 & 0 \\ 0 & 0 & 1 \\ -1 & 0 & 0 \end{bmatrix}, \begin{bmatrix} 0 & 0 & 0 \\ 0 & 0 & 3I \\ 3I & 0 & 0 \end{bmatrix}, \begin{bmatrix} 0 & 0 & 0 \\ 6I & 0 & 0 \\ 0 & 0 & 0 \end{bmatrix} \right] \quad (17)$$

**Part 2.2:** This is another special choice, because it is the only 4D isotropy to feature a compact subalgebra (the first basis element spans this).

```
> rData:=LieAlgebraData(R,r):DGsetup(rData);
```

*Lie algebra: r*

(18)

```
> R_real:=map(realify,R):m_r:=Representation(r,R6,R_real):dm_r:=
TensorProductOfRepresentations(m_r,DGinfo(R6,"FrameBaseForms"),
R6);
```

$$dm_r := \left[ \begin{bmatrix} 0 & -1 & 0 & 0 & 0 & 0 \\ 1 & 0 & 0 & 0 & 0 & 0 \\ 0 & 0 & 0 & -1 & 0 & 0 \\ 0 & 0 & 1 & 0 & 0 & 0 \\ 0 & 0 & 0 & 0 & 0 & 2 \\ 0 & 0 & 0 & 0 & -2 & 0 \end{bmatrix}, \begin{bmatrix} 0 & 0 & 0 & 0 & 1 & 0 \\ 0 & 0 & 0 & 0 & 0 & 1 \\ 0 & 0 & 0 & 0 & 0 & 0 \\ 0 & 0 & 0 & 0 & 0 & 0 \\ 0 & 0 & -1 & 0 & 0 & 0 \\ 0 & 0 & 0 & -1 & 0 & 0 \end{bmatrix}, \begin{bmatrix} 0 & 0 & 0 & 0 & 1 & 0 \\ 0 & 0 & 0 & 0 & 0 & 1 \\ 0 & 0 & 0 & 0 & 0 & 0 \\ 0 & 0 & 0 & 0 & 0 & 0 \\ 0 & 0 & -1 & 0 & 0 & 0 \\ 0 & 0 & 0 & -1 & 0 & 0 \end{bmatrix} \right] e1, e2, e3, \quad (19)$$

$$\begin{aligned}
& \left[ \begin{array}{cccccc} 0 & 0 & 0 & 0 & 0 & -3 \\ 0 & 0 & 0 & 0 & 3 & 0 \\ 0 & 0 & 0 & 0 & 0 & 0 \\ 0 & 0 & 0 & 0 & 0 & 0 \\ 0 & 0 & 0 & -3 & 0 & 0 \\ 0 & 0 & 3 & 0 & 0 & 0 \end{array} \right], e4, \left[ \begin{array}{cccccc} 0 & 0 & 0 & -6 & 0 & 0 \\ 0 & 0 & 6 & 0 & 0 & 0 \\ 0 & 0 & 0 & 0 & 0 & 0 \\ 0 & 0 & 0 & 0 & 0 & 0 \\ 0 & 0 & 0 & 0 & 0 & 0 \\ 0 & 0 & 0 & 0 & 0 & 0 \end{array} \right], \\
& ad_r := \left[ \left[ \begin{array}{cccc} 0 & 0 & 0 & 0 \\ 0 & 0 & -9 & 0 \\ 0 & 1 & 0 & 0 \\ 0 & 0 & 0 & 0 \end{array} \right], e1, \left[ \begin{array}{cccc} 0 & 0 & 0 & 0 \\ 0 & 0 & 0 & 0 \\ -1 & 0 & 0 & 0 \\ 0 & 0 & 1 & 0 \end{array} \right], e2, \left[ \begin{array}{cccc} 0 & 0 & 0 & 0 \\ 9 & 0 & 0 & 0 \\ 0 & 0 & 0 & 0 \\ 0 & -1 & 0 & 0 \end{array} \right], e3, \left[ \begin{array}{cccc} 0 & 0 & 0 & 0 \\ 0 & 0 & 0 & 0 \\ 0 & 0 & 0 & 0 \\ 0 & 0 & 0 & 0 \end{array} \right], e4, \right. \\
& \left. \left[ \begin{array}{cccc} 0 & 0 & 0 & 0 \\ 0 & 0 & 0 & 0 \\ 0 & 0 & 0 & 0 \\ 0 & 0 & 0 & 0 \end{array} \right] \right]
\end{aligned} \tag{20}$$

```
> dmtad_r:=TensorProductOfRepresentations([dm_r,ad_r],R24);
```

This coefficient space is the tensor product of the realification of the restriction of the tautological representation and the adjoint representation of r.

```
> DGsetup(r,dmtad_r,Cspace);
Lie algebra with coefficients: Cspace
```

```
> Chains:=RelativeChains([ ]):Cohomology(Chains[1..3]);
[[ ]]
```

The cohomology is trivial in this case.

```
> R:=MinimalSubalgebra([a*P[1]+b*P[2],P[3],P[4]]);
```

$$R := \left[ \begin{array}{ccc} Ia+b & 0 & 0 \\ 0 & Ia-b & 0 \\ 0 & 0 & -2Ia \end{array} \right], \left[ \begin{array}{ccc} 0 & 0 & 0 \\ 0 & 0 & 1 \\ -1 & 0 & 0 \end{array} \right], \left[ \begin{array}{ccc} 0 & 0 & 0 \\ 0 & 0 & 3I \\ 3I & 0 & 0 \end{array} \right], \left[ \begin{array}{ccc} 0 & 0 & 0 \\ 6I & 0 & 0 \\ 0 & 0 & 0 \end{array} \right] \tag{23}$$

**Part 2.3:** Now we consider 4D isotropy for general parameter. We use two parameters (a,b) for convenience, but they are not allowed to simultaneously vanish, and the algebras given by scaling them simultaneously are equivalent.

```
> rData:=LieAlgebraData(R,r):DGsetup(rData);
Lie algebra: r
```

```
> R_real:=map(realify,R):m_r:=Representation(r,R6,R_real):dm_r:=
TensorProductOfRepresentations(m_r,DGinfo(R6,"FrameBaseForms"),
```

$$\begin{aligned}
& R6); \\
dm\_r := & \left[ \begin{matrix} e1, \\ \begin{bmatrix} -b & -a & 0 & 0 & 0 & 0 \\ a & -b & 0 & 0 & 0 & 0 \\ 0 & 0 & b & -a & 0 & 0 \\ 0 & 0 & a & b & 0 & 0 \\ 0 & 0 & 0 & 0 & 0 & 2a \\ 0 & 0 & 0 & 0 & -2a & 0 \end{bmatrix} \end{matrix} \right], e2, \left[ \begin{matrix} \begin{bmatrix} 0 & 0 & 0 & 0 & 1 & 0 \\ 0 & 0 & 0 & 0 & 0 & 1 \\ 0 & 0 & 0 & 0 & 0 & 0 \\ 0 & 0 & 0 & 0 & 0 & 0 \\ 0 & 0 & -1 & 0 & 0 & 0 \\ 0 & 0 & 0 & -1 & 0 & 0 \end{bmatrix} \end{matrix} \right], e3, \\
& \left[ \begin{matrix} \begin{bmatrix} 0 & 0 & 0 & 0 & 0 & -3 \\ 0 & 0 & 0 & 0 & 3 & 0 \\ 0 & 0 & 0 & 0 & 0 & 0 \\ 0 & 0 & 0 & 0 & 0 & 0 \\ 0 & 0 & 0 & -3 & 0 & 0 \\ 0 & 0 & 3 & 0 & 0 & 0 \end{bmatrix} \end{matrix} \right], e4, \left[ \begin{matrix} \begin{bmatrix} 0 & 0 & 0 & -6 & 0 & 0 \\ 0 & 0 & 6 & 0 & 0 & 0 \\ 0 & 0 & 0 & 0 & 0 & 0 \\ 0 & 0 & 0 & 0 & 0 & 0 \\ 0 & 0 & 0 & 0 & 0 & 0 \\ 0 & 0 & 0 & 0 & 0 & 0 \end{bmatrix} \end{matrix} \right],
\end{aligned} \tag{25}$$

```

> ad_r:=Adjoint(r,representationSpace=r):
> dmtad_r:=TensorProductOfRepresentations([dm_r,ad_r],R24):

```

This coefficient space is the tensor product of the realification of the restriction of the tautological representation and the adjoint representation of r.

```

> DGsetup(r,dmtad_r,Cspace);
Lie algebra with coefficients: Cspace

```

(26)

Since we have parameters in our representation and Lie algebra, we cannot use the Cohomology() command directly in this case. Instead, we need to look for parameters where the rank of the exterior derivative changes, besides a=0 and b=0 which were already treated as special cases (so we may assume a\*b nonzero).

```

> Chains:=RelativeChains([]):
Cspace > genericimageh0:=ExteriorDerivative(evalDG(add(h|i*
Chains[1][i],i=1..nops(Chains[1])))):
Cspace > genericimageh1:=ExteriorDerivative(evalDG(add(k|i*
Chains[2][i],i=1..nops(Chains[2])))):
Cspace > eq1:=DGinfo(genericimageh1,"CoefficientSet"):nops
(eq1);
6

```

(27)

```

Cspace > coeffeq1:={seq(coeffs(collect(eq1[i],Chains[1]),
Chains[1]),i=1..6)}:
Cspace > eqsols:=solve(coeffeq1):
Cspace > nops([eqsols]);
6

```

(28)

```

Cspace > generickernelh1:=DGsimplify(subs(eqsols[4],evalDG
(add(k|i*Chains[2][i],i=1..nops(Chains[2])))):
Cspace > coeffset:=DGinfo(evalDG(generickernelh1-
genericimageh0),"CoefficientSet"):

```



```
Cspace > nops(coeffset);
```

4

(29)

```
Cspace > finaleq:={seq(coeffs(collect(coeffset[i],Chains[1]),Chains[1]),i=1..4)}:
```

```
Cspace > solve(finaleq,[seq(h||i,i=1..nops(Chains[1]))]);
```

$$\left[ \begin{aligned} h1 &= \frac{1}{24} \frac{6 k17 + 3 k32 + 2 k7 - 6 k95}{a}, h2 = \\ &= -\frac{1}{2} \frac{2 a^2 k15 + 2 b^2 k15 + 3 a k77 - 3 b k93}{a^2 + b^2}, h3 \\ &= \frac{1}{2} \frac{2 a^2 k14 + 2 b^2 k14 + a k93 + b k77}{a^2 + b^2}, h4 = \frac{a k29 - 3 b k13}{a^2 + 9 b^2}, h5 = \\ &= -\frac{1}{24} \frac{18 k17 - 3 k32 - 2 k7 + 6 k95}{b}, h6 = \\ &= -\frac{1}{2} \frac{2 a^2 k31 + 2 b^2 k31 + 3 a k93 + 3 b k77}{a^2 + b^2}, h7 \\ &= \frac{1}{2} \frac{2 a^2 k30 + 2 b^2 k30 - a k77 + b k93}{a^2 + b^2}, h8 = -\frac{a k13 + 3 b k29}{a^2 + 9 b^2}, h9 = \frac{1}{3} k83, h10 \\ &= b k2 - k70, h11 = \frac{1}{9} k3 b + \frac{1}{3} k91, h12 = \frac{1}{4} k17 + \frac{1}{8} k32 - \frac{1}{36} k7 + \frac{1}{12} k95, h13 = \\ &= -k82, h14 = -\frac{1}{3} k3 b - k86, h15 = \frac{1}{3} k2 b - \frac{1}{3} k75, h16 = \\ &= -\frac{1}{72} \frac{24 a k6 + 24 a k79 - 6 b k17 - 3 b k32 - 2 b k7 + 6 b k95}{a}, h17 = k2, h18 \\ &= \frac{1}{24} \frac{24 a k6 - 6 b k17 - 3 b k32 - 2 b k7 + 6 b k95}{a}, h19 = \frac{1}{4} k17 + \frac{1}{8} k32 - \frac{1}{36} k7 \\ &+ \frac{1}{12} k95 + k78, h20 = -\frac{1}{2} \frac{a k93 + b k77}{a^2 + b^2}, h21 = -\frac{1}{3} k3, h22 = \frac{3}{4} k17 + \frac{3}{8} k32 \\ &- \frac{1}{12} k7 - \frac{3}{4} k95, h23 = \\ &= -\frac{1}{72} \frac{24 a k6 + 24 a k79 - 72 a k94 - 6 b k17 - 3 b k32 - 2 b k7 + 6 b k95}{a}, h24 \\ &= \frac{1}{2} \frac{a k77 - b k93}{a^2 + b^2} \end{aligned} \right]$$

These equations express a basis of cocycles as a linear combination of coboundaries. Hence the cohomology is trivial. The assumption used is  $a \cdot b$  nonzero, as our solution requires division by  $a$ ,  $b$  and homogeneous quadratic polynomials in these.

### Part 3:

Isotropy algebra  $h$  of dimension 3. There are 3 inequivalent choices, which are labeled by the

dimension of the intersection between them and the Cartan subalgebra of  $\mathfrak{su}(2,1)$ .

```
> L0:=MinimalSubalgebra([P[3],P[4]]);
```

$$L0 := \left[ \begin{bmatrix} 0 & 0 & 0 \\ 0 & 0 & 1 \\ -1 & 0 & 0 \end{bmatrix}, \begin{bmatrix} 0 & 0 & 0 \\ 0 & 0 & 3I \\ 3I & 0 & 0 \end{bmatrix}, \begin{bmatrix} 0 & 0 & 0 \\ 6I & 0 & 0 \\ 0 & 0 & 0 \end{bmatrix} \right] \quad (31)$$

**Part 3.1:** The case of 0D-intersection between  $\mathfrak{h}$  and the Cartan subalgebra.

```
> l0Data:=LieAlgebraData(L0,l0);DGsetup(l0Data);
```

$l0Data := [[e1, e2] = e3]$

*Lie algebra: l0*

(32)

```
> L0_real:=map(realify,L0):m_l0:=Representation(l0,R6,L0_real)
:dm_l0:=TensorProductOfRepresentations(m_l0,DGinfo(R6,
"FrameBaseForms"),R6);
```

$$dm_{l0} := \left[ \begin{matrix} e1, \begin{bmatrix} 0 & 0 & 0 & 0 & 1 & 0 \\ 0 & 0 & 0 & 0 & 0 & 1 \\ 0 & 0 & 0 & 0 & 0 & 0 \\ 0 & 0 & 0 & 0 & 0 & 0 \\ 0 & 0 & -1 & 0 & 0 & 0 \\ 0 & 0 & 0 & -1 & 0 & 0 \end{bmatrix}, e2, \begin{bmatrix} 0 & 0 & 0 & 0 & 0 & -3 \\ 0 & 0 & 0 & 0 & 3 & 0 \\ 0 & 0 & 0 & 0 & 0 & 0 \\ 0 & 0 & 0 & 0 & 0 & 0 \\ 0 & 0 & 0 & -3 & 0 & 0 \\ 0 & 0 & 3 & 0 & 0 & 0 \end{bmatrix}, e3, \begin{bmatrix} 0 & 0 & 0 & -6 & 0 & 0 \\ 0 & 0 & 6 & 0 & 0 & 0 \\ 0 & 0 & 0 & 0 & 0 & 0 \\ 0 & 0 & 0 & 0 & 0 & 0 \\ 0 & 0 & 0 & 0 & 0 & 0 \\ 0 & 0 & 0 & 0 & 0 & 0 \end{bmatrix} \end{matrix} \right], \quad (33)$$

```
> ad_l0:=Adjoint(l0,representationspace=l0);
```

$$ad_{l0} := \left[ \begin{matrix} e1, \begin{bmatrix} 0 & 0 & 0 \\ 0 & 0 & 0 \\ 0 & 1 & 0 \end{bmatrix}, e2, \begin{bmatrix} 0 & 0 & 0 \\ 0 & 0 & 0 \\ -1 & 0 & 0 \end{bmatrix}, e3, \begin{bmatrix} 0 & 0 & 0 \\ 0 & 0 & 0 \\ 0 & 0 & 0 \end{bmatrix} \end{matrix} \right] \quad (34)$$

```
> dmtad_l0:=TensorProductOfRepresentations([dm_l0,ad_l0],R18):
```

This coefficient space is the tensor product of the realification of the restriction of the tautological representation and the adjoint representation of  $l0$ .

```
> DGsetup(l0,dmtad_l0,Cspace);
```

*Lie algebra with coefficients: Cspace*

(35)

```
> Chains:=RelativeChains([ ]):H:=Cohomology(Chains[1..3]);
```

(36)

$$\begin{aligned}
H := & \left[ \left( r18\_14 + \frac{389 r18\_9}{6050} \right) \theta_1 + \left( \frac{12729 r18\_17}{6050} - \frac{423 r18\_13}{6050} + \frac{3807 r18\_12}{6050} \right) \theta_2 \right. \\
& - \left( -\frac{141 r18\_18}{110} + \frac{5421 r18\_5}{6050} + \frac{423 r18\_1}{6050} \right) \theta_3, \left( -\frac{55 r18\_17}{117} - \frac{55 r18\_13}{39} \right. \\
& + \left. \frac{8 r18\_12}{117} \right) \theta_1 + \left( -3 r18\_16 + r18\_14 - \frac{8 r18\_9}{39} \right) \theta_2 - \left( -\frac{16 r18\_4}{13} \right. \\
& + \left. \frac{16 r18\_2}{39} \right) \theta_3, -\left( \frac{r18\_17}{117} - \frac{4243 r18\_13}{1833} + \frac{19 r18\_12}{117} \right) \theta_1 + \left( \frac{234 r18\_16}{47} \right. \\
& + \left. \frac{1517 r18\_9}{1833} \right) \theta_2 + \left( r18\_15 - \frac{1201 r18\_4}{611} - \frac{r18\_2}{39} \right) \theta_3, \left( r18\_16 \right. \\
& + \left. \frac{423 r18\_9}{6050} \right) \theta_1 + \left( -\frac{47 r18\_17}{6050} - \frac{13011 r18\_13}{6050} + \frac{2149 r18\_12}{6050} \right) \theta_2 \\
& + \left( \frac{47 r18\_18}{110} - \frac{47 r18\_5}{6050} + \frac{5139 r18\_1}{6050} \right) \theta_3, \frac{9 r18\_4}{5} \theta_1 + \left( -\frac{6 r18\_18}{5} \right. \\
& + r18\_1 \theta_2 + \frac{3 r18\_6}{5} \theta_3, -\left( r18\_15 + \frac{19 r18\_4}{15} - r18\_2 \right) \theta_1 - \frac{19 r18\_18}{15} \theta_2 \\
& + \frac{7 r18\_6}{15} \theta_3, \left( -\frac{3 r18\_18}{7} + \frac{24 r18\_5}{7} + \frac{r18\_1}{7} \right) \theta_1 + \left( \frac{r18\_15}{7} + r18\_2 \right) \theta_2, -\left( \right. \\
& - \frac{15 r18\_18}{7} + \frac{15 r18\_5}{7} + \frac{19 r18\_1}{7} \theta_1 - \frac{19 r18\_15}{7} \theta_2 + r18\_3 \theta_3, -\left( -\frac{9 r18\_18}{7} \right. \\
& + \frac{9 r18\_5}{7} + \frac{24 r18\_1}{7} \theta_1 - \left( \frac{3 r18\_15}{7} - r18\_4 \right) \theta_2, -\left( 3 r18\_15 + \frac{21 r18\_4}{5} \right) \theta_1 \\
& \left. - \left( \frac{21 r18\_18}{5} - r18\_5 \right) \theta_2 + \frac{8 r18\_6}{5} \theta_3 \right]
\end{aligned}$$

**Cspace > nops(H[1]);**

10

(37)

We find that the cohomology is 10D, and the above is a basis given in terms of representatives. The following code converts the representatives to representation matrices of indecomposable modules.

**Cspace > srule:=seq(r18\_| |i=dx| |(ceil(i/3))\*e| |(i-1 mod 3 +1),i=1..18):**

**Cspace > H\_r:=seq(subs(srule,H[1][i]),i=1..10):H\_r:**

**r > mu:=add(u| |i\*H\_r[i],i=1..10):**

**Cspace > C:=(i,j,k)->Hook(evalDG(Hook(R6Hook(mu,j),e| |k)), theta| |i):**

**Cspace > uMat:=DGinfo(DirectSumOfRepresentations([ad\_10, m\_10],R9),"RepresentationMatrices"):**

**Cspace > for i to 3 do for j to 6 do for k to 3 do try uMat [k][i,j+3]:=C(i,j,k) catch: end try end do end do**

**Cspace > uMat;**

$$\begin{aligned}
& \left[ \left[ \left[ 0, 0, 0, \frac{1}{7} u_7 - \frac{19}{7} u_8 - \frac{24}{7} u_9, \frac{9}{5} u_5 - \frac{19}{15} u_6 - \frac{21}{5} u_{10}, 0, 0, -\frac{55}{39} u_2 + \frac{4243}{1833} u_3, \right. \right. \right. \\
& \left. \left. \left. u_4 \right], \right. \right.
\end{aligned}$$

(38)

$$\left[0, 0, 0, u_6, \frac{24}{7} u_7 - \frac{15}{7} u_8 - \frac{9}{7} u_9, 0, 0, u_1, -\frac{55}{117} u_2 - \frac{1}{117} u_3\right],$$

$$\left[0, 1, 0, 0, 0, \frac{389}{6050} u_1 + \frac{423}{6050} u_4, \frac{8}{117} u_2 - \frac{19}{117} u_3, -u_6 - 3 u_{10}, -\frac{3}{7} u_7 + \frac{15}{7} u_8 + \frac{9}{7} u_9\right],$$

$$\left[0, 0, 0, 0, 0, 0, 0, 0, 0, 0\right],$$

---


$$\begin{bmatrix} 0, 0, 0, 0, 0, 0, 0, 0, 0 \end{bmatrix},$$

$$\begin{bmatrix} 0, 0, 0, 0, 0, 0, 0, 1, 0 \end{bmatrix},$$

$$\begin{bmatrix} 0, 0, 0, 0, 0, 0, 0, 0, 1 \end{bmatrix},$$

$$\begin{bmatrix} 0, 0, 0, -1, 0, 0, 0, 0, 0 \end{bmatrix},$$

$$\begin{bmatrix} 0, 0, 0, 0, -1, 0, 0, 0, 0 \end{bmatrix}, \left[ \begin{bmatrix} 0, 0, 0, u5, u9, 0, 0, -\frac{423}{6050} u1 - \frac{13011}{6050} u4, -3 u2 \right. \right. \\ \left. \left. + \frac{234}{47} u3 \right], \right.$$

$$\begin{bmatrix} 0, 0, 0, u7, u10, 0, 0, u2, \frac{12729}{6050} u1 - \frac{47}{6050} u4 \end{bmatrix},$$

$$\begin{bmatrix} -1, 0, 0, 0, 0, -\frac{8}{39} u2 + \frac{1517}{1833} u3, \frac{3807}{6050} u1 + \frac{2149}{6050} u4, \frac{1}{7} u7 - \frac{19}{7} u8 - \frac{3}{7} u9, \\ -\frac{6}{5} u5 - \frac{19}{15} u6 - \frac{21}{5} u10 \end{bmatrix},$$

---


$$\begin{bmatrix} 0, 0, 0, 0, 0, 0, 0, 0, 0 \end{bmatrix},$$

$$\begin{bmatrix} 0, 0, 0, 0, 0, 0, 0, 0, 0 \end{bmatrix},$$

$$\begin{bmatrix} 0, 0, 0, 0, 0, 0, 0, 0, -3 \end{bmatrix},$$

---


$$\begin{bmatrix} 0, 0, 0, 0, 0, 0, 0, 3, 0 \end{bmatrix},$$

$$\begin{bmatrix} 0, 0, 0, 0, -3, 0, 0, 0, 0 \end{bmatrix},$$

$$\begin{bmatrix} 0, 0, 0, 3, 0, 0, 0, 0, 0 \end{bmatrix}],$$



$$\begin{aligned}
& \left[ \left[ 0, 0, 0, -\frac{423}{6050} u1 + \frac{5139}{6050} u4, \frac{16}{13} u2 - \frac{1201}{611} u3, 0, 0, 0, 0 \right], \right. \\
& \left[ 0, 0, 0, -\frac{16}{39} u2 - \frac{1}{39} u3, -\frac{5421}{6050} u1 - \frac{47}{6050} u4, 0, 0, 0, 0 \right], \\
& \left[ 0, 0, 0, u8, \frac{3}{5} u5 + \frac{7}{15} u6 + \frac{8}{5} u10, 0, 0, u3, \frac{141}{110} u1 + \frac{47}{110} u4 \right], \\
& \left[ 0, 0, 0, 0, 0, 0, 0, 0, 0 \right], \\
& \left[ 0, 0, 0, 0, 0, 0, 0, 0, 0 \right], \\
& \left[ 0, 0, 0, 0, -6, 0, 0, 0, 0 \right], \\
& \left[ 0, 0, 0, 6, 0, 0, 0, 0, 0 \right], \\
& \left[ 0, 0, 0, 0, 0, 0, 0, 0, 0 \right], \\
& \left. \left[ 0, 0, 0, 0, 0, 0, 0, 0, 0 \right] \right]
\end{aligned}$$

These matrices represent the most general 10-module  $g$  with  $g/10=m$  and  $g$  indecomposable, up to change of basis. The parameters  $u_i$  give the cohomology class, with  $u_i=0$  corresponding to the decomposable case (the matrices are visibly block diagonal in this case). We export the matrices to another file to look for Lie algebra structures on the module  $g$ .

```
> L1:=MinimalSubalgebra([P[2],P[3],P[5]]);
```

$$L1 := \left[ \begin{bmatrix} 1 & 0 & 0 \\ 0 & -1 & 0 \\ 0 & 0 & 0 \end{bmatrix}, \begin{bmatrix} 0 & 0 & 0 \\ 0 & 0 & 1 \\ -1 & 0 & 0 \end{bmatrix}, \begin{bmatrix} 0 & 0 & 0 \\ 6I & 0 & 0 \\ 0 & 0 & 0 \end{bmatrix} \right] \quad (39)$$

**Part 3.2:** The intersection of  $h$  and the Cartan subalgebra is 1D.

```
> l1Data:=LieAlgebraData(L1,l1):DGsetup(l1Data);
```

*Lie algebra: l1* (40)

```
> L1_real:=map(realify,L1):m_l1:=Representation(l1,R6,L1_real)
:dm_l1:=TensorProductOfRepresentations(m_l1,DGinfo(R6,
"FrameBaseForms"),R6);
```

$$dm_{l1} := \left[ \begin{matrix} e1, \\ \begin{bmatrix} -1 & 0 & 0 & 0 & 0 & 0 \\ 0 & -1 & 0 & 0 & 0 & 0 \\ 0 & 0 & 1 & 0 & 0 & 0 \\ 0 & 0 & 0 & 1 & 0 & 0 \\ 0 & 0 & 0 & 0 & 0 & 0 \\ 0 & 0 & 0 & 0 & 0 & 0 \end{bmatrix} \end{matrix} \right], \left[ \begin{matrix} e2, \\ \begin{bmatrix} 0 & 0 & 0 & 0 & 1 & 0 \\ 0 & 0 & 0 & 0 & 0 & 1 \\ 0 & 0 & 0 & 0 & 0 & 0 \\ 0 & 0 & 0 & 0 & 0 & 0 \\ 0 & 0 & -1 & 0 & 0 & 0 \\ 0 & 0 & 0 & -1 & 0 & 0 \end{bmatrix} \end{matrix} \right], \left[ \begin{matrix} e3, \end{matrix} \right] \quad (41)$$

$$\begin{bmatrix} 0 & 0 & 0 & -6 & 0 & 0 \\ 0 & 0 & 6 & 0 & 0 & 0 \\ 0 & 0 & 0 & 0 & 0 & 0 \\ 0 & 0 & 0 & 0 & 0 & 0 \\ 0 & 0 & 0 & 0 & 0 & 0 \\ 0 & 0 & 0 & 0 & 0 & 0 \end{bmatrix},$$

```
> ad_l1:=Adjoint(l1,representationspace=l1);
```

$$ad_{l1} := \left[ \left[ e1, \begin{bmatrix} 0 & 0 & 0 \\ 0 & -1 & 0 \\ 0 & 0 & -2 \end{bmatrix} \right], \left[ e2, \begin{bmatrix} 0 & 0 & 0 \\ 1 & 0 & 0 \\ 0 & 0 & 0 \end{bmatrix} \right], \left[ e3, \begin{bmatrix} 0 & 0 & 0 \\ 0 & 0 & 0 \\ 2 & 0 & 0 \end{bmatrix} \right] \right] \quad (42)$$

```
> dmtad_l1:=TensorProductOfRepresentations([dm_l1,ad_l1],R18):
```

This coefficient space is the tensor product of the realification of the restriction of the tautological representation and the adjoint representation of l1.

```
> DGsetup(l1,dmtad_l1,Cspace);
```

*Lie algebra with coefficients: Cspace*

(43)

```
> Chains:=RelativeChains([ ]):H:=Cohomology(Chains[1..3]);
```

$$H := \left[ \left[ -\left(6r18_{17} - \frac{6r18_{4}}{5}\right) \theta_2 + \left(\frac{12r18_{18}}{5} + r18_{2}\right) \theta_3, -\left(-6r18_{14} + \frac{6r18_{1}}{5}\right) \theta_2 - \left(\frac{12r18_{15}}{5} - r18_{5}\right) \theta_3, -\left(-r18_{9} + \frac{12r18_{4}}{5}\right) \theta_2 + \frac{6r18_{18}}{5} \theta_3, \left(r18_{12} + \frac{12r18_{1}}{5}\right) \theta_2 - \frac{6r18_{15}}{5} \theta_3 \right] \right] \quad (44)$$

```
Cspace > nops(H[1]);
```

4

(45)

We find that the cohomology is 4D, and the above is a basis given in terms of representatives. The following code converts the representatives to representation matrices of indecomposable modules.

```
Cspace > srule:=seq(r18_|i=dx|(ceil(i/3))*e|(i-1 mod 3 +1),i=1..18):
```

```
Cspace > H_r:=seq(subs(srule,H[1][i]),i=1..4):H_r:
```

```
r > mu:=add(u|i*H_r[i],i=1..4):
```

```
Cspace > C:=(i,j,k)->Hook(evalDG(Hook(R6Hook(mu,j),e|k)),theta|i):
```

```
Cspace > uMat:=DGinfo(DirectSumOfRepresentations([ad_l1,m_l1],R9),"RepresentationMatrices");
```

```
Cspace > for i to 3 do for j to 6 do for k to 3 do try uMat[k][i,j+3]:=C(i,j,k) catch: end try end do end do end do;
```

```
Cspace > uMat;
```

(46)

$$\begin{bmatrix}
\begin{bmatrix}
0 & 0 & 0 & 0 & 0 & 0 & 0 & 0 & 0 \\
0 & -1 & 0 & 0 & 0 & 0 & 0 & 0 & 0 \\
0 & 0 & -2 & 0 & 0 & 0 & 0 & 0 & 0 \\
0 & 0 & 0 & 1 & 0 & 0 & 0 & 0 & 0 \\
0 & 0 & 0 & 0 & 1 & 0 & 0 & 0 & 0 \\
0 & 0 & 0 & 0 & 0 & -1 & 0 & 0 & 0 \\
0 & 0 & 0 & 0 & 0 & 0 & -1 & 0 & 0 \\
0 & 0 & 0 & 0 & 0 & 0 & 0 & 0 & 0 \\
0 & 0 & 0 & 0 & 0 & 0 & 0 & 0 & 0
\end{bmatrix}, \\
\begin{bmatrix}
0 & 0 & 0 & -\frac{6}{5}u_2 + \frac{12}{5}u_4 & \frac{6}{5}u_1 - \frac{12}{5}u_3 & 0 & 0 & 0 & 0 \\
1 & 0 & 0 & 0 & 0 & 0 & 0 & 6u_2 & -6u_1 \\
0 & 0 & 0 & 0 & 0 & u_3 & u_4 & 0 & 0 \\
0 & 0 & 0 & 0 & 0 & 0 & 0 & 0 & 0 \\
0 & 0 & 0 & 0 & 0 & 0 & 0 & 0 & 0 \\
0 & 0 & 0 & 0 & 0 & 0 & 0 & 1 & 0 \\
0 & 0 & 0 & 0 & 0 & 0 & 0 & 0 & 1 \\
0 & 0 & 0 & -1 & 0 & 0 & 0 & 0 & 0 \\
0 & 0 & 0 & 0 & -1 & 0 & 0 & 0 & 0
\end{bmatrix}, \\
\begin{bmatrix}
0 & 0 & 0 & 0 & 0 & 0 & 0 & 0 & 0 \\
0 & 0 & 0 & u_1 & u_2 & 0 & 0 & 0 & 0 \\
2 & 0 & 0 & 0 & 0 & 0 & 0 & -\frac{12}{5}u_2 - \frac{6}{5}u_4 & \frac{12}{5}u_1 + \frac{6}{5}u_3 \\
0 & 0 & 0 & 0 & 0 & 0 & 0 & 0 & 0 \\
0 & 0 & 0 & 0 & 0 & 0 & 0 & 0 & 0 \\
0 & 0 & 0 & 0 & -6 & 0 & 0 & 0 & 0 \\
0 & 0 & 0 & 6 & 0 & 0 & 0 & 0 & 0 \\
0 & 0 & 0 & 0 & 0 & 0 & 0 & 0 & 0 \\
0 & 0 & 0 & 0 & 0 & 0 & 0 & 0 & 0
\end{bmatrix}
\end{bmatrix}$$

These matrices represent the most general 11-module  $g$  with  $g/11=m$  and  $g$  indecomposable, up to change of basis. The parameters  $u_i$  give the cohomology class, with  $u_i=0$  corresponding to the decomposable case (the matrices are visibly block diagonal in this case). We export the matrices to another file to look for Lie algebra structures on the module  $g$ .

```
> L2:=MinimalSubalgebra([P[1],P[2],P[5]]);
```

$$L2 := \left[ \begin{bmatrix} I & 0 & 0 \\ 0 & I & 0 \\ 0 & 0 & -2I \end{bmatrix}, \begin{bmatrix} 1 & 0 & 0 \\ 0 & -1 & 0 \\ 0 & 0 & 0 \end{bmatrix}, \begin{bmatrix} 0 & 0 & 0 \\ 6I & 0 & 0 \\ 0 & 0 & 0 \end{bmatrix} \right] \quad (47)$$

Part 3.3: The intersection of  $\mathfrak{h}$  and the Cartan subalgebra is 2D.

```
> l2Data:=LieAlgebraData(L2,l2):DGsetup(l2Data);
```

*Lie algebra: l2*

(48)

```
> L2_real:=map(realify,L2):m_l2:=Representation(l2,R6,L2_real)
:dm_l2:=TensorProductOfRepresentations(m_l2,DGinfo(R6,
"FrameBaseForms"),R6);
```

$$dm_{l2} := \left[ \begin{matrix} e1, \begin{bmatrix} 0 & -1 & 0 & 0 & 0 & 0 \\ 1 & 0 & 0 & 0 & 0 & 0 \\ 0 & 0 & 0 & -1 & 0 & 0 \\ 0 & 0 & 1 & 0 & 0 & 0 \\ 0 & 0 & 0 & 0 & 0 & 2 \\ 0 & 0 & 0 & 0 & -2 & 0 \end{bmatrix} \\ e2, \begin{bmatrix} -1 & 0 & 0 & 0 & 0 & 0 \\ 0 & -1 & 0 & 0 & 0 & 0 \\ 0 & 0 & 1 & 0 & 0 & 0 \\ 0 & 0 & 0 & 1 & 0 & 0 \\ 0 & 0 & 0 & 0 & 0 & 0 \\ 0 & 0 & 0 & 0 & 0 & 0 \end{bmatrix} \\ e3, \begin{bmatrix} 0 & 0 & 0 & -6 & 0 & 0 \\ 0 & 0 & 6 & 0 & 0 & 0 \\ 0 & 0 & 0 & 0 & 0 & 0 \\ 0 & 0 & 0 & 0 & 0 & 0 \\ 0 & 0 & 0 & 0 & 0 & 0 \\ 0 & 0 & 0 & 0 & 0 & 0 \end{bmatrix} \end{matrix} \right], \quad (49)$$

```
> ad_l2:=Adjoint(l2,representationspace=l2);
```

$$ad_{l2} := \left[ \begin{matrix} e1, \begin{bmatrix} 0 & 0 & 0 \\ 0 & 0 & 0 \\ 0 & 0 & 0 \end{bmatrix} \\ e2, \begin{bmatrix} 0 & 0 & 0 \\ 0 & 0 & 0 \\ 0 & 0 & -2 \end{bmatrix} \\ e3, \begin{bmatrix} 0 & 0 & 0 \\ 0 & 0 & 0 \\ 0 & 2 & 0 \end{bmatrix} \end{matrix} \right] \quad (50)$$

```
> dmtad_l2:=TensorProductOfRepresentations([dm_l2,ad_l2],R18):
```

This coefficient space is the tensor product of the realification of the restriction of the tautological representation and the adjoint representation of  $\mathfrak{l}_0$ .

```
> DGsetup(l2,dmtad_l2,Cspace);
```

*Lie algebra with coefficients: Cspace*

(51)

```
> Chains:=RelativeChains([ ]):Cohomology(Chains[1..3]);
```

$[[ ]]$

(52)

The cohomology is trivial in this case.
