# Supplementary material for: Almost complex structures in 6D with nondegenerate Nijenhuis tensors and large symmetry groups
Source: arXiv:1512.07161 ancillary file (2015-12-22)
Supplement: Supplementary file 2 [file All_solvable_isotropy_Jacobi.pdf]

## Section 1: indecomposable h-modules g

In this section we show that the Jacobi identity for g cannot be satisfied unless g decomposes as a direct sum as an h-module.

### Part 1.1: 4D isotropy algebra R

```
> restart:with(DifferentialGeometry): with(Tensor): with(Tools):  
with(LieAlgebras):
```

```
h > dimM:=6;
```

*dimM:=6*

(1)

These matrices give the most general non-decomposable representation of R with the required properties, up to change of basis. The parameters  $u_i$  determine the cohomology class. The representation matrices were imported from a separate worksheet.

```
v > MrepMat := [Matrix(10, 10, {(1, 1) = 0, (1, 2) = 0, (1, 3) =  
0, (1, 4) = 0, (1, 5) = 0, (1, 6) = 0, (1, 7) = 0, (1, 8) =  
0, (1, 9) = 0, (1, 10) = 0, (2, 1) = 0, (2, 2) = -1, (2, 3) =  
0, (2, 4) = 0, (2, 5) = 0, (2, 6) = 0, (2, 7) = 0, (2, 8) =  
0, (2, 9) = 0, (2, 10) = 0, (3, 1) = 0, (3, 2) = 0, (3, 3) =  
-1, (3, 4) = 0, (3, 5) = 0, (3, 6) = 0, (3, 7) = 0, (3, 8) =  
0, (3, 9) = 0, (3, 10) = 0, (4, 1) = 0, (4, 2) = 0, (4, 3) =  
0, (4, 4) = -2, (4, 5) = 0, (4, 6) = 0, (4, 7) = 0, (4, 8) =  
0, (4, 9) = 0, (4, 10) = 0, (5, 1) = 0, (5, 2) = 0, (5, 3) =  
0, (5, 4) = 0, (5, 5) = 1, (5, 6) = 0, (5, 7) = 0, (5, 8) =  
0, (5, 9) = 0, (5, 10) = 0, (6, 1) = 0, (6, 2) = 0, (6, 3) =  
0, (6, 4) = 0, (6, 5) = 0, (6, 6) = 1, (6, 7) = 0, (6, 8) =  
0, (6, 9) = 0, (6, 10) = 0, (7, 1) = 0, (7, 2) = 0, (7, 3) =  
0, (7, 4) = 0, (7, 5) = 0, (7, 6) = 0, (7, 7) = -1, (7, 8) =  
0, (7, 9) = 0, (7, 10) = 0, (8, 1) = 0, (8, 2) = 0, (8, 3) =  
0, (8, 4) = 0, (8, 5) = 0, (8, 6) = 0, (8, 7) = 0, (8, 8) =  
-1, (8, 9) = 0, (8, 10) = 0, (9, 1) = 0, (9, 2) = 0, (9, 3) =  
0, (9, 4) = 0, (9, 5) = 0, (9, 6) = 0, (9, 7) = 0, (9, 8) =  
0, (9, 9) = 0, (9, 10) = 0, (10, 1) = 0, (10, 2) = 0, (10, 3) =  
0, (10, 4) = 0, (10, 5) = 0, (10, 6) = 0, (10, 7) = 0, (10, 8) =  
0, (10, 9) = 0, (10, 10) = 0}), Matrix(10, 10, {(1, 1) =  
0, (1, 2) = 0, (1, 3) = 0, (1, 4) = 0, (1, 5) = (60/803)*u1+  
(4/2409)*u2+(8627/2409)*u5, (1, 6) = -(18/13)*u3+(823/104)*u4-  
5*u6, (1, 7) = 0, (1, 8) = 0, (1, 9) = 0, (1, 10) = 0, (2,  
1) = 1, (2, 2) = 0, (2, 3) = 0, (2, 4) = 0, (2, 5) = 0, (2,  
6) = 0, (2, 7) = 0, (2, 8) = 0, (2, 9) = (597/1606)*u1+  
(1967/4818)*u2-(2671/2409)*u5, (2, 10) = (7/39)*u3-(2005/312)*  
u4+6*u6, (3, 1) = 0, (3, 2) = 0, (3, 3) = 0, (3, 4) = 0, (3,  
5) = 0, (3, 6) = 0, (3, 7) = 0, (3, 8) = 0, (3, 9) =  
(109/117)*u3-(2461/936)*u4+(5/3)*u6, (3, 10) = u2, (4, 1) =  
0, (4, 2) = 0, (4, 3) = 1, (4, 4) = 0, (4, 5) = 0, (4, 6) =  
0, (4, 7) = (46/117)*u3-(2317/936)*u4+(5/3)*u6, (4, 8) = u5,  
(4, 9) = 0, (4, 10) = 0, (5, 1) = 0, (5, 2) = 0, (5, 3) = 0,  
(5, 4) = 0, (5, 5) = 0, (5, 6) = 0, (5, 7) = 0, (5, 8) = 0,  
(5, 9) = 0, (5, 10) = 0, (6, 1) = 0, (6, 2) = 0, (6, 3) = 0,  
(6, 4) = 0, (6, 5) = 0, (6, 6) = 0, (6, 7) = 0, (6, 8) = 0,  
(6, 9) = 0, (6, 10) = 0, (7, 1) = 0, (7, 2) = 0, (7, 3) = 0,
```

```

(7, 4) = 0, (7, 5) = 0, (7, 6) = 0, (7, 7) = 0, (7, 8) = 0,
(7, 9) = 1, (7, 10) = 0, (8, 1) = 0, (8, 2) = 0, (8, 3) = 0,
(8, 4) = 0, (8, 5) = 0, (8, 6) = 0, (8, 7) = 0, (8, 8) = 0,
(8, 9) = 0, (8, 10) = 1, (9, 1) = 0, (9, 2) = 0, (9, 3) = 0,
(9, 4) = 0, (9, 5) = -1, (9, 6) = 0, (9, 7) = 0, (9, 8) = 0,
(9, 9) = 0, (9, 10) = 0, (10, 1) = 0, (10, 2) = 0, (10, 3) =
0, (10, 4) = 0, (10, 5) = 0, (10, 6) = -1, (10, 7) = 0, (10,
8) = 0, (10, 9) = 0, (10, 10) = 0}}, Matrix(10, 10, {(1, 1) =
0, (1, 2) = 0, (1, 3) = 0, (1, 4) = 0, (1, 5) = -(8/117)*u3+
(136/117)*u4+(1/3)*u6, (1, 6) = -(1357/4818)*u1+(5573/4818)*
u2-(7597/2409)*u5, (1, 7) = 0, (1, 8) = 0, (1, 9) = 0, (1,
10) = 0, (2, 1) = 0, (2, 2) = 0, (2, 3) = 0, (2, 4) = 0, (2,
5) = 0, (2, 6) = 0, (2, 7) = 0, (2, 8) = 0, (2, 9) = -(1/3)*
u3+(307/24)*u4-13*u6, (2, 10) = u1, (3, 1) = 1, (3, 2) = 0,
(3, 3) = 0, (3, 4) = 0, (3, 5) = 0, (3, 6) = 0, (3, 7) = 0,
(3, 8) = 0, (3, 9) = (40/803)*u1-(5083/2409)*u2+(6019/2409)*
u5, (3, 10) = u3, (4, 1) = 0, (4, 2) = -1, (4, 3) = 0, (4, 4)
= 0, (4, 5) = 0, (4, 6) = 0, (4, 7) = (397/1606)*u1-
(3935/4818)*u2+(5167/2409)*u5, (4, 8) = u6, (4, 9) = 0, (4,
10) = 0, (5, 1) = 0, (5, 2) = 0, (5, 3) = 0, (5, 4) = 0, (5,
5) = 0, (5, 6) = 0, (5, 7) = 0, (5, 8) = 0, (5, 9) = 0, (5,
10) = 0, (6, 1) = 0, (6, 2) = 0, (6, 3) = 0, (6, 4) = 0, (6,
5) = 0, (6, 6) = 0, (6, 7) = 0, (6, 8) = 0, (6, 9) = 0, (6,
10) = 0, (7, 1) = 0, (7, 2) = 0, (7, 3) = 0, (7, 4) = 0, (7,
5) = 0, (7, 6) = 0, (7, 7) = 0, (7, 8) = 0, (7, 9) = 0, (7,
10) = -3, (8, 1) = 0, (8, 2) = 0, (8, 3) = 0, (8, 4) = 0, (8,
5) = 0, (8, 6) = 0, (8, 7) = 0, (8, 8) = 0, (8, 9) = 3, (8,
10) = 0, (9, 1) = 0, (9, 2) = 0, (9, 3) = 0, (9, 4) = 0, (9,
5) = 0, (9, 6) = -3, (9, 7) = 0, (9, 8) = 0, (9, 9) = 0, (9,
10) = 0, (10, 1) = 0, (10, 2) = 0, (10, 3) = 0, (10, 4) = 0,
(10, 5) = 3, (10, 6) = 0, (10, 7) = 0, (10, 8) = 0, (10, 9) =
0, (10, 10) = 0}}, Matrix(10, 10, {(1, 1) = 0, (1, 2) = 0,
(1, 3) = 0, (1, 4) = 0, (1, 5) = 0, (1, 6) = 0, (1, 7) = 0,
(1, 8) = 0, (1, 9) = 0, (1, 10) = 0, (2, 1) = 0, (2, 2) = 0,
(2, 3) = 0, (2, 4) = 0, (2, 5) = (16/117)*u3-(623/117)*u4+
(16/3)*u6, (2, 6) = -(956/2409)*u1-(164/2409)*u2+(416/2409)*
u5, (2, 7) = 0, (2, 8) = 0, (2, 9) = 0, (2, 10) = 0, (3, 1) =
0, (3, 2) = 0, (3, 3) = 0, (3, 4) = 0, (3, 5) = -(20/803)*u1+
(2140/2409)*u2-(2608/2409)*u5, (3, 6) = -(16/39)*u3-(1/39)*
u4, (3, 7) = 0, (3, 8) = 0, (3, 9) = 0, (3, 10) = 0, (4, 1) =
2, (4, 2) = 0, (4, 3) = 0, (4, 4) = 0, (4, 5) = 0, (4, 6) =
0, (4, 7) = 0, (4, 8) = 0, (4, 9) = (140/803)*u1-(2132/2409)*
u2+(5408/2409)*u5, (4, 10) = u4, (5, 1) = 0, (5, 2) = 0, (5,
3) = 0, (5, 4) = 0, (5, 5) = 0, (5, 6) = 0, (5, 7) = 0, (5,
8) = 0, (5, 9) = 0, (5, 10) = 0, (6, 1) = 0, (6, 2) = 0, (6,
3) = 0, (6, 4) = 0, (6, 5) = 0, (6, 6) = 0, (6, 7) = 0, (6,
8) = 0, (6, 9) = 0, (6, 10) = 0, (7, 1) = 0, (7, 2) = 0, (7,
3) = 0, (7, 4) = 0, (7, 5) = 0, (7, 6) = -6, (7, 7) = 0, (7,
8) = 0, (7, 9) = 0, (7, 10) = 0, (8, 1) = 0, (8, 2) = 0, (8,
3) = 0, (8, 4) = 0, (8, 5) = 6, (8, 6) = 0, (8, 7) = 0, (8,
8) = 0, (8, 9) = 0, (8, 10) = 0, (9, 1) = 0, (9, 2) = 0, (9,
3) = 0, (9, 4) = 0, (9, 5) = 0, (9, 6) = 0, (9, 7) = 0, (9,
8) = 0, (9, 9) = 0, (9, 10) = 0, (10, 1) = 0, (10, 2) = 0,
(10, 3) = 0, (10, 4) = 0, (10, 5) = 0, (10, 6) = 0, (10, 7) =
0, (10, 8) = 0, (10, 9) = 0, (10, 10) = 0}}]):

```

```

V80 > HData:=LieAlgebraData(MrepMat,h):DGsetup(HData);

```

```

Lie algebra: h (2)

```

```

V > DGsetup([seq(v||i,i=1..dimM)],m);
frame name: m (3)

```

```

m > DGsetup([seq(w||i,i=1..10)],g);
frame name: g (4)

```

```

g > rep:=Representation(h,g,MrepMat);
V > Mrep:=TensorProductOfRepresentations(grep,[seq(dw||i,i=5..10)
],m);

```

$Mrep := e1 \rightarrow \begin{bmatrix} -1 & 0 & 0 & 0 & 0 & 0 \\ 0 & -1 & 0 & 0 & 0 & 0 \\ 0 & 0 & 1 & 0 & 0 & 0 \\ 0 & 0 & 0 & 1 & 0 & 0 \\ 0 & 0 & 0 & 0 & 0 & 0 \\ 0 & 0 & 0 & 0 & 0 & 0 \end{bmatrix}, e2 \rightarrow \begin{bmatrix} 0 & 0 & 0 & 0 & 1 & 0 \\ 0 & 0 & 0 & 0 & 0 & 1 \\ 0 & 0 & 0 & 0 & 0 & 0 \\ 0 & 0 & 0 & 0 & 0 & 0 \\ 0 & 0 & -1 & 0 & 0 & 0 \\ 0 & 0 & 0 & -1 & 0 & 0 \end{bmatrix}, e3 \rightarrow$

$\begin{bmatrix} 0 & 0 & 0 & 0 & 0 & -3 \\ 0 & 0 & 0 & 0 & 3 & 0 \\ 0 & 0 & 0 & 0 & 0 & 0 \\ 0 & 0 & 0 & 0 & 0 & 0 \\ 0 & 0 & 0 & -3 & 0 & 0 \\ 0 & 0 & 3 & 0 & 0 & 0 \end{bmatrix}, e4 \rightarrow \begin{bmatrix} 0 & 0 & 0 & -6 & 0 & 0 \\ 0 & 0 & 6 & 0 & 0 & 0 \\ 0 & 0 & 0 & 0 & 0 & 0 \\ 0 & 0 & 0 & 0 & 0 & 0 \\ 0 & 0 & 0 & 0 & 0 & 0 \\ 0 & 0 & 0 & 0 & 0 & 0 \end{bmatrix}$

```

G > ChangeFrame(g);
g (6)

```

```

V80 > L2m:=GenerateForms([seq(dw||i,i=5..10)],2):L2mtg:=
GenerateTensors([L2m,[seq(D_w||i,i=1..10)]]):

```

We have defined the space  $\Lambda^2 m^* \otimes g$ . The next step is to find the subspace which satisfies all linear equations coming from  $g.x=0$ . This will reduce the number of parameters significantly. We repeatedly apply the Lie algebra basis to a generic element and solve only the linear equations until no further linear equations are generated.

```

g > G:=DGinfo(rep, "ObjectAttributes")[2,1,1]:conbasG:=DGinfo(G,
"FrameBaseVectors"):nG:=DGinfo(G, "LieAlgebraDimension")
:bracket_elements[0]:=evalDG(add(a[i]*L2mtg[i],i=1..nops
(L2mtg))):

```

```

g > image_elements[1]:=ApplyRepresentation(rep,conbasG[1],
bracket_elements[1-1]):
g > image_coefficients[1]:=DGinfo(image_elements[1],
"CoefficientSet"):
g > kernel_equations[1]:=solve(image_coefficients[1]):nops(%);

```

110

```

g > bracket_elements[1]:=DGsimplify(subs(kernel_equations[1],
bracket_elements[1-1])):

```

(7)

```

g > image_elements[2]:=ApplyRepresentation(rep,conbasG[2],
bracket_elements[2-1]):
g > image_coefficients[2]:=DGinfo(image_elements[2],
"CoefficientSet")[1..40];
image_coefficients2 := { -a35 - a19, a35 + a19, -a36 - a20, a36 + a20, -a45 + a75, -a46 + a76,
-a75 + a45, -a76 + a46, -a85 - a69, a85 + a69, -a86 - a70, a86 + a70, -a107 + a19, a107
-a19, -a108 + a20, a108 - a20, -a117 + a59, a117 - a59, -a118 + a60, a118 - a60, -a127
+ a29, a127 - a29, -a128 + a30, a128 - a30, -a137 + a69, a137 - a69, -a138 + a70, a138 - a70,
-a149 + a45 + a29, -a149 - a75 - a59, -a149 + a117 - a127, a149 - a45 - a29, a149 + a75
+ a59, a149 + a127 - a117, -a150 + a46 + a30, -a150 - a76 - a60, -a150 + a118 - a128, a150
-a46 - a30, a150 + a76 + a60, a150 + a128 - a118 }
g > kernel_equations[2]:=solve(image_coefficients[2]):nops(%);
26
g > bracket_elements[2]:=DGsimplify(subs(kernel_equations[2],
bracket_elements[2-1]]):

```

```

g > image_elements[3]:=ApplyRepresentation(rep,conbasG[3],
bracket_elements[3-1]):
g > image_coefficients[3]:=DGinfo(image_elements[3],
"CoefficientSet")[1..16];
image_coefficients3 := { -3 a19 - 3 a128, 3 a19 + 3 a69, 3 a20 + 3 a70, 3 a20 - 3 a127, -3 a69
- 3 a19, 3 a69 - 3 a128, -3 a70 - 3 a20, 3 a70 + 3 a127, -3 a102 - 3 a132, -3 a127 - 3 a70,
3 a127 - 3 a20, 3 a128 + 3 a19, 3 a128 - 3 a69, 3 a132 + 3 a102, -a141 + 3 a133 + 3 a103, a141
- 3 a103 - 3 a133 }
g > kernel_equations[3]:=solve(image_coefficients[3]):
g > bracket_elements[3]:=DGsimplify(subs(kernel_equations[3],
bracket_elements[3-1]]):

```

```

g > image_elements[4]:=ApplyRepresentation(rep,conbasG[4],
bracket_elements[4-1]):
g > image_coefficients[4]:=DGinfo(image_elements[4],
"CoefficientSet")[1..4]:
g > kernel_equations[4]:=solve(image_coefficients[4]):
g > bracket_elements[4]:=DGsimplify(subs(kernel_equations[4],
bracket_elements[4-1]]):

```

```

g > image_elements[5]:=ApplyRepresentation(rep,conbasG[2],
bracket_elements[5-1]):
g > image_coefficients[5]:=DGinfo(image_elements[5],
"CoefficientSet")[1..4]:
g > kernel_equations[5]:=solve(image_coefficients[5]):
g > bracket_elements[5]:=DGsimplify(subs(kernel_equations[5],
bracket_elements[5-1]]):

```

```

g > image_elements[6]:=ApplyRepresentation(rep,conbasG[4],

```

**bracket\_elements[6-1]):**  
**g > image\_coefficients[6]:=DGinfo(image\_elements[6],**  
**"CoefficientSet");**

$$\begin{aligned}
 \text{image\_coefficients}_6 := & \left\{ -u4 a_{128} - \frac{140}{803} a_{127} u1 + \frac{2132}{2409} a_{127} u2 - \frac{5408}{2409} a_{127} u5 - 2 a_{21}, \right. \\
 & -u4 a_{128} - \frac{140}{803} a_{127} u1 + \frac{2132}{2409} a_{127} u2 - \frac{5408}{2409} a_{127} u5 - 2 a_{51}, u4 a_{128} + \frac{140}{803} a_{127} u1 \\
 & - \frac{2132}{2409} a_{127} u2 + \frac{5408}{2409} a_{127} u5 + 2 a_{21}, u4 a_{128} + \frac{140}{803} a_{127} u1 - \frac{2132}{2409} a_{127} u2 \\
 & + \frac{5408}{2409} a_{127} u5 + 2 a_{51}, -6 a_{123} + \frac{16}{39} a_{127} u3 + \frac{1}{39} a_{127} u4 - \frac{20}{803} u1 a_{128} \\
 & + \frac{2140}{2409} a_{128} u2 - \frac{2608}{2409} u5 a_{128}, 6 a_{123} - \frac{16}{39} a_{127} u3 - \frac{1}{39} a_{127} u4 + \frac{20}{803} u1 a_{128} \\
 & - \frac{2140}{2409} a_{128} u2 + \frac{2608}{2409} u5 a_{128}, -6 a_{133} + \frac{16}{39} u3 a_{128} + \frac{1}{39} u4 a_{128} + \frac{20}{803} a_{127} u1 \\
 & - \frac{2140}{2409} a_{127} u2 + \frac{2608}{2409} a_{127} u5, 6 a_{133} - \frac{16}{39} u3 a_{128} - \frac{1}{39} u4 a_{128} - \frac{20}{803} a_{127} u1 \\
 & + \frac{2140}{2409} a_{127} u2 - \frac{2608}{2409} a_{127} u5, -a_{127} u4 - 6 a_{94} + \frac{140}{803} u1 a_{128} - \frac{2132}{2409} a_{128} u2 \\
 & + \frac{5408}{2409} u5 a_{128} + 2 a_{61}, -a_{127} u4 + 6 a_{94} + \frac{140}{803} u1 a_{128} - \frac{2132}{2409} a_{128} u2 \\
 & + \frac{5408}{2409} u5 a_{128} + 2 a_{61}, a_{127} u4 - 6 a_{94} - \frac{140}{803} u1 a_{128} + \frac{2132}{2409} a_{128} u2 \\
 & - \frac{5408}{2409} u5 a_{128} - 2 a_{61}, a_{127} u4 + 6 a_{94} - \frac{140}{803} u1 a_{128} + \frac{2132}{2409} a_{128} u2 \\
 & - \frac{5408}{2409} u5 a_{128} - 2 a_{61}, -6 a_{122} + \frac{956}{2409} a_{127} u1 + \frac{164}{2409} a_{127} u2 - \frac{416}{2409} a_{127} u5 \\
 & + \frac{16}{117} u3 a_{128} - \frac{623}{117} u4 a_{128} + \frac{16}{3} u6 a_{128}, 6 a_{122} - \frac{956}{2409} a_{127} u1 - \frac{164}{2409} a_{127} u2 \\
 & + \frac{416}{2409} a_{127} u5 - \frac{16}{117} u3 a_{128} + \frac{623}{117} u4 a_{128} - \frac{16}{3} u6 a_{128}, -6 a_{132} + \frac{956}{2409} u1 a_{128} \\
 & + \frac{164}{2409} a_{128} u2 - \frac{416}{2409} u5 a_{128} - \frac{16}{117} a_{127} u3 + \frac{623}{117} a_{127} u4 - \frac{16}{3} a_{127} u6, 6 a_{132} \\
 & - \frac{956}{2409} u1 a_{128} - \frac{164}{2409} a_{128} u2 + \frac{416}{2409} u5 a_{128} + \frac{16}{117} a_{127} u3 - \frac{623}{117} a_{127} u4 \\
 & \left. + \frac{16}{3} a_{127} u6 \right\}
 \end{aligned}
 \tag{11}$$

**g > bracket:=bracket\_elements[6-1]:**  
**g > DGinfo(nonlinear\_element,"CoefficientSet");nops(%);**  
 $\{a_{21}, a_{51}, a_{61}, a_{94}, a_{122}, a_{123}, a_{127}, a_{128}, a_{132}, a_{133}, -a_{21}, -a_{51}, -a_{61}, -a_{94}, -a_{122}, -a_{123}, -a_{127},$   
 $-a_{128}, -a_{132}, -a_{133}\}$

The number of parameters  $a_i$  has been reduced from 150 to 10.

**g > bracket;**

$$\begin{aligned}
 & -a_{61} dw5 \otimes dw7 \otimes \partial_{w1} - a_{128} dw5 \otimes dw7 \otimes \partial_{w9} + a_{127} dw5 \otimes dw7 \otimes \partial_{w10} + a_{21} dw5 \otimes dw8 \\
 & \otimes \partial_{w1} + a_{127} dw5 \otimes dw8 \otimes \partial_{w9} + a_{128} dw5 \otimes dw8 \otimes \partial_{w10} + a_{128} dw5 \otimes dw9 \otimes \partial_{w5} \\
 & - a_{127} dw5 \otimes dw9 \otimes \partial_{w6} - a_{127} dw5 \otimes dw10 \otimes \partial_{w5} - a_{128} dw5 \otimes dw10 \otimes \partial_{w6} + a_{51} dw6 \\
 & \otimes dw7 \otimes \partial_{w1} + a_{127} dw6 \otimes dw7 \otimes \partial_{w9} + a_{128} dw6 \otimes dw7 \otimes \partial_{w10} + a_{61} dw6 \otimes dw8 \otimes \partial_{w1} \\
 & + a_{128} dw6 \otimes dw8 \otimes \partial_{w9} - a_{127} dw6 \otimes dw8 \otimes \partial_{w10} - a_{127} dw6 \otimes dw9 \otimes \partial_{w5} - a_{128} dw6 \\
 & \otimes dw9 \otimes \partial_{w6} - a_{128} dw6 \otimes dw10 \otimes \partial_{w5} + a_{127} dw6 \otimes dw10 \otimes \partial_{w6} + a_{61} dw7 \otimes dw5 \otimes \partial_{w1} \\
 & + a_{128} dw7 \otimes dw5 \otimes \partial_{w9} - a_{127} dw7 \otimes dw5 \otimes \partial_{w10} - a_{51} dw7 \otimes dw6 \otimes \partial_{w1} - a_{127} dw7 \\
 & \otimes dw6 \otimes \partial_{w9} - a_{128} dw7 \otimes dw6 \otimes \partial_{w10} + a_{94} dw7 \otimes dw8 \otimes \partial_{w4} - a_{132} dw7 \otimes dw9 \otimes \partial_{w2} \\
 & - a_{133} dw7 \otimes dw9 \otimes \partial_{w3} - a_{128} dw7 \otimes dw9 \otimes \partial_{w7} + a_{127} dw7 \otimes dw9 \otimes \partial_{w8} + a_{122} dw7 \\
 & \otimes dw10 \otimes \partial_{w2} + a_{123} dw7 \otimes dw10 \otimes \partial_{w3} + a_{127} dw7 \otimes dw10 \otimes \partial_{w7} + a_{128} dw7 \otimes dw10 \\
 & \otimes \partial_{w8} - a_{21} dw8 \otimes dw5 \otimes \partial_{w1} - a_{127} dw8 \otimes dw5 \otimes \partial_{w9} - a_{128} dw8 \otimes dw5 \otimes \partial_{w10} - a_{61} dw8 \\
 & \otimes dw6 \otimes \partial_{w1} - a_{128} dw8 \otimes dw6 \otimes \partial_{w9} + a_{127} dw8 \otimes dw6 \otimes \partial_{w10} - a_{94} dw8 \otimes dw7 \\
 & \otimes \partial_{w4} + a_{122} dw8 \otimes dw9 \otimes \partial_{w2} + a_{123} dw8 \otimes dw9 \otimes \partial_{w3} + a_{127} dw8 \otimes dw9 \otimes \partial_{w7} + a_{128} dw8 \\
 & \otimes dw9 \otimes \partial_{w8} + a_{132} dw8 \otimes dw10 \otimes \partial_{w2} + a_{133} dw8 \otimes dw10 \otimes \partial_{w3} + a_{128} dw8 \otimes dw10 \\
 & \otimes \partial_{w7} - a_{127} dw8 \otimes dw10 \otimes \partial_{w8} - a_{128} dw9 \otimes dw5 \otimes \partial_{w5} + a_{127} dw9 \otimes dw5 \otimes \partial_{w6} \\
 & + a_{127} dw9 \otimes dw6 \otimes \partial_{w5} + a_{128} dw9 \otimes dw6 \otimes \partial_{w6} + a_{132} dw9 \otimes dw7 \otimes \partial_{w2} + a_{133} dw9 \\
 & \otimes dw7 \otimes \partial_{w3} + a_{128} dw9 \otimes dw7 \otimes \partial_{w7} - a_{127} dw9 \otimes dw7 \otimes \partial_{w8} - a_{122} dw9 \otimes dw8 \otimes \partial_{w2} \\
 & - a_{123} dw9 \otimes dw8 \otimes \partial_{w3} - a_{127} dw9 \otimes dw8 \otimes \partial_{w7} - a_{128} dw9 \otimes dw8 \otimes \partial_{w8} + a_{127} dw10 \\
 & \otimes dw5 \otimes \partial_{w5} + a_{128} dw10 \otimes dw5 \otimes \partial_{w6} + a_{128} dw10 \otimes dw6 \otimes \partial_{w5} - a_{127} dw10 \otimes dw6 \\
 & \otimes \partial_{w6} - a_{122} dw10 \otimes dw7 \otimes \partial_{w2} - a_{123} dw10 \otimes dw7 \otimes \partial_{w3} - a_{127} dw10 \otimes dw7 \otimes \partial_{w7} \\
 & - a_{128} dw10 \otimes dw7 \otimes \partial_{w8} - a_{132} dw10 \otimes dw8 \otimes \partial_{w2} - a_{133} dw10 \otimes dw8 \otimes \partial_{w3} - a_{128} dw10 \\
 & \otimes dw8 \otimes \partial_{w7} + a_{127} dw10 \otimes dw8 \otimes \partial_{w8}
 \end{aligned} \tag{13}$$

We initialize the bracket as an algebra and check the Jacobi identity to find more equations.

**V80 > HTensor:=[seq(convert(MrepMat[i],DGtensor,[["con\_bas",  
"cov\_bas"]],[i=1..nops(MrepMat)])];**

$$\begin{aligned}
 HTensor := & \left[ -\partial_{w2} \otimes dw2 - \partial_{w3} \otimes dw3 - 2 \partial_{w4} \otimes dw4 + \partial_{w5} \otimes dw5 + \partial_{w6} \otimes dw6 - \partial_{w7} \otimes dw7 - \partial_{w8} \otimes dw8, \right. \\
 & \left( \frac{60 u1}{803} + \frac{4 u2}{2409} + \frac{8627 u5}{2409} \right) \partial_{w1} \otimes dw5 - \left( \frac{18 u3}{13} - \frac{823 u4}{104} + 5 u6 \right) \\
 & \left. \partial_{w1} \otimes dw6 + \partial_{w2} \otimes dw1 + \left( \frac{597 u1}{1606} + \frac{1967 u2}{4818} - \frac{2671 u5}{2409} \right) \partial_{w2} \otimes dw9 + \left( \frac{7 u3}{39} \right. \right.
 \end{aligned} \tag{14}$$

$$\begin{aligned}
& -\frac{2005 u4}{312} + 6 u6 \Big) \partial_{w2} \otimes dw10 + \left( \frac{109 u3}{117} - \frac{2461 u4}{936} + \frac{5 u6}{3} \right) \partial_{w3} \otimes dw9 + u2 \partial_{w3} \\
& \otimes dw10 + \partial_{w4} \otimes dw3 + \left( \frac{46 u3}{117} - \frac{2317 u4}{936} + \frac{5 u6}{3} \right) \partial_{w4} \otimes dw7 + u5 \partial_{w4} \otimes dw8 + \partial_{w7} \\
& \otimes dw9 + \partial_{w8} \otimes dw10 - \partial_{w9} \otimes dw5 - \partial_{w10} \otimes dw6, - \left( \frac{8 u3}{117} - \frac{136 u4}{117} - \frac{u6}{3} \right) \partial_{w1} \otimes d \\
& w5 - \left( \frac{1357 u1}{4818} - \frac{5573 u2}{4818} + \frac{7597 u5}{2409} \right) \partial_{w1} \otimes dw6 - \left( \frac{u3}{3} - \frac{307 u4}{24} + 13 u6 \right) \partial_{w2} \otimes d \\
& w9 + u1 \partial_{w2} \otimes dw10 + \partial_{w3} \otimes dw1 + \left( \frac{40 u1}{803} - \frac{5083 u2}{2409} + \frac{6019 u5}{2409} \right) \partial_{w3} \otimes dw9 \\
& + u3 \partial_{w3} \otimes dw10 - \partial_{w4} \otimes dw2 + \left( \frac{397 u1}{1606} - \frac{3935 u2}{4818} + \frac{5167 u5}{2409} \right) \partial_{w4} \otimes dw7 + u6 \partial_{w4} \\
& \otimes dw8 - 3 \partial_{w7} \otimes dw10 + 3 \partial_{w8} \otimes dw9 - 3 \partial_{w9} \otimes dw6 + 3 \partial_{w10} \otimes dw5, \left( \frac{16 u3}{117} \right. \\
& - \frac{623 u4}{117} + \frac{16 u6}{3} \Big) \partial_{w2} \otimes dw5 - \left( \frac{956 u1}{2409} + \frac{164 u2}{2409} - \frac{416 u5}{2409} \right) \partial_{w2} \otimes dw6 - \\
& \left( \frac{20 u1}{803} - \frac{2140 u2}{2409} + \frac{2608 u5}{2409} \right) \partial_{w3} \otimes dw5 - \left( \frac{16 u3}{39} + \frac{u4}{39} \right) \partial_{w3} \otimes dw6 + 2 \partial_{w4} \otimes dw1 \\
& + \left( \frac{140 u1}{803} - \frac{2132 u2}{2409} + \frac{5408 u5}{2409} \right) \partial_{w4} \otimes dw9 + u4 \partial_{w4} \otimes dw10 - 6 \partial_{w7} \otimes dw6 + 6 \partial_{w8} \\
& \otimes dw5 \Big]
\end{aligned}$$

```

V > A:=(x,y,z)->GetComponents(evalDG(ContractIndices(HTensor[x],
HTensor[y],[[2,1]])&minus ContractIndices(HTensor[y],HTensor
[x],[[2,1]])),HTensor)[z]:

```

```

V > B:=(x,y,z)->GetComponents(convert(evalDG(ContractIndices
(HTensor[x],D_w|y,[[2,1]])),DGvector),DGinfo(g,
"FrameBaseVectors"))[z]:

```

```

g > C:=(x,y,z)->GetComponents(convert(ContractIndices( evalDG
(D_w||x &t D_w||y), bracket,[[1,1],[2,2]]),DGvector),DGinfo
(g,"FrameBaseVectors"))[z]:

```

```

V > CH:=[seq(seq([q||i,q||j]=add(A(i,j,k)*q||k,k=1..nops(MrepMat)
),i=j+1..nops(MrepMat)),j=1..nops(MrepMat))];

```

$$CH := [[q2, q1] = q2, [q3, q1] = q3, [q4, q1] = 2 q4, [q3, q2] = -q4, [q4, q2] = 0, [q4, q3] = 0] \quad (15)$$

```

L2 > ChangeFrame(g);

```

$g$

(16)

```

V > CHM:=[seq(seq([q||i,q||j]=add(B(i,j,k)*q||k,k=1..10),i=1..
nops(MrepMat)),j=5..10)];

```

$$\begin{aligned}
CHM := & \left[ [q1, q5] = q5, [q2, q5] = \left( \frac{60}{803} u1 + \frac{4}{2409} u2 + \frac{8627}{2409} u5 \right) q1 - q9, [q3, q5] = \left( \right. \right. \\
& - \frac{8}{117} u3 + \frac{136}{117} u4 + \frac{1}{3} u6 \Big) q1 + 3 q10, [q4, q5] = \left( \frac{16}{117} u3 - \frac{623}{117} u4 \right. \\
& \left. \left. + \frac{16}{3} u6 \right) q2 + \left( - \frac{20}{803} u1 + \frac{2140}{2409} u2 - \frac{2608}{2409} u5 \right) q3 + 6 q8, [q1, q6] = q6, [q2, q6] \right] \quad (17)
\end{aligned}$$

$$\begin{aligned}
&= \left( -\frac{18}{13} u_3 + \frac{823}{104} u_4 - 5 u_6 \right) q_1 - q_{10}, [q_3, q_6] = \left( -\frac{1357}{4818} u_1 + \frac{5573}{4818} u_2 \right. \\
&\quad \left. - \frac{7597}{2409} u_5 \right) q_1 - 3 q_9, [q_4, q_6] = \left( -\frac{956}{2409} u_1 - \frac{164}{2409} u_2 + \frac{416}{2409} u_5 \right) q_2 + \left( \right. \\
&\quad \left. - \frac{16}{39} u_3 - \frac{1}{39} u_4 \right) q_3 - 6 q_7, [q_1, q_7] = -q_7, [q_2, q_7] = \left( \frac{46}{117} u_3 - \frac{2317}{936} u_4 \right. \\
&\quad \left. + \frac{5}{3} u_6 \right) q_4, [q_3, q_7] = \left( \frac{397}{1606} u_1 - \frac{3935}{4818} u_2 + \frac{5167}{2409} u_5 \right) q_4, [q_4, q_7] = 0, [q_1, q_8] \\
&= -q_8, [q_2, q_8] = u_5 q_4, [q_3, q_8] = u_6 q_4, [q_4, q_8] = 0, [q_1, q_9] = 0, [q_2, q_9] \\
&= \left( \frac{597}{1606} u_1 + \frac{1967}{4818} u_2 - \frac{2671}{2409} u_5 \right) q_2 + \left( \frac{109}{117} u_3 - \frac{2461}{936} u_4 + \frac{5}{3} u_6 \right) q_3 + q_7, \\
&[q_3, q_9] = \left( -\frac{1}{3} u_3 + \frac{307}{24} u_4 - 13 u_6 \right) q_2 + \left( \frac{40}{803} u_1 - \frac{5083}{2409} u_2 + \frac{6019}{2409} u_5 \right) q_3 \\
&\quad + 3 q_8, [q_4, q_9] = \left( \frac{140}{803} u_1 - \frac{2132}{2409} u_2 + \frac{5408}{2409} u_5 \right) q_4, [q_1, q_{10}] = 0, [q_2, q_{10}] \\
&= \left( \frac{7}{39} u_3 - \frac{2005}{312} u_4 + 6 u_6 \right) q_2 + u_2 q_3 + q_8, [q_3, q_{10}] = q_2 u_1 + q_3 u_3 - 3 q_7, [q_4, \\
&\quad q_{10}] = u_4 q_4
\end{aligned}$$

**g > CM:= [seq(seq([q||i,q||j]=add(C(i,j,k)\*q||k,k=1..10),j=i+1..10),i=5..10)];**

$CM := [ [q_5, q_6] = 0, [q_5, q_7] = -q_1 a_{61} + q_{10} a_{127} - q_9 a_{128}, [q_5, q_8] = q_1 a_{21} + q_{10} a_{128} + q_9 a_{127}, [q_5, q_9] = q_5 a_{128} - q_6 a_{127}, [q_5, q_{10}] =$

**v > KData:=LieAlgebraData([op(CH),op(CHM),op(CM)], [seq(q||i,i=1..nops(MrepMat)+dimM)]);**

$KData := [e_1, e_2] = -e_2, [e_1, e_3] = -e_3, [e_1, e_4] = -2 e_4, [e_1, e_5] = e_5, [e_1, e_6] = e_6, [e_1, e_7] = -e_7, [e_1, e_8] = -e_8, [e_1, e_9] = 0, [e_1, e_{10}] = 0, [e_2, e_3] = e_4, [e_2, e_4] = 0, [e_2, e_5]$  (19)

$$\begin{aligned}
&= \left( \frac{60 u_1}{803} + \frac{4 u_2}{2409} + \frac{8627 u_5}{2409} \right) e_1 - e_9, [e_2, e_6] = -\left( \frac{18 u_3}{13} - \frac{823 u_4}{104} + 5 u_6 \right) e_1 \\
&\quad - e_{10}, [e_2, e_7] = \left( \frac{46 u_3}{117} - \frac{2317 u_4}{936} + \frac{5 u_6}{3} \right) e_4, [e_2, e_8] = u_5 e_4, [e_2, e_9] = \left( \frac{597 u_1}{1606} \right. \\
&\quad \left. + \frac{1967 u_2}{4818} - \frac{2671 u_5}{2409} \right) e_2 + \left( \frac{109 u_3}{117} - \frac{2461 u_4}{936} + \frac{5 u_6}{3} \right) e_3 + e_7, [e_2, e_{10}] = \\
&\quad \left( \frac{7 u_3}{39} - \frac{2005 u_4}{312} + 6 u_6 \right) e_2 + u_2 e_3 + e_8, [e_3, e_4] = 0, [e_3, e_5] = -\left( \frac{8 u_3}{117} - \frac{136 u_4}{117} \right. \\
&\quad \left. - \frac{u_6}{3} \right) e_1 + 3 e_{10}, [e_3, e_6] = -\left( \frac{1357 u_1}{4818} - \frac{5573 u_2}{4818} + \frac{7597 u_5}{2409} \right) e_1 - 3 e_9, [e_3, e_7] \\
&= \left( \frac{397 u_1}{1606} - \frac{3935 u_2}{4818} + \frac{5167 u_5}{2409} \right) e_4, [e_3, e_8] = u_6 e_4, [e_3, e_9] = -\left( \frac{u_3}{3} - \frac{307 u_4}{24} \right. \\
&\quad \left. + 13 u_6 \right) e_2 + \left( \frac{40 u_1}{803} - \frac{5083 u_2}{2409} + \frac{6019 u_5}{2409} \right) e_3 + 3 e_8, [e_3, e_{10}] = u_1 e_2 + u_3 e_3
\end{aligned}$$



$$\begin{aligned}
& -3 e7, [e4, e5] = \left( \frac{16 u3}{117} - \frac{623 u4}{117} + \frac{16 u6}{3} \right) e2 - \left( \frac{20 u1}{803} - \frac{2140 u2}{2409} + \frac{2608 u5}{2409} \right) e3 + 6 e8, [e4, e6] = - \left( \frac{956 u1}{2409} + \frac{164 u2}{2409} - \frac{416 u5}{2409} \right) e2 - \left( \frac{16 u3}{39} + \frac{u4}{39} \right) e3 \\
& -6 e7, [e4, e7] = 0, [e4, e8] = 0, [e4, e9] = \left( \frac{140 u1}{803} - \frac{2132 u2}{2409} + \frac{5408 u5}{2409} \right) e4, [e4, e10] = u4 e4, [e5, e6] = 0, [e5, e7] = -a_{61} e1 - a_{128} e9 + a_{127} e10, [e5, e8] = a_{21} e1 \\
& + a_{127} e9 + a_{128} e10, [e5, e9] = a_{128} e5 - a_{127} e6, [e5, e10] = -a_{127} e5 - a_{128} e6, [e6, e7] = a_{51} e1 + a_{127} e9 + a_{128} e10, [e6, e8] = a_{61} e1 + a_{128} e9 - a_{127} e10, [e6, e9] = -a_{127} e5 \\
& - a_{128} e6, [e6, e10] = -a_{128} e5 + a_{127} e6, [e7, e8] = a_{94} e4, [e7, e9] = -a_{132} e2 - a_{133} e3 - a_{128} e7 + a_{127} e8, [e7, e10] = a_{122} e2 + a_{123} e3 + a_{127} e7 + a_{128} e8, [e8, e9] = a_{122} e2 \\
& + a_{123} e3 + a_{127} e7 + a_{128} e8, [e8, e10] = a_{132} e2 + a_{133} e3 + a_{128} e7 - a_{127} e8, [e9, e10] = 0
\end{aligned}$$

These are the most general possible structure constants of g.

```
h > DGsetup(KData);
```

*Lie algebra: L1*

(20)

```
h > Jaceq:=Query({seq(a||i,i=1..150),seq(u||i,i=1..6)},"Jacobi");
```

```
L1 > Jaceq[2];
```

$$\left\{ u1, a_{21}, a_{51}, a_{132}, -3u2, 3u2, -3u3, 3u3, 6u5, 6u6, -a_{21}, -a_{51}, -a_{122}, -3a_{123}, 3a_{123}, -a_{132}, -3a_{133}, 3a_{133}, -\frac{16}{13}u3 - \frac{1}{13}u4, \frac{79}{13}u4 + \dots \right\}$$

The Jacobi identity yields linear equations in the cohomology parameters  $u_i$  (in the output above,  $u1=0, 3u2=0, \dots$ ). We immediately get that they must vanish, and hence the module g is actually decomposable with respect to h.

```
L1 > solve(Jaceq[2]);
```

$$\left\{ u1=0, u2=0, u3=0, u4=0, u5=0, u6=0, a_{21}=0, a_{51}=0, a_{61}=0, a_{94}=0, a_{122}=0, a_{123}=0, \right. \\
\left. a_{127} = \text{RootOf}(\_Z^2 + 1), a_{128}, a_{128} = a_{128}, a_{132}=0, a_{133}=0 \right\} \quad (22)$$

```
v > jacoperator:=(x,y,z)->evalDG(LieBracket(LieBracket(x,y),z)+
LieBracket(LieBracket(z,x),y)+LieBracket(LieBracket(y,z),x));
```

```
L1 > jacoperator(e5,e9,e10);
```

$$- \left( 2 a_{127}^2 + 2 a_{128}^2 \right) e6 \quad (23)$$

This Jacobi identity says that  $a_{127}=a_{128}=0$ . The only real solution is the flat case.

**Part 1.2: 3D isotropy l\_2.**

```
> restart: with(DifferentialGeometry): with(Tensor): with(Tools):
with(LieAlgebras):
```

```
h > dimM:=6;
```

$\dim M := 6$

(24)

We import the representation matrices from the other worksheet. In this case, the cohomology is 10D.

```
V > MrepMat := [Matrix(9, 9, {(1, 1) = 0, (1, 2) = 0, (1, 3) = 0,
(1, 4) = (1/7)*u7-(19/7)*u8-(24/7)*u9, (1, 5) = (9/5)*u5-
(19/15)*u6-(21/5)*u10, (1, 6) = 0, (1, 7) = 0, (1, 8) = -
(55/39)*u2+(4243/1833)*u3, (1, 9) = u4, (2, 1) = 0, (2, 2) =
0, (2, 3) = 0, (2, 4) = u6, (2, 5) = (24/7)*u7-(15/7)*u8-
(9/7)*u9, (2, 6) = 0, (2, 7) = 0, (2, 8) = u1, (2, 9) = -
(55/117)*u2-(1/117)*u3, (3, 1) = 0, (3, 2) = 1, (3, 3) = 0,
(3, 4) = 0, (3, 5) = 0, (3, 6) = (389/6050)*u1+(423/6050)*u4,
(3, 7) = (8/117)*u2-(19/117)*u3, (3, 8) = -u6-3*u10, (3, 9) =
-(3/7)*u7+(15/7)*u8+(9/7)*u9, (4, 1) = 0, (4, 2) = 0, (4, 3)
= 0, (4, 4) = 0, (4, 5) = 0, (4, 6) = 0, (4, 7) = 0, (4, 8) =
0, (4, 9) = 0, (5, 1) = 0, (5, 2) = 0, (5, 3) = 0, (5, 4) =
0, (5, 5) = 0, (5, 6) = 0, (5, 7) = 0, (5, 8) = 0, (5, 9) =
0, (6, 1) = 0, (6, 2) = 0, (6, 3) = 0, (6, 4) = 0, (6, 5) =
0, (6, 6) = 0, (6, 7) = 0, (6, 8) = 1, (6, 9) = 0, (7, 1) =
0, (7, 2) = 0, (7, 3) = 0, (7, 4) = 0, (7, 5) = 0, (7, 6) =
0, (7, 7) = 0, (7, 8) = 0, (7, 9) = 1, (8, 1) = 0, (8, 2) =
0, (8, 3) = 0, (8, 4) = -1, (8, 5) = 0, (8, 6) = 0, (8, 7) =
0, (8, 8) = 0, (8, 9) = 0, (9, 1) = 0, (9, 2) = 0, (9, 3) =
0, (9, 4) = 0, (9, 5) = -1, (9, 6) = 0, (9, 7) = 0, (9, 8) =
0, (9, 9) = 0}), Matrix(9, 9, {(1, 1) = 0, (1, 2) = 0, (1, 3)
= 0, (1, 4) = u5, (1, 5) = u9, (1, 6) = 0, (1, 7) = 0, (1, 8)
= -(423/6050)*u1-(13011/6050)*u4, (1, 9) = -3*u2+(234/47)*u3,
(2, 1) = 0, (2, 2) = 0, (2, 3) = 0, (2, 4) = u7, (2, 5) =
u10, (2, 6) = 0, (2, 7) = 0, (2, 8) = u2, (2, 9) =
(12729/6050)*u1-(47/6050)*u4, (3, 1) = -1, (3, 2) = 0, (3, 3)
= 0, (3, 4) = 0, (3, 5) = 0, (3, 6) = -(8/39)*u2+(1517/1833)*
u3, (3, 7) = (3807/6050)*u1+(2149/6050)*u4, (3, 8) = (1/7)*u7
-(19/7)*u8-(3/7)*u9, (3, 9) = -(6/5)*u5-(19/15)*u6-(21/5)*
u10, (4, 1) = 0, (4, 2) = 0, (4, 3) = 0, (4, 4) = 0, (4, 5) =
0, (4, 6) = 0, (4, 7) = 0, (4, 8) = 0, (4, 9) = 0, (5, 1) =
0, (5, 2) = 0, (5, 3) = 0, (5, 4) = 0, (5, 5) = 0, (5, 6) =
0, (5, 7) = 0, (5, 8) = 0, (5, 9) = 0, (6, 1) = 0, (6, 2) =
0, (6, 3) = 0, (6, 4) = 0, (6, 5) = 0, (6, 6) = 0, (6, 7) =
0, (6, 8) = 0, (6, 9) = -3, (7, 1) = 0, (7, 2) = 0, (7, 3) =
0, (7, 4) = 0, (7, 5) = 0, (7, 6) = 0, (7, 7) = 0, (7, 8) =
3, (7, 9) = 0, (8, 1) = 0, (8, 2) = 0, (8, 3) = 0, (8, 4) =
0, (8, 5) = -3, (8, 6) = 0, (8, 7) = 0, (8, 8) = 0, (8, 9) =
0, (9, 1) = 0, (9, 2) = 0, (9, 3) = 0, (9, 4) = 3, (9, 5) =
0, (9, 6) = 0, (9, 7) = 0, (9, 8) = 0, (9, 9) = 0}), Matrix
(9, 9, {(1, 1) = 0, (1, 2) = 0, (1, 3) = 0, (1, 4) = -
(423/6050)*u1+(5139/6050)*u4, (1, 5) = (16/13)*u2-(1201/611)*
u3, (1, 6) = 0, (1, 7) = 0, (1, 8) = 0, (1, 9) = 0, (2, 1) =
0, (2, 2) = 0, (2, 3) = 0, (2, 4) = -(16/39)*u2-(1/39)*u3,
(2, 5) = -(5421/6050)*u1-(47/6050)*u4, (2, 6) = 0, (2, 7) =
0, (2, 8) = 0, (2, 9) = 0, (3, 1) = 0, (3, 2) = 0, (3, 3) =
0, (3, 4) = u8, (3, 5) = (3/5)*u5+(7/15)*u6+(8/5)*u10, (3, 6)
= 0, (3, 7) = 0, (3, 8) = u3, (3, 9) = (141/110)*u1+(47/110)*
```

$$\begin{aligned}
& u4, (4, 1) = 0, (4, 2) = 0, (4, 3) = 0, (4, 4) = 0, (4, 5) = \\
& 0, (4, 6) = 0, (4, 7) = 0, (4, 8) = 0, (4, 9) = 0, (5, 1) = \\
& 0, (5, 2) = 0, (5, 3) = 0, (5, 4) = 0, (5, 5) = 0, (5, 6) = \\
& 0, (5, 7) = 0, (5, 8) = 0, (5, 9) = 0, (6, 1) = 0, (6, 2) = \\
& 0, (6, 3) = 0, (6, 4) = 0, (6, 5) = -6, (6, 6) = 0, (6, 7) = \\
& 0, (6, 8) = 0, (6, 9) = 0, (7, 1) = 0, (7, 2) = 0, (7, 3) = \\
& 0, (7, 4) = 6, (7, 5) = 0, (7, 6) = 0, (7, 7) = 0, (7, 8) = \\
& 0, (7, 9) = 0, (8, 1) = 0, (8, 2) = 0, (8, 3) = 0, (8, 4) = \\
& 0, (8, 5) = 0, (8, 6) = 0, (8, 7) = 0, (8, 8) = 0, (8, 9) = \\
& 0, (9, 1) = 0, (9, 2) = 0, (9, 3) = 0, (9, 4) = 0, (9, 5) = \\
& 0, (9, 6) = 0, (9, 7) = 0, (9, 8) = 0, (9, 9) = 0\} )1;
\end{aligned}$$

$$\begin{aligned}
MrepMat := & \left[ \left[ \left[ 0, 0, 0, \frac{1}{7} u7 - \frac{19}{7} u8 - \frac{24}{7} u9, \frac{9}{5} u5 - \frac{19}{15} u6 - \frac{21}{5} u10, 0, 0, -\frac{55}{39} u2 \right. \right. \right. \\
& \left. \left. \left. + \frac{4243}{1833} u3, u4 \right] \right] \right] \quad (25)
\end{aligned}$$

$$\left[ 0, 0, 0, u6, \frac{24}{7} u7 - \frac{15}{7} u8 - \frac{9}{7} u9, 0, 0, u1, -\frac{55}{117} u2 - \frac{1}{117} u3 \right],$$

$$\begin{aligned}
& \left[ 0, 1, 0, 0, 0, \frac{389}{6050} u1 + \frac{423}{6050} u4, \frac{8}{117} u2 - \frac{19}{117} u3, -u6 - 3 u10, -\frac{3}{7} u7 + \frac{15}{7} u8 \right. \\
& \left. + \frac{9}{7} u9 \right],
\end{aligned}$$

---

$$\begin{bmatrix} 0, 0, 0, 0, 0, 0, 0, 0, 0 \end{bmatrix},$$

$$\begin{bmatrix} 0, 0, 0, 0, 0, 0, 0, 0, 0 \end{bmatrix},$$

$$\begin{bmatrix} 0, 0, 0, 0, 0, 0, 0, 1, 0 \end{bmatrix},$$

$$\left[0, 0, 0, 0, 0, 0, 0, 0, 1\right],$$

$$\left[0, 0, 0, -1, 0, 0, 0, 0, 0\right],$$

$$\left[0, 0, 0, 0, -1, 0, 0, 0, 0\right]\Big], \left[\left[0, 0, 0, u5, u9, 0, 0, -\frac{423}{6050} \, u1 - \frac{13011}{6050} \, u4, -3 \, u2\right.\right. \\ \left.\left.+ \frac{234}{47} \, u3\right],$$

$$\left[0, 0, 0, u7, u10, 0, 0, u2, \frac{12729}{6050} u1 - \frac{47}{6050} u4\right],$$

$$\left[-1, 0, 0, 0, 0, -\frac{8}{39} u2 + \frac{1517}{1833} u3, \frac{3807}{6050} u1 + \frac{2149}{6050} u4, \frac{1}{7} u7 - \frac{19}{7} u8 - \frac{3}{7} u9, \right. \\ \left.-\frac{6}{5} u5 - \frac{19}{15} u6 - \frac{21}{5} u10\right],$$

$$\left[0, 0, 0, 0, 0, 0, 0, 0, 0, 0\right],$$

---


$$\begin{bmatrix} 0, 0, 0, 0, 0, 0, 0, 0, 0 \end{bmatrix},$$

$$\begin{bmatrix} 0, 0, 0, 0, 0, 0, 0, 0, -3 \end{bmatrix},$$

$$\begin{bmatrix} 0, 0, 0, 0, 0, 0, 0, 3, 0 \end{bmatrix},$$

$$\begin{bmatrix} 0, 0, 0, 0, -3, 0, 0, 0, 0 \end{bmatrix},$$

$$\begin{bmatrix} 0, 0, 0, 3, 0, 0, 0, 0, 0 \end{bmatrix}],$$

$$\begin{bmatrix} \left[ 0, 0, 0, -\frac{423}{6050} u1 + \frac{5139}{6050} u4, \frac{16}{13} u2 - \frac{1201}{611} u3, 0, 0, 0, 0 \right], \end{bmatrix}$$

$$\begin{bmatrix} 0, 0, 0, -\frac{16}{39} u2 - \frac{1}{39} u3, -\frac{5421}{6050} u1 - \frac{47}{6050} u4, 0, 0, 0, 0 \end{bmatrix},$$

$$\begin{bmatrix} 0, 0, 0, u8, \frac{3}{5} u5 + \frac{7}{15} u6 + \frac{8}{5} u10, 0, 0, u3, \frac{141}{110} u1 + \frac{47}{110} u4 \end{bmatrix},$$

$$\begin{bmatrix} 0, 0, 0, 0, 0, 0, 0, 0, 0 \end{bmatrix},$$

$$\begin{bmatrix} 0, 0, 0, 0, 0, 0, 0, 0, 0 \end{bmatrix},$$

$$\begin{bmatrix} 0, 0, 0, 0, -6, 0, 0, 0, 0 \end{bmatrix},$$

$$\begin{bmatrix} 0, 0, 0, 6, 0, 0, 0, 0, 0 \end{bmatrix},$$



$$\begin{bmatrix} 0, 0, 0, 0, 0, 0, 0, 0, 0 \\ 0, 0, 0, 0, 0, 0, 0, 0, 0 \end{bmatrix}$$

For some reason Maple has a hard time computing the structure constants from these matrices, so we enter them manually.

```
V80 > HData:=LieAlgebraData([[t1,t2]=t3],[t1,t2,t3],h):DGsetup
      (HData);
```

*Lie algebra: h* (26)

```
V > DGsetup([seq(v||i,i=1..dimM)],m);
```

*frame name: m* (27)

```
m > DGsetup([seq(w||i,i=1..9)],g);
```

*frame name: g* (28)

```
g > rep:=Representation(h,g,MrepMat):
```

```
V > Mrep:=TensorProductOfRepresentations(rep,[seq(dw||i,i=4..9)],
      m);
```

$$Mrep := e1 \rightarrow \begin{bmatrix} 0 & 0 & 0 & 0 & 1 & 0 \\ 0 & 0 & 0 & 0 & 0 & 1 \\ 0 & 0 & 0 & 0 & 0 & 0 \\ 0 & 0 & 0 & 0 & 0 & 0 \\ 0 & 0 & -1 & 0 & 0 & 0 \\ 0 & 0 & 0 & -1 & 0 & 0 \end{bmatrix}, e2 \rightarrow \begin{bmatrix} 0 & 0 & 0 & 0 & 0 & -3 \\ 0 & 0 & 0 & 0 & 3 & 0 \\ 0 & 0 & 0 & 0 & 0 & 0 \\ 0 & 0 & 0 & 0 & 0 & 0 \\ 0 & 0 & 0 & -3 & 0 & 0 \\ 0 & 0 & 3 & 0 & 0 & 0 \end{bmatrix}, e3 \rightarrow$$

$$\begin{bmatrix} 0 & 0 & 0 & -6 & 0 & 0 \\ 0 & 0 & 6 & 0 & 0 & 0 \\ 0 & 0 & 0 & 0 & 0 & 0 \\ 0 & 0 & 0 & 0 & 0 & 0 \\ 0 & 0 & 0 & 0 & 0 & 0 \\ 0 & 0 & 0 & 0 & 0 & 0 \end{bmatrix}$$

```
G > ChangeFrame(g);
```

*g* (30)

We find and solve all linear equations for the bracket.

```
V80 > L2m:=GenerateForms([seq(dw||i,i=4..9)],2):L2mtg:=
      GenerateTensors([L2m,[seq(D_w||i,i=1..9)]]):
```

```
g > G:=DGinfo(rep, "ObjectAttributes")[2,1,1]:conbasG:=DGinfo(G,
      "FrameBaseVectors"):nG:=DGinfo(G, "LieAlgebraDimension")
      :bracket_elements[0]:=evalDG(add(a[i]*L2mtg[i],i=1..nops
      (L2mtg))):
```

```
g > image_elements[1]:=ApplyRepresentation(rep,conbasG[1],
```

```

[ bracket_elements[0]):
g > image_coefficients[1]:=DGinfo(image_elements[1],
  "CoefficientSet")[1..152]:
[
g > kernel_equations[1]:=solve(image_coefficients[1]):
g > bracket_elements[1]:=DGsimplify(subs(kernel_equations[1],
  bracket_elements[0])):

```

```

[ g > image_elements[2]:=ApplyRepresentation(rep,conbasG[2],
  bracket_elements[1]):
[
g > image_coefficients[2]:=DGinfo(image_elements[2],
  "CoefficientSet")[1..38]:
[
g > kernel_equations[2]:=solve(image_coefficients[2]):
g > bracket_elements[2]:=DGsimplify(subs(kernel_equations[2],
  bracket_elements[1])):

```

```

[ g > image_elements[3]:=ApplyRepresentation(rep,conbasG[3],
  bracket_elements[2]):
[
g > image_coefficients[3]:=DGinfo(image_elements[3],
  "CoefficientSet"):
[
g > kernel_equations[3]:=solve(image_coefficients[3]):

```

```

[ g > image_elements[3]:=ApplyRepresentation(rep,conbasG[1],
  bracket_elements[2]):
[
g > image_coefficients[3]:=DGinfo(image_elements[3],
  "CoefficientSet")[1..4]:
[
g > kernel_equations[3]:=solve(image_coefficients[3]):
g > bracket_elements[3]:=DGsimplify(subs(kernel_equations[3],
  bracket_elements[2])):

```

```

[ g > image_elements[4]:=ApplyRepresentation(rep,conbasG[3],
  bracket_elements[3]):
[
g > image_coefficients[4]:=DGinfo(image_elements[4],
  "CoefficientSet");

```

$$\begin{aligned}
image\_coefficients_4 := & \left\{ -\frac{141}{110} u1 a_{62} - \frac{47}{110} a_{62} u4 + a_{63} u3, \frac{141}{110} u1 a_{62} + \frac{47}{110} a_{62} u4 \right. & (31) \\
& - a_{63} u3, -6 a_{84} - \frac{141}{110} a_{63} u1 - \frac{47}{110} u4 a_{63} - a_{62} u3, -6 a_{84} + \frac{141}{110} a_{63} u1 \\
& + \frac{47}{110} u4 a_{63} + a_{62} u3, 6 a_{84} - \frac{141}{110} a_{63} u1 - \frac{47}{110} u4 a_{63} - a_{62} u3, 6 a_{84} + \frac{141}{110} a_{63} u1 \\
& + \frac{47}{110} u4 a_{63} + a_{62} u3, -6 a_{109} + \frac{16}{13} a_{63} u2 - \frac{1201}{611} a_{63} u3 - \frac{423}{6050} u1 a_{62} \\
& + \frac{5139}{6050} a_{62} u4, 6 a_{109} - \frac{16}{13} a_{63} u2 + \frac{1201}{611} a_{63} u3 + \frac{423}{6050} u1 a_{62} - \frac{5139}{6050} a_{62} u4, \\
& -6 a_{110} - \frac{5421}{6050} a_{63} u1 - \frac{47}{6050} u4 a_{63} - \frac{16}{39} a_{62} u2 - \frac{1}{39} a_{62} u3, 6 a_{110} + \frac{5421}{6050} a_{63} u1 \\
& \left. + \frac{47}{6050} u4 a_{63} + \frac{16}{39} a_{62} u2 + \frac{1}{39} a_{62} u3, -6 a_{118} - \frac{16}{13} a_{62} u2 + \frac{1201}{611} a_{62} u3 \right\}
\end{aligned}$$

$$\begin{aligned}
& -\frac{423}{6050} a_{63} u1 + \frac{5139}{6050} u4 a_{63}, 6 a_{118} + \frac{16}{13} a_{62} u2 - \frac{1201}{611} a_{62} u3 + \frac{423}{6050} a_{63} u1 \\
& -\frac{5139}{6050} u4 a_{63}, -6 a_{119} + \frac{5421}{6050} u1 a_{62} + \frac{47}{6050} a_{62} u4 - \frac{16}{39} a_{63} u2 - \frac{1}{39} a_{63} u3, \\
& 6 a_{119} - \frac{5421}{6050} u1 a_{62} - \frac{47}{6050} a_{62} u4 + \frac{16}{39} a_{63} u2 + \frac{1}{39} a_{63} u3, -6 a_{93} + \frac{141}{110} u1 a_{80} \\
& + \frac{47}{110} a_{80} u4 - a_{81} u3 + \frac{3}{5} u5 a_{62} + \frac{7}{15} a_{62} u6 + \frac{8}{5} a_{62} u10 - a_{63} u8, 6 a_{93} \\
& -\frac{141}{110} u1 a_{80} - \frac{47}{110} a_{80} u4 + a_{81} u3 - \frac{3}{5} u5 a_{62} - \frac{7}{15} a_{62} u6 - \frac{8}{5} a_{62} u10 + a_{63} u8, \\
& -6 a_{102} - \frac{141}{110} a_{81} u1 - \frac{47}{110} u4 a_{81} - a_{80} u3 + \frac{3}{5} a_{63} u5 + \frac{7}{15} a_{63} u6 + \frac{8}{5} u10 a_{63} \\
& + a_{62} u8, 6 a_{102} + \frac{141}{110} a_{81} u1 + \frac{47}{110} u4 a_{81} + a_{80} u3 - \frac{3}{5} a_{63} u5 - \frac{7}{15} a_{63} u6 \\
& -\frac{8}{5} u10 a_{63} - a_{62} u8, -6 a_{111} - \frac{141}{110} u1 a_{44} - \frac{47}{110} a_{44} u4 + a_{45} u3 + \frac{3}{5} a_{63} u5 \\
& + \frac{7}{15} a_{63} u6 + \frac{8}{5} u10 a_{63} + a_{62} u8, 6 a_{111} + \frac{141}{110} u1 a_{44} + \frac{47}{110} a_{44} u4 - a_{45} u3 \\
& -\frac{3}{5} a_{63} u5 - \frac{7}{15} a_{63} u6 - \frac{8}{5} u10 a_{63} - a_{62} u8, -6 a_{120} + \frac{141}{110} u1 a_{45} + \frac{47}{110} u4 a_{45} \\
& + a_{44} u3 - \frac{3}{5} u5 a_{62} - \frac{7}{15} a_{62} u6 - \frac{8}{5} a_{62} u10 + a_{63} u8, 6 a_{120} - \frac{141}{110} u1 a_{45} \\
& -\frac{47}{110} u4 a_{45} - a_{44} u3 + \frac{3}{5} u5 a_{62} + \frac{7}{15} a_{62} u6 + \frac{8}{5} a_{62} u10 - a_{63} u8, -6 a_{10} - 6 a_{55} \\
& -\frac{16}{13} a_{45} u2 - \frac{16}{13} a_{80} u2 + \frac{1201}{611} a_{45} u3 + \frac{1201}{611} a_{80} u3 + \frac{423}{6050} u1 a_{44} \\
& -\frac{423}{6050} a_{81} u1 - \frac{5139}{6050} a_{44} u4 + \frac{5139}{6050} u4 a_{81}, -6 a_{11} - 6 a_{56} + \frac{5421}{6050} u1 a_{45} \\
& + \frac{5421}{6050} u1 a_{80} + \frac{47}{6050} u4 a_{45} + \frac{47}{6050} a_{80} u4 + \frac{16}{39} a_{44} u2 - \frac{16}{39} a_{81} u2 + \frac{1}{39} a_{44} u3 \\
& -\frac{1}{39} a_{81} u3, 6 a_{55} + 6 a_{10} + \frac{16}{13} a_{80} u2 + \frac{16}{13} a_{45} u2 - \frac{1201}{611} a_{80} u3 - \frac{1201}{611} a_{45} u3 \\
& + \frac{423}{6050} a_{81} u1 - \frac{423}{6050} u1 a_{44} - \frac{5139}{6050} u4 a_{81} + \frac{5139}{6050} a_{44} u4, 6 a_{56} + 6 a_{11} \\
& -\frac{5421}{6050} u1 a_{80} - \frac{5421}{6050} u1 a_{45} - \frac{47}{6050} a_{80} u4 - \frac{47}{6050} u4 a_{45} + \frac{16}{39} a_{81} u2 \\
& -\frac{16}{39} a_{44} u2 + \frac{1}{39} a_{81} u3 - \frac{1}{39} a_{44} u3, -6 a_{12} - 6 a_{57} - \frac{141}{110} a_{33} u1 - \frac{141}{110} a_{78} u1 \\
& -\frac{47}{110} a_{33} u4 - \frac{47}{110} a_{78} u4 + a_{34} u3 + a_{79} u3 - \frac{3}{5} a_{45} u5 - \frac{3}{5} u5 a_{80} - \frac{7}{15} a_{45} u6 \\
& -\frac{7}{15} a_{80} u6 - \frac{8}{5} u10 a_{45} - \frac{8}{5} a_{80} u10 - a_{44} u8 + a_{81} u8, 6 a_{57} + 6 a_{12} + \frac{141}{110} a_{33} u1 \\
& + \frac{141}{110} a_{78} u1 + \frac{47}{110} a_{33} u4 + \frac{47}{110} a_{78} u4 - a_{34} u3 - a_{79} u3 + \frac{3}{5} u5 a_{80} + \frac{3}{5} a_{45} u5
\end{aligned}$$

$$+ \frac{7}{15} a_{80} u6 + \frac{7}{15} a_{45} u6 + \frac{8}{5} a_{80} u10 + \frac{8}{5} u10 a_{45} + a_{44} u8 - a_{81} u8 \}$$

$$\mathbf{g} > \text{DGinfo}(\text{bracket\_elements}[3], \text{"CoefficientSet"})[1..55];$$

$$\{a_1, a_2, a_3, a_6, a_7, a_{10}, a_{11}, a_{12}, a_{19}, a_{20}, a_{21}, a_{28}, a_{29}, a_{30}, a_{33}, a_{34}, a_{37}, a_{38}, a_{39}, a_{42}, a_{43}, a_{44}, a_{45},$$

$$a_{46}, a_{47}, a_{48}, a_{55}, a_{56}, a_{57}, a_{62}, a_{63}, a_{64}, a_{65}, a_{66}, a_{73}, a_{74}, a_{75}, a_{78}, a_{79}, a_{80}, a_{81}, a_{84}, a_{93}, a_{102},$$

$$a_{109}, a_{110}, a_{111}, a_{118}, a_{119}, a_{120}, a_{127}, a_{128}, a_{129}, a_{132}, a_{133}\}$$

The bracket still has 55 free parameters after solving all linear equations.

$$\mathbf{g} > \text{bracket} := \text{bracket\_elements}[3];$$

$$\mathbf{g} > \text{ChangeFrame}(\mathbf{g});$$

$$g$$

$$\mathbf{V80} > \text{HTensor} := [\text{seq}(\text{convert}(\text{MrepMat}[i], \text{DGtensor}, [[\text{"con\_bas"}, \text{"cov\_bas"}], []]), i=1..nops(\text{MrepMat}))];$$

$$\text{HTensor} := \left[ \left( \frac{u7}{7} - \frac{19u8}{7} - \frac{24u9}{7} \right) \partial_{w1} \otimes dw4 - \left( -\frac{9u5}{5} + \frac{19u6}{15} + \frac{21u10}{5} \right) \partial_{w1} \otimes d \right.$$

$$w5 - \left( \frac{55u2}{39} - \frac{4243u3}{1833} \right) \partial_{w1} \otimes dw8 + u4 \partial_{w1} \otimes dw9 + u6 \partial_{w2} \otimes dw4 + \left( \frac{24u7}{7} \right.$$

$$- \frac{15u8}{7} - \frac{9u9}{7} \left. \right) \partial_{w2} \otimes dw5 + u1 \partial_{w2} \otimes dw8 - \left( \frac{55u2}{117} + \frac{u3}{117} \right) \partial_{w2} \otimes dw9 + \partial_{w3} \otimes d$$

$$w2 + \left( \frac{389u1}{6050} + \frac{423u4}{6050} \right) \partial_{w3} \otimes dw6 + \left( \frac{8u2}{117} - \frac{19u3}{117} \right) \partial_{w3} \otimes dw7 - \left( u6 + 3u10 \right) \partial_{w3}$$

$$\otimes dw8 - \left( \frac{3u7}{7} - \frac{15u8}{7} - \frac{9u9}{7} \right) \partial_{w3} \otimes dw9 + \partial_{w6} \otimes dw8 + \partial_{w7} \otimes dw9 - \partial_{w8} \otimes dw4$$

$$- \partial_{w9} \otimes dw5, u5 \partial_{w1} \otimes dw4 + u9 \partial_{w1} \otimes dw5 - \left( \frac{423u1}{6050} + \frac{13011u4}{6050} \right) \partial_{w1} \otimes dw8 - \left( 3u2 \right.$$

$$- \frac{234u3}{47} \left. \right) \partial_{w1} \otimes dw9 + u7 \partial_{w2} \otimes dw4 + u10 \partial_{w2} \otimes dw5 + u2 \partial_{w2} \otimes dw8 + \left( \frac{12729u1}{6050} \right.$$

$$- \frac{47u4}{6050} \left. \right) \partial_{w2} \otimes dw9 - \partial_{w3} \otimes dw1 - \left( \frac{8u2}{39} - \frac{1517u3}{1833} \right) \partial_{w3} \otimes dw6 + \left( \frac{3807u1}{6050} \right.$$

$$+ \frac{2149u4}{6050} \left. \right) \partial_{w3} \otimes dw7 + \left( \frac{u7}{7} - \frac{19u8}{7} - \frac{3u9}{7} \right) \partial_{w3} \otimes dw8 - \left( \frac{6u5}{5} + \frac{19u6}{15} \right.$$

$$+ \frac{21u10}{5} \left. \right) \partial_{w3} \otimes dw9 - 3 \partial_{w6} \otimes dw9 + 3 \partial_{w7} \otimes dw8 - 3 \partial_{w8} \otimes dw5 + 3 \partial_{w9} \otimes dw4, -$$

$$\left( \frac{423u1}{6050} - \frac{5139u4}{6050} \right) \partial_{w1} \otimes dw4 + \left( \frac{16u2}{13} - \frac{1201u3}{611} \right) \partial_{w1} \otimes dw5 - \left( \frac{16u2}{39} + \frac{u3}{39} \right.$$

$$\left. \right) \partial_{w2} \otimes dw4 - \left( \frac{5421u1}{6050} + \frac{47u4}{6050} \right) \partial_{w2} \otimes dw5 + u8 \partial_{w3} \otimes dw4 + \left( \frac{3u5}{5} + \frac{7u6}{15} \right.$$

$$+ \frac{8u10}{5} \left. \right) \partial_{w3} \otimes dw5 + u3 \partial_{w3} \otimes dw8 + \left( \frac{141u1}{110} + \frac{47u4}{110} \right) \partial_{w3} \otimes dw9 - 6 \partial_{w6} \otimes dw5$$

$$+ 6 \partial_{w7} \otimes dw4 \left. \right]$$

$$\mathbf{V} > \mathbf{A} := (\mathbf{x}, \mathbf{y}, \mathbf{z}) \rightarrow \text{GetComponents}(\text{evalDG}(\text{ContractIndices}(\text{HTensor}[\mathbf{x}],$$

```
HTensor[y],[[2,1]])&minus ContractIndices(HTensor[y],HTensor
[x],[[2,1]])),HTensor)[z]:
```

```
V > B:=(x,y,z)->GetComponents(convert(evalDG(ContractIndices
(HTensor[x],D_w|y,[[2,1]])),DGvector),DGinfo(g,
"FrameBaseVectors"))[z]:
g > C:=(x,y,z)->GetComponents(convert(ContractIndices(D_w|y,
ContractIndices(bracket,D_w|x,[[1,1]]),[[1,1]]),DGvector),
DGinfo(g,"FrameBaseVectors"))[z]:
V > CH:=[seq(seq([q| i,q| j]=add(A(i,j,k)*q| k,k=1..nops(MrepMat)
),i=j+1..nops(MrepMat)),j=1..nops(MrepMat))];
CH:=[q2,q1]=-q3,[q3,q1]=0,[q3,q2]=0] (35)
```

```
L2 > ChangeFrame(g);
```

$g$

```
V > CHM:=[seq(seq([q| i,q| j]=add(B(i,j,k)*q| k,k=1..9),i=1..nops
(MrepMat)),j=4..9)];
```

```
CHM:=[q1,q4]=\left(\frac{1}{7}u7-\frac{19}{7}u8-\frac{24}{7}u9\right)q1+u6q2-q8,[q2,q4]=q1u5+q2u7 (37)
```

$$\begin{aligned}
& + 3q9, [q3,q4] = \left(-\frac{423}{6050}u1 + \frac{5139}{6050}u4\right)q1 + \left(-\frac{16}{39}u2 - \frac{1}{39}u3\right)q2 + u8q3 \\
& + 6q7, [q1,q5] = \left(\frac{9}{5}u5 - \frac{19}{15}u6 - \frac{21}{5}u10\right)q1 + \left(\frac{24}{7}u7 - \frac{15}{7}u8 - \frac{9}{7}u9\right)q2 \\
& - q9, [q2,q5] = q1u9 + q2u10 - 3q8, [q3,q5] = \left(\frac{16}{13}u2 - \frac{1201}{611}u3\right)q1 + \left( \right. \\
& \left. - \frac{5421}{6050}u1 - \frac{47}{6050}u4\right)q2 + \left(\frac{3}{5}u5 + \frac{7}{15}u6 + \frac{8}{5}u10\right)q3 - 6q6, [q1,q6] \\
& = \left(\frac{389}{6050}u1 + \frac{423}{6050}u4\right)q3, [q2,q6] = \left(-\frac{8}{39}u2 + \frac{1517}{1833}u3\right)q3, [q3,q6] = 0, [q1, \\
& q7] = \left(\frac{8}{117}u2 - \frac{19}{117}u3\right)q3, [q2,q7] = \left(\frac{3807}{6050}u1 + \frac{2149}{6050}u4\right)q3, [q3,q7] = 0, \\
& [q1,q8] = \left(-\frac{55}{39}u2 + \frac{4243}{1833}u3\right)q1 + u1q2 + (-u6 - 3u10)q3 + q6, [q2,q8] = \left( \right. \\
& \left. - \frac{423}{6050}u1 - \frac{13011}{6050}u4\right)q1 + u2q2 + \left(\frac{1}{7}u7 - \frac{19}{7}u8 - \frac{3}{7}u9\right)q3 + 3q7, [q3,q8] \\
& = u3q3, [q1,q9] = u4q1 + \left(-\frac{55}{117}u2 - \frac{1}{117}u3\right)q2 + \left(-\frac{3}{7}u7 + \frac{15}{7}u8 \right. \\
& \left. + \frac{9}{7}u9\right)q3 + q7, [q2,q9] = \left(-3u2 + \frac{234}{47}u3\right)q1 + \left(\frac{12729}{6050}u1 - \frac{47}{6050}u4\right)q2 \\
& + \left(-\frac{6}{5}u5 - \frac{19}{15}u6 - \frac{21}{5}u10\right)q3 - 3q6, [q3,q9] = \left(\frac{141}{110}u1 + \frac{47}{110}u4\right)q3]
\end{aligned}$$

```
g > CM:=[seq(seq([q| j,q| i]=add(C(i,j,k)*q| k,k=1..9),i=j+1..9),
j=4..9)];
```

```
CM:=[q4,q5]=-a1q1-a2q2-a3q3+(-a44+a81)q4+(-a45-a80)q5-a6q6 (38)
-a7q7+(a34+a79)q8+(-a33-a78)q9,[q4,q6]=-q1a10-q2a11-q3a12
-q6a45+q7a44+q8a62+q9a63,[q4,q7]=-a19q1-a20q2-a21q3+(-a132
-a44)q6+(-a133-a45)q7+a63q8-a62q9,[q4,q8]=-q1a28-q2a29-q3a30
```

$$\begin{aligned}
& -q4 a_{62} - q5 a_{63} - q6 a_{33} - q7 a_{34} - q8 a_{45} + q9 a_{44}, [q4, q9] = -q1 a_{37} - q2 a_{38} \\
& -q3 a_{39} - q4 a_{63} + q5 a_{62} - q6 a_{42} - q7 a_{43} - q8 a_{44} - q9 a_{45}, [q5, q6] = -a_{46} q1 \\
& -a_{47} q2 - a_{48} q3 + (a_{132} - a_{81}) q6 + (a_{133} + a_{80}) q7 + a_{63} q8 - a_{62} q9, [q5, q7] = \\
& -q1 a_{55} - q2 a_{56} - q3 a_{57} - q6 a_{80} - q7 a_{81} - q8 a_{62} - q9 a_{63}, [q5, q8] = -a_{64} q1 \\
& -a_{65} q2 - a_{66} q3 - a_{63} q4 + a_{62} q5 + (a_{34} + a_{79} - a_{42}) q6 + (-a_{33} - a_{78} - a_{43}) q7 \\
& -a_{81} q8 + a_{80} q9, [q5, q9] = -q1 a_{73} - q2 a_{74} - q3 a_{75} + q4 a_{62} + q5 a_{63} - q6 a_{78} \\
& -q7 a_{79} - q8 a_{80} - q9 a_{81}, [q6, q7] = -a_{84} q3, [q6, q8] = q1 a_{118} + q2 a_{119} - q3 a_{93} \\
& + q6 a_{62} + q7 a_{63}, [q6, q9] = -q1 a_{109} - q2 a_{110} - q3 a_{102} + q6 a_{63} - q7 a_{62}, [q7, q8] = \\
& -q1 a_{109} - q2 a_{110} - q3 a_{111} + q6 a_{63} - q7 a_{62}, [q7, q9] = -q1 a_{118} - q2 a_{119} - q3 a_{120} \\
& -q6 a_{62} - q7 a_{63}, [q8, q9] = -q1 a_{127} - q2 a_{128} - q3 a_{129} - q6 a_{132} - q7 a_{133}
\end{aligned}$$

**V > KData:=LieAlgebraData([op(CH),op(CHM),op(CM)],[seq(q|i,i=1..nops(MrepMat)+dimM)]);**

$$\begin{aligned}
KData := [e1, e2] = e3, [e1, e3] = 0, [e1, e4] &= \left( \frac{u7}{7} - \frac{19 u8}{7} - \frac{24 u9}{7} \right) e1 + u6 e2 - e8, \\
[e1, e5] &= -\left( -\frac{9 u5}{5} + \frac{19 u6}{15} + \frac{21 u10}{5} \right) e1 + \left( \frac{24 u7}{7} - \frac{15 u8}{7} - \frac{9 u9}{7} \right) e2 - e9, \\
[e1, e6] &= \left( \frac{389 u1}{6050} + \frac{423 u4}{6050} \right) e3, [e1, e7] = \left( \frac{8 u2}{117} - \frac{19 u3}{117} \right) e3, [e1, e8] = -\left( \frac{55 u2}{39} \right. \\
& \left. - \frac{4243 u3}{1833} \right) e1 + u1 e2 - (u6 + 3 u10) e3 + e6, [e1, e9] = u4 e1 - \left( \frac{55 u2}{117} + \frac{u3}{117} \right) e2 \\
& - \left( \frac{3 u7}{7} - \frac{15 u8}{7} - \frac{9 u9}{7} \right) e3 + e7, [e2, e3] = 0, [e2, e4] = u5 e1 + u7 e2 + 3 e9, [e2, \\
e5] &= u9 e1 + u10 e2 - 3 e8, [e2, e6] = -\left( \frac{8 u2}{39} - \frac{1517 u3}{1833} \right) e3, [e2, e7] = \left( \frac{3807 u1}{6050} \right. \\
& \left. + \frac{2149 u4}{6050} \right) e3, [e2, e8] = -\left( \frac{423 u1}{6050} + \frac{13011 u4}{6050} \right) e1 + u2 e2 + \left( \frac{u7}{7} - \frac{19 u8}{7} \right. \\
& \left. - \frac{3 u9}{7} \right) e3 + 3 e7, [e2, e9] = -\left( 3 u2 - \frac{234 u3}{47} \right) e1 + \left( \frac{12729 u1}{6050} - \frac{47 u4}{6050} \right) e2 - \\
& \left( \frac{6 u5}{5} + \frac{19 u6}{15} + \frac{21 u10}{5} \right) e3 - 3 e6, [e3, e4] = -\left( \frac{423 u1}{6050} - \frac{5139 u4}{6050} \right) e1 - \left( \frac{16 u2}{39} \right. \\
& \left. + \frac{u3}{39} \right) e2 + u8 e3 + 6 e7, [e3, e5] = \left( \frac{16 u2}{13} - \frac{1201 u3}{611} \right) e1 - \left( \frac{5421 u1}{6050} + \frac{47 u4}{6050} \right) e2 \\
& + \left( \frac{3 u5}{5} + \frac{7 u6}{15} + \frac{8 u10}{5} \right) e3 - 6 e6, [e3, e6] = 0, [e3, e7] = 0, [e3, e8] = u3 e3, [e3, e9] \\
& = \left( \frac{141 u1}{110} + \frac{47 u4}{110} \right) e3, [e4, e5] = -a_1 e1 - a_2 e2 - a_3 e3 - (-a_{81} + a_{44}) e4 - (a_{80} \\
& + a_{45}) e5 - a_6 e6 - a_7 e7 + (a_{34} + a_{79}) e8 - (a_{33} + a_{78}) e9, [e4, e6] = -a_{10} e1 - a_{11} e2 \\
& - a_{12} e3 - a_{45} e6 + a_{44} e7 + a_{62} e8 + a_{63} e9, [e4, e7] = -a_{19} e1 - a_{20} e2 - a_{21} e3 - (a_{132} \\
& + a_{44}) e6 - (a_{133} + a_{45}) e7 + a_{63} e8 - a_{62} e9, [e4, e8] = -a_{28} e1 - a_{29} e2 - a_{30} e3 \\
& - a_{62} e4 - a_{63} e5 - a_{33} e6 - a_{34} e7 - a_{45} e8 + a_{44} e9, [e4, e9] = -a_{37} e1 - a_{38} e2
\end{aligned} \tag{39}$$

$$\begin{aligned}
& -a_{39} e3 - a_{63} e4 + a_{62} e5 - a_{42} e6 - a_{43} e7 - a_{44} e8 - a_{45} e9, [e5, e6] = -a_{46} e1 \\
& -a_{47} e2 - a_{48} e3 - (-a_{132} + a_{81}) e6 + (a_{133} + a_{80}) e7 + a_{63} e8 - a_{62} e9, [e5, e7] = \\
& -a_{55} e1 - a_{56} e2 - a_{57} e3 - a_{80} e6 - a_{81} e7 - a_{62} e8 - a_{63} e9, [e5, e8] = -a_{64} e1 \\
& -a_{65} e2 - a_{66} e3 - a_{63} e4 + a_{62} e5 + (a_{34} + a_{79} - a_{42}) e6 - (a_{33} + a_{78} + a_{43}) e7 - a_{81} e8 \\
& + a_{80} e9, [e5, e9] = -a_{73} e1 - a_{74} e2 - a_{75} e3 + a_{62} e4 + a_{63} e5 - a_{78} e6 - a_{79} e7 \\
& -a_{80} e8 - a_{81} e9, [e6, e7] = -a_{84} e3, [e6, e8] = a_{118} e1 + a_{119} e2 - a_{93} e3 + a_{62} e6 \\
& + a_{63} e7, [e6, e9] = -a_{109} e1 - a_{110} e2 - a_{102} e3 + a_{63} e6 - a_{62} e7, [e7, e8] = -a_{109} e1 \\
& -a_{110} e2 - a_{111} e3 + a_{63} e6 - a_{62} e7, [e7, e9] = -a_{118} e1 - a_{119} e2 - a_{120} e3 - a_{62} e6 \\
& -a_{63} e7, [e8, e9] = -a_{127} e1 - a_{128} e2 - a_{129} e3 - a_{132} e6 - a_{133} e7
\end{aligned}$$

These are the most general structure constants for g.

```
h > DGsetup(KData);
```

*Lie algebra: L1*

(40)

```
h > Jaceq:=Query({seq(a[i],i=1..300),seq(u[i],i=1..10)},"Jacobi")
      :
```

```
g > Jaceq[2];
```

```
{u4, u5, u9, a109, a118, -3 u1, 3 u1, 3 u10, -3 u2, 3 u2, -234/47 u3, 110/47 u3, -3 u6, -3 u7, -6 u8, -3 a110, 3 a110, -a118, -3 a119, 3 a119, -3 u1, -u1}
```

There are linear equations in  $u_i$  coming from the Jacobi identity. The only solution is all  $u_i=0$  which means the decomposable case.

### Part 1.3: the 3D algebra L1.

```
> restart:with(DifferentialGeometry): with(Tensor): with(Tools):
  with(LieAlgebras):
```

```
h > dimM:=6;
```

*dimM := 6*

(42)

These representation matrices come from another worksheet. The cohomology is 4D.

```
V > MrepMat := [Matrix(9, 9, {(1, 1) = 0, (1, 2) = 0, (1, 3) = 0,
      (1, 4) = 0, (1, 5) = 0, (1, 6) = 0, (1, 7) = 0, (1, 8) = 0,
```

```

(1, 9) = 0, (2, 1) = 0, (2, 2) = -1, (2, 3) = 0, (2, 4) = 0,
(2, 5) = 0, (2, 6) = 0, (2, 7) = 0, (2, 8) = 0, (2, 9) = 0,
(3, 1) = 0, (3, 2) = 0, (3, 3) = -2, (3, 4) = 0, (3, 5) = 0,
(3, 6) = 0, (3, 7) = 0, (3, 8) = 0, (3, 9) = 0, (4, 1) = 0,
(4, 2) = 0, (4, 3) = 0, (4, 4) = 1, (4, 5) = 0, (4, 6) = 0,
(4, 7) = 0, (4, 8) = 0, (4, 9) = 0, (5, 1) = 0, (5, 2) = 0,
(5, 3) = 0, (5, 4) = 0, (5, 5) = 1, (5, 6) = 0, (5, 7) = 0,
(5, 8) = 0, (5, 9) = 0, (6, 1) = 0, (6, 2) = 0, (6, 3) = 0,
(6, 4) = 0, (6, 5) = 0, (6, 6) = -1, (6, 7) = 0, (6, 8) = 0,
(6, 9) = 0, (7, 1) = 0, (7, 2) = 0, (7, 3) = 0, (7, 4) = 0,
(7, 5) = 0, (7, 6) = 0, (7, 7) = -1, (7, 8) = 0, (7, 9) = 0,
(8, 1) = 0, (8, 2) = 0, (8, 3) = 0, (8, 4) = 0, (8, 5) = 0,
(8, 6) = 0, (8, 7) = 0, (8, 8) = 0, (8, 9) = 0, (9, 1) = 0,
(9, 2) = 0, (9, 3) = 0, (9, 4) = 0, (9, 5) = 0, (9, 6) = 0,
(9, 7) = 0, (9, 8) = 0, (9, 9) = 0}}, Matrix(9, 9, {(1, 1) =
0, (1, 2) = 0, (1, 3) = 0, (1, 4) = -(6/5)*u2+(12/5)*u4, (1,
5) = (6/5)*u1-(12/5)*u3, (1, 6) = 0, (1, 7) = 0, (1, 8) = 0,
(1, 9) = 0, (2, 1) = 1, (2, 2) = 0, (2, 3) = 0, (2, 4) = 0,
(2, 5) = 0, (2, 6) = 0, (2, 7) = 0, (2, 8) = 6*u2, (2, 9) =
-6*u1, (3, 1) = 0, (3, 2) = 0, (3, 3) = 0, (3, 4) = 0, (3, 5)
= 0, (3, 6) = u3, (3, 7) = u4, (3, 8) = 0, (3, 9) = 0, (4, 1)
= 0, (4, 2) = 0, (4, 3) = 0, (4, 4) = 0, (4, 5) = 0, (4, 6) =
0, (4, 7) = 0, (4, 8) = 0, (4, 9) = 0, (5, 1) = 0, (5, 2) =
0, (5, 3) = 0, (5, 4) = 0, (5, 5) = 0, (5, 6) = 0, (5, 7) =
0, (5, 8) = 0, (5, 9) = 0, (6, 1) = 0, (6, 2) = 0, (6, 3) =
0, (6, 4) = 0, (6, 5) = 0, (6, 6) = 0, (6, 7) = 0, (6, 8) =
1, (6, 9) = 0, (7, 1) = 0, (7, 2) = 0, (7, 3) = 0, (7, 4) =
0, (7, 5) = 0, (7, 6) = 0, (7, 7) = 0, (7, 8) = 0, (7, 9) =
1, (8, 1) = 0, (8, 2) = 0, (8, 3) = 0, (8, 4) = -1, (8, 5) =
0, (8, 6) = 0, (8, 7) = 0, (8, 8) = 0, (8, 9) = 0, (9, 1) =
0, (9, 2) = 0, (9, 3) = 0, (9, 4) = 0, (9, 5) = -1, (9, 6) =
0, (9, 7) = 0, (9, 8) = 0, (9, 9) = 0}}, Matrix(9, 9, {(1, 1)
= 0, (1, 2) = 0, (1, 3) = 0, (1, 4) = 0, (1, 5) = 0, (1, 6) =
0, (1, 7) = 0, (1, 8) = 0, (1, 9) = 0, (2, 1) = 0, (2, 2) =
0, (2, 3) = 0, (2, 4) = u1, (2, 5) = u2, (2, 6) = 0, (2, 7) =
0, (2, 8) = 0, (2, 9) = 0, (3, 1) = 2, (3, 2) = 0, (3, 3) =
0, (3, 4) = 0, (3, 5) = 0, (3, 6) = 0, (3, 7) = 0, (3, 8) = -
(12/5)*u2-(6/5)*u4, (3, 9) = (12/5)*u1+(6/5)*u3, (4, 1) = 0,
(4, 2) = 0, (4, 3) = 0, (4, 4) = 0, (4, 5) = 0, (4, 6) = 0,
(4, 7) = 0, (4, 8) = 0, (4, 9) = 0, (5, 1) = 0, (5, 2) = 0,
(5, 3) = 0, (5, 4) = 0, (5, 5) = 0, (5, 6) = 0, (5, 7) = 0,
(5, 8) = 0, (5, 9) = 0, (6, 1) = 0, (6, 2) = 0, (6, 3) = 0,
(6, 4) = 0, (6, 5) = -6, (6, 6) = 0, (6, 7) = 0, (6, 8) = 0,
(6, 9) = 0, (7, 1) = 0, (7, 2) = 0, (7, 3) = 0, (7, 4) = 6,
(7, 5) = 0, (7, 6) = 0, (7, 7) = 0, (7, 8) = 0, (7, 9) = 0,
(8, 1) = 0, (8, 2) = 0, (8, 3) = 0, (8, 4) = 0, (8, 5) = 0,
(8, 6) = 0, (8, 7) = 0, (8, 8) = 0, (8, 9) = 0, (9, 1) = 0,
(9, 2) = 0, (9, 3) = 0, (9, 4) = 0, (9, 5) = 0, (9, 6) = 0,
(9, 7) = 0, (9, 8) = 0, (9, 9) = 0}}]};

```



$$MrepMat := \begin{bmatrix} \begin{bmatrix} 0 & 0 & 0 & 0 & 0 & 0 & 0 & 0 & 0 \\ 0 & -1 & 0 & 0 & 0 & 0 & 0 & 0 & 0 \\ 0 & 0 & -2 & 0 & 0 & 0 & 0 & 0 & 0 \\ 0 & 0 & 0 & 1 & 0 & 0 & 0 & 0 & 0 \\ 0 & 0 & 0 & 0 & 1 & 0 & 0 & 0 & 0 \\ 0 & 0 & 0 & 0 & 0 & -1 & 0 & 0 & 0 \\ 0 & 0 & 0 & 0 & 0 & 0 & -1 & 0 & 0 \\ 0 & 0 & 0 & 0 & 0 & 0 & 0 & 0 & 0 \\ 0 & 0 & 0 & 0 & 0 & 0 & 0 & 0 & 0 \end{bmatrix} \end{bmatrix}, \quad (43)$$

$$\begin{bmatrix} 0 & 0 & 0 & -\frac{6}{5}u_2 + \frac{12}{5}u_4 & \frac{6}{5}u_1 - \frac{12}{5}u_3 & 0 & 0 & 0 & 0 \\ 1 & 0 & 0 & 0 & 0 & 0 & 0 & 6u_2 & -6u_1 \\ 0 & 0 & 0 & 0 & 0 & u_3 & u_4 & 0 & 0 \\ 0 & 0 & 0 & 0 & 0 & 0 & 0 & 0 & 0 \\ 0 & 0 & 0 & 0 & 0 & 0 & 0 & 0 & 0 \\ 0 & 0 & 0 & 0 & 0 & 0 & 0 & 1 & 0 \\ 0 & 0 & 0 & 0 & 0 & 0 & 0 & 0 & 1 \\ 0 & 0 & 0 & -1 & 0 & 0 & 0 & 0 & 0 \\ 0 & 0 & 0 & 0 & -1 & 0 & 0 & 0 & 0 \end{bmatrix},$$

$$\begin{bmatrix} 0 & 0 & 0 & 0 & 0 & 0 & 0 & 0 & 0 \\ 0 & 0 & 0 & u_1 & u_2 & 0 & 0 & 0 & 0 \\ 2 & 0 & 0 & 0 & 0 & 0 & 0 & -\frac{12}{5}u_2 - \frac{6}{5}u_4 & \frac{12}{5}u_1 + \frac{6}{5}u_3 \\ 0 & 0 & 0 & 0 & 0 & 0 & 0 & 0 & 0 \\ 0 & 0 & 0 & 0 & 0 & 0 & 0 & 0 & 0 \\ 0 & 0 & 0 & 0 & -6 & 0 & 0 & 0 & 0 \\ 0 & 0 & 0 & 6 & 0 & 0 & 0 & 0 & 0 \\ 0 & 0 & 0 & 0 & 0 & 0 & 0 & 0 & 0 \\ 0 & 0 & 0 & 0 & 0 & 0 & 0 & 0 & 0 \end{bmatrix}$$

$$\text{V80} > \text{HData} := \text{LieAlgebraData}(MrepMat, h) : \text{DGsetup}(HData);$$

Lie algebra: h (44)

$$\text{V} > \text{DGsetup}([\text{seq}(v || i, i=1..dimM)], m);$$

frame name: m (45)

$$\text{m} > \text{DGsetup}([\text{seq}(w || i, i=1..9)], g);$$

frame name: g (46)

```

g > rep:=Representation(h,g,MrepMat):
V > Mrep:=TensorProductOfRepresentations(rep,[seq(dw||i,i=4..9)],
m);

```

$$Mrep := e1 \rightarrow \begin{bmatrix} -1 & 0 & 0 & 0 & 0 & 0 \\ 0 & -1 & 0 & 0 & 0 & 0 \\ 0 & 0 & 1 & 0 & 0 & 0 \\ 0 & 0 & 0 & 1 & 0 & 0 \\ 0 & 0 & 0 & 0 & 0 & 0 \\ 0 & 0 & 0 & 0 & 0 & 0 \end{bmatrix}, e2 \rightarrow \begin{bmatrix} 0 & 0 & 0 & 0 & 1 & 0 \\ 0 & 0 & 0 & 0 & 0 & 1 \\ 0 & 0 & 0 & 0 & 0 & 0 \\ 0 & 0 & 0 & 0 & 0 & 0 \\ 0 & 0 & -1 & 0 & 0 & 0 \\ 0 & 0 & 0 & -1 & 0 & 0 \end{bmatrix}, e3 \rightarrow$$

(47)

$$\begin{bmatrix} 0 & 0 & 0 & -6 & 0 & 0 \\ 0 & 0 & 6 & 0 & 0 & 0 \\ 0 & 0 & 0 & 0 & 0 & 0 \\ 0 & 0 & 0 & 0 & 0 & 0 \\ 0 & 0 & 0 & 0 & 0 & 0 \\ 0 & 0 & 0 & 0 & 0 & 0 \end{bmatrix}$$

```

G > ChangeFrame(g);

```

$g$

(48)

We find and solve all linear equations for the bracket.

```

V80 > L2m:=GenerateForms([seq(dw||i,i=4..9)],2):L2mtg:=
GenerateTensors([L2m,[seq(D_w||i,i=1..9)]]):
g > G:=DGinfo(rep, "ObjectAttributes")[2,1,1]:conbasG:=DGinfo(G,
"FrameBaseVectors"):nG:=DGinfo(G, "LieAlgebraDimension")
:bracket_elements[0]:=evalDG(add(a[i]*L2mtg[i],i=1..nops
(L2mtg))):

```

```

g > image_elements[1]:=ApplyRepresentation(rep,conbasG[1],
bracket_elements[1-1]):
g > image_coefficients[1]:=DGinfo(image_elements[1],
"CoefficientSet"):
g > kernel_equations[1]:=solve(image_coefficients[1]):
g > bracket_elements[1]:=DGSimplify(subs(kernel_equations[1],
bracket_elements[1-1])):

```

```

g > image_elements[2]:=ApplyRepresentation(rep,conbasG[2],
bracket_elements[2-1]):
g > image_coefficients[2]:=DGinfo(image_elements[2],
"CoefficientSet")[1..40];

```

$image\_coefficients_2 := \{-a_{31} - a_{17}, a_{31} + a_{17}, -a_{32} - a_{18}, a_{32} + a_{18}, -a_{40} + a_{67}, -a_{41} + a_{68},$   
 $-a_{67} + a_{40}, -a_{68} + a_{41}, -a_{76} - a_{62}, a_{76} + a_{62}, -a_{77} - a_{63}, a_{77} + a_{63}, -a_{96} + a_{17}, a_{96}$   
 $-a_{17}, -a_{97} + a_{18}, a_{97} - a_{18}, -a_{105} + a_{53}, a_{105} - a_{53}, -a_{106} + a_{54}, a_{106} - a_{54}, -a_{114} + a_{26},$   
 $a_{114} - a_{26}, -a_{115} + a_{27}, a_{115} - a_{27}, -a_{123} + a_{62}, a_{123} - a_{62}, -a_{124} + a_{63}, a_{124} - a_{63}, -a_{134}$

(49)

$$+ a_{40} + a_{26}, -a_{134} - a_{67} - a_{53}, -a_{134} + a_{105} - a_{114}, a_{134} - a_{40} - a_{26}, a_{134} + a_{67} + a_{53}, \\ a_{134} + a_{114} - a_{105}, -a_{135} + a_{41} + a_{27}, -a_{135} - a_{68} - a_{54}, -a_{135} + a_{106} - a_{115}, a_{135} - a_{41} \\ - a_{27}, a_{135} + a_{68} + a_{54}, a_{135} + a_{115} - a_{106}\}$$

```
g > kernel_equations[2]:=solve(image_coefficients[2]):
g > bracket_elements[2]:=DGsimplify(subs(kernel_equations[2],
bracket_elements[2-1])):
```

```
g > image_elements[3]:=ApplyRepresentation(rep,conbasG[3],
bracket_elements[3-1]):
g > image_coefficients[3]:=DGinfo(image_elements[3],
"CoefficientSet")[1..16];
image_coefficients3 := { -2 a127, 2 a127, -6 a10 - 6 a55, -6 a17 - 6 a62, 6 a17 + 6 a27, -6 a18
- 6 a63, -6 a26 + 6 a18, 6 a26 - 6 a18, 6 a26 + 6 a63, -6 a27 - 6 a17, 6 a55 + 6 a10, -6 a62
+ 6 a27, 6 a62 + 6 a17, 6 a62 - 6 a27, -6 a63 - 6 a26, 6 a63 + 6 a18}
```

(50)

```
g > kernel_equations[3]:=solve(image_coefficients[3]):
g > bracket_elements[3]:=DGsimplify(subs(kernel_equations[3],
bracket_elements[3-1])):
```

```
g > image_elements[4]:=ApplyRepresentation(rep,conbasG[2],
bracket_elements[4-1]):
g > image_coefficients[4]:=DGinfo(image_elements[4],
"CoefficientSet")[1..2];
image_coefficients4 := { a101 - a110, a110 - a101}
```

(51)

```
g > kernel_equations[4]:=solve(image_coefficients[4]):
g > bracket_elements[4]:=DGsimplify(subs(kernel_equations[4],
bracket_elements[4-1])):
```

```
g > image_elements[5]:=ApplyRepresentation(rep,conbasG[3],
bracket_elements[5-1]):
g > image_coefficients[5]:=DGinfo(image_elements[5],
"CoefficientSet");
```

$$image\_coefficients_5 := \left\{ -\frac{12}{5} u1 a_{62} - \frac{6}{5} u3 a_{62} - \frac{12}{5} u2 a_{63} - \frac{6}{5} u4 a_{63} - 2 a_{19}, \right. \\ -\frac{12}{5} u1 a_{62} - \frac{6}{5} u3 a_{62} - \frac{12}{5} u2 a_{63} - \frac{6}{5} u4 a_{63} - 2 a_{46}, \frac{12}{5} u1 a_{62} + \frac{6}{5} u3 a_{62} \\ + \frac{12}{5} u2 a_{63} + \frac{6}{5} u4 a_{63} + 2 a_{19}, \frac{12}{5} u1 a_{62} + \frac{6}{5} u3 a_{62} + \frac{12}{5} u2 a_{63} + \frac{6}{5} u4 a_{63} \\ + 2 a_{46}, -6 a_{84} - \frac{12}{5} a_{63} u1 - \frac{6}{5} a_{63} u3 + \frac{12}{5} a_{62} u2 + \frac{6}{5} a_{62} u4 - 2 a_{55}, -6 a_{84} \\ + \frac{12}{5} a_{63} u1 + \frac{6}{5} a_{63} u3 - \frac{12}{5} a_{62} u2 - \frac{6}{5} a_{62} u4 + 2 a_{55}, 6 a_{84} - \frac{12}{5} a_{63} u1 \\ - \frac{6}{5} a_{63} u3 + \frac{12}{5} a_{62} u2 + \frac{6}{5} a_{62} u4 - 2 a_{55}, 6 a_{84} + \frac{12}{5} a_{63} u1 + \frac{6}{5} a_{63} u3 \\ \left. - \frac{12}{5} a_{62} u2 - \frac{6}{5} a_{62} u4 + 2 a_{55}, -u1 a_{63} + u2 a_{62} - 6 a_{92}, u1 a_{63} - u2 a_{62} + 6 a_{92}, \right\}$$

(52)

$$\{-u_1 a_{62} - u_2 a_{63} + 6 a_{110}, u_1 a_{62} + u_2 a_{63} - 6 a_{110}, -u_1 a_{63} + u_2 a_{62} + 6 a_{119}, u_1 a_{63} - u_2 a_{62} - 6 a_{119}\}$$

```
> bracket:=bracket_elements[4]:
> DGinfo(bracket,"CoefficientSet")[1..9];
{a19, a46, a55, a62, a63, a84, a92, a110, a119}
```

(53)

There are 9 free parameters in this bracket.

```
V80 > HTensor:=[seq(convert(MrepMat[i],DGtensor,[["con_bas",
"cov_bas"],[]]),i=1..nops(MrepMat))];
```

$$HTensor := \left[ -\partial_{w2} \otimes dw2 - 2 \partial_{w3} \otimes dw3 + \partial_{w4} \otimes dw4 + \partial_{w5} \otimes dw5 - \partial_{w6} \otimes dw6 - \partial_{w7} \otimes dw7, \right. \\ \left. - \left( \frac{6 u2}{5} - \frac{12 u4}{5} \right) \partial_{w1} \otimes dw4 + \left( \frac{6 u1}{5} - \frac{12 u3}{5} \right) \partial_{w1} \otimes dw5 + \partial_{w2} \otimes dw1 \right. \\ \left. + 6 u2 \partial_{w2} \otimes dw8 - 6 u1 \partial_{w2} \otimes dw9 + u3 \partial_{w3} \otimes dw6 + u4 \partial_{w3} \otimes dw7 + \partial_{w6} \otimes dw8 + \partial_{w7} \otimes dw9 \right. \\ \left. - \partial_{w8} \otimes dw4 - \partial_{w9} \otimes dw5, u1 \partial_{w2} \otimes dw4 + u2 \partial_{w2} \otimes dw5 + 2 \partial_{w3} \otimes dw1 - \right. \\ \left. \left( \frac{12 u2}{5} + \frac{6 u4}{5} \right) \partial_{w3} \otimes dw8 + \left( \frac{12 u1}{5} + \frac{6 u3}{5} \right) \partial_{w3} \otimes dw9 - 6 \partial_{w6} \otimes dw5 + 6 \partial_{w7} \otimes dw4 \right]$$
(54)

```
V > A:=(x,y,z)->GetComponents(evalDG(ContractIndices(HTensor[x],
HTensor[y],[[2,1]])&minus ContractIndices(HTensor[y],HTensor
[x],[[2,1]])),HTensor)[z]:
V > B:=(x,y,z)->GetComponents(convert(evalDG(ContractIndices
(HTensor[x],D_w|y,[[2,1]])),DGvector),DGinfo(g,
"FrameBaseVectors"))[z]:
g > C:=(x,y,z)->GetComponents(convert(ContractIndices(D_w|y,
ContractIndices(bracket,D_w|x,[[1,1]]),[[1,1]]),DGvector),
DGinfo(g,"FrameBaseVectors"))[z]:
V > CH:=[seq(seq([q| |i,q| |j]=add(A(i,j,k)*q| |k,k=1..nops(MrepMat)
),i=j+1..nops(MrepMat)),j=1..nops(MrepMat))];
CH:=[[q2,q1]=q2,[q3,q1]=2 q3,[q3,q2]=0]
```

(55)

```
L2 > ChangeFrame(g);
```

$$g$$
(56)

```
V > CHM:=[seq(seq([q| |i,q| |j]=add(B(i,j,k)*q| |k,k=1..9),i=1..nops
(MrepMat)),j=4..9)];
```

$$CHM := \left[ [q1, q4] = q4, [q2, q4] = \left( -\frac{6}{5} u2 + \frac{12}{5} u4 \right) q1 - q8, [q3, q4] = q2 u1 + 6 q7, \right. \\ [q1, q5] = q5, [q2, q5] = \left( \frac{6}{5} u1 - \frac{12}{5} u3 \right) q1 - q9, [q3, q5] = q2 u2 - 6 q6, [q1, q6] = \\ -q6, [q2, q6] = u3 q3, [q3, q6] = 0, [q1, q7] = -q7, [q2, q7] = u4 q3, [q3, q7] = 0, [q1, \\ q8] = 0, [q2, q8] = 6 q2 u2 + q6, [q3, q8] = \left( -\frac{12}{5} u2 - \frac{6}{5} u4 \right) q3, [q1, q9] = 0, [q2, q9]$$
(57)

$$= -6 q_2 u_1 + q_7, [q_3, q_9] = \left( \frac{12}{5} u_1 + \frac{6}{5} u_3 \right) q_3 \Big]$$

```
g > CM:=[seq(seq([q|j,q|i]=add(C(i,j,k)*q|k,k=1..9),i=j+1..9),
j=4..9)];
```

```
CM:=[q4,q5]=0,[q4,q6]=q1 a55 + q8 a62 + q9 a63,[q4,q7]=-q1 a19 + q8 a63 - q9 a62,[q4,q8]=-q4 a62 - q5 a63,[q4,q9]=-q4 a63
```

```
V > KData:=LieAlgebraData([op(CH),op(CHM),op(CM)],[seq(q|i,i=1..
nops(MrepMat)+dimM)]);
```

```
KData := [e1, e2] = -e2, [e1, e3] = -2 e3, [e1, e4] = e4, [e1, e5] = e5, [e1, e6] = -e6, [e1, (59)
```

$$e7] = -e7, [e1, e8] = 0, [e1, e9] = 0, [e2, e3] = 0, \left[ e2, e4 \right] = -\left( \frac{6 u_2}{5} - \frac{12 u_4}{5} \right) e1 - e8,$$

$$\left[ e2, e5 \right] = \left( \frac{6 u_1}{5} - \frac{12 u_3}{5} \right) e1 - e9, [e2, e6] = u_3 e3, [e2, e7] = u_4 e3, [e2, e8] = 6 u_2 e2$$

$$+ e6, [e2, e9] = -6 u_1 e2 + e7, [e3, e4] = u_1 e2 + 6 e7, [e3, e5] = u_2 e2 - 6 e6, [e3, e6]$$

$$] = 0, [e3, e7] = 0, \left[ e3, e8 \right] = -\left( \frac{12 u_2}{5} + \frac{6 u_4}{5} \right) e3, \left[ e3, e9 \right] = \left( \frac{12 u_1}{5} + \frac{6 u_3}{5} \right) e3,$$

$$[e4, e5] = 0, [e4, e6] = a_{55} e1 + a_{62} e8 + a_{63} e9, [e4, e7] = -a_{19} e1 + a_{63} e8 - a_{62} e9,$$

$$[e4, e8] = -a_{62} e4 - a_{63} e5, [e4, e9] = -a_{63} e4 + a_{62} e5, [e5, e6] = -a_{46} e1 + a_{63} e8$$

$$- a_{62} e9, [e5, e7] = -a_{55} e1 - a_{62} e8 - a_{63} e9, [e5, e8] = -a_{63} e4 + a_{62} e5, [e5, e9]$$

$$] = a_{62} e4 + a_{63} e5, [e6, e7] = -a_{84} e3, [e6, e8] = -a_{92} e2 + a_{62} e6 + a_{63} e7, [e6, e9] =$$

$$- a_{110} e2 + a_{63} e6 - a_{62} e7, [e7, e8] = -a_{110} e2 + a_{63} e6 - a_{62} e7, [e7, e9] = -a_{119} e2$$

$$- a_{62} e6 - a_{63} e7, [e8, e9] = 0$$

These are the most general structure constants for g.

```
h > DGsetup(KData);
```

*Lie algebra: L2*

(60)

```
h > Jaceq:=Query({seq(u|i,i=1..4),seq(a|i,i=1..9)},"Jacobi");
```

```
Jaceq:=false, {u1, u2, a19, a46, a92, a110, a119, -6 u1, -u1, 6 u1, 6 u2, -6 u3, 6 u4, -a19, -a46, (61)
```

$$-a_{110}, -\frac{67}{5} u_1 - \frac{36}{5} u_3, -\frac{6}{5} u_1 + \frac{12}{5} u_3, \frac{72}{5} u_1 + \frac{36}{5} u_3, -\frac{67}{5} u_2 - \frac{36}{5} u_4,$$

$$-\frac{6}{5} u_2 + \frac{12}{5} u_4, \frac{6}{5} u_2 - \frac{12}{5} u_4, \frac{72}{5} u_2 + \frac{36}{5} u_4, \frac{42}{5} u_3 - \frac{6}{5} u_1, -\frac{42}{5} u_4$$

$$+ \frac{6}{5} u_2, \frac{6}{5} u_2^2 - \frac{12}{5} u_2 u_4 + \frac{6}{5} u_1^2 - \frac{12}{5} u_1 u_3, -u_4 a_{63} - u_3 a_{62} - \frac{42}{5} u_3 u_2$$

$$- \frac{6}{5} u_3 u_4, u_4 a_{63} + u_3 a_{62} + \frac{42}{5} u_4 u_1 + \frac{6}{5} u_3 u_4, -2 a_{62} a_{19} - 2 a_{63} a_{55} + \frac{6}{5} a_{110} u_2$$

$$- \frac{12}{5} a_{110} u_4, -a_{62} a_{19} + a_{62} a_{46} + \frac{6}{5} a_{110} u_2 - \frac{12}{5} a_{110} u_4, -a_{62} a_{46} + a_{62} a_{19}$$

$$- \frac{6}{5} a_{119} u_1 + \frac{12}{5} a_{119} u_3, -2 a_{62} a_{55} + 2 a_{63} a_{46} - \frac{6}{5} a_{110} u_1 + \frac{12}{5} a_{110} u_3, -2 a_{63} a_{19}$$

$$\begin{aligned}
& + 2 a_{62} a_{55} + \frac{6}{5} a_{119} u_2 - \frac{12}{5} a_{119} u_4, a_{63} a_{19} - a_{63} a_{46} + \frac{6}{5} a_{92} u_2 - \frac{12}{5} a_{92} u_4, \\
& a_{63} a_{46} - a_{63} a_{19} - \frac{6}{5} a_{110} u_1 + \frac{12}{5} a_{110} u_3, 2 a_{63} a_{55} + 2 a_{62} a_{46} - \frac{6}{5} a_{92} u_1 \\
& + \frac{12}{5} a_{92} u_3, -\frac{12}{5} a_{84} u_1 - \frac{6}{5} a_{84} u_3 - a_{119} u_3 + a_{110} u_4, \frac{12}{5} a_{84} u_2 + \frac{6}{5} a_{84} u_4 \\
& - a_{110} u_3 + a_{92} u_4, 6 a_{92} - a_{62} u_2 + a_{63} u_1 + \frac{42}{5} u_2^2 + \frac{6}{5} u_2 u_4, -6 a_{110} + u_2 a_{63} \\
& + u_1 a_{62} + \frac{42}{5} u_2 u_1 + \frac{6}{5} u_4 u_1, 6 a_{110} - u_2 a_{63} - u_1 a_{62} - \frac{42}{5} u_2 u_1 - \frac{6}{5} u_3 u_2, \\
& -6 a_{119} - a_{62} u_2 + a_{63} u_1 - \frac{42}{5} u_1^2 - \frac{6}{5} u_1 u_3, a_{62} u_4 - a_{84} - a_{63} u_3 + \frac{42}{5} u_1 u_3 \\
& + \frac{6}{5} u_3^2, a_{62} u_4 - a_{63} u_3 + a_{84} - \frac{42}{5} u_2 u_4 - \frac{6}{5} u_4^2, \frac{12}{5} u_1 a_{62} + \frac{6}{5} u_3 a_{62} \\
& + \frac{12}{5} u_2 a_{63} + \frac{6}{5} u_4 a_{63} + u_3 u_2 + 2 a_{46}, \frac{12}{5} u_1 a_{62} + \frac{6}{5} u_3 a_{62} + \frac{12}{5} u_2 a_{63} \\
& + \frac{6}{5} u_4 a_{63} + u_4 u_1 + 2 a_{19}, -a_{19} - \frac{6}{5} u_1 a_{62} + \frac{12}{5} u_3 a_{62} - \frac{6}{5} u_2 a_{63} + \frac{12}{5} u_4 a_{63} \\
& - \frac{36}{5} u_2 u_1 + \frac{72}{5} u_4 u_1, -a_{46} - \frac{6}{5} u_1 a_{62} + \frac{12}{5} u_3 a_{62} - \frac{6}{5} u_2 a_{63} + \frac{12}{5} u_4 a_{63} \\
& - \frac{36}{5} u_2 u_1 + \frac{72}{5} u_3 u_2, -a_{55} - \frac{6}{5} a_{63} u_1 + \frac{12}{5} a_{63} u_3 + \frac{6}{5} a_{62} u_2 - \frac{12}{5} a_{62} u_4 \\
& + \frac{36}{5} u_1^2 - \frac{72}{5} u_1 u_3, a_{55} + \frac{6}{5} a_{63} u_1 - \frac{12}{5} a_{63} u_3 - \frac{6}{5} a_{62} u_2 + \frac{12}{5} a_{62} u_4 \\
& + \frac{36}{5} u_2^2 - \frac{72}{5} u_2 u_4, -\frac{12}{5} a_{63} u_1 - \frac{6}{5} a_{63} u_3 + \frac{12}{5} a_{62} u_2 + \frac{6}{5} a_{62} u_4 + u_1 u_3 \\
& - 2 a_{55} + 6 a_{84}, \frac{12}{5} a_{63} u_1 + \frac{6}{5} a_{63} u_3 - \frac{12}{5} a_{62} u_2 - \frac{6}{5} a_{62} u_4 + u_2 u_4 + 2 a_{55} \\
& + 6 a_{84}, -2 a_{62}^2 - 2 a_{63}^2, 2 a_{62}^2 + 2 a_{63}^2, -2 a_{62}^2 - 2 a_{63}^2 - a_{55}, 2 a_{62}^2 + 2 a_{63}^2 - a_{55}, -2 a_{62}^2 \\
& - 2 a_{63}^2 - a_{92}, 2 a_{62}^2 + 2 a_{63}^2 + a_{92}, 2 a_{62}^2 + 2 a_{63}^2 + a_{119}, -2 a_{62}^2 - 2 a_{63}^2 - a_{55} + 6 a_{84}, 2 \\
& a_{62}^2 + 2 a_{63}^2 - a_{55} - 6 a_{84}, -u_1 a_{84} + 2 a_{62} a_{110} - a_{63} a_{92} + a_{63} a_{119}, -u_2 a_{84} + a_{62} a_{92} \\
& - a_{62} a_{119} + 2 a_{63} a_{110}, -6 u_1 a_{62} - u_2 u_3 - 6 u_2 a_{63} + a_{46} - a_{110}, -u_1 u_3 + 6 u_1 a_{63} \\
& - 6 u_2 a_{62} - a_{55} - a_{92}, -u_1 u_4 - 6 u_1 a_{62} - 6 u_2 a_{63} + a_{19} - a_{110}, -6 u_1 a_{63} - u_2 u_4 \\
& + 6 u_2 a_{62} + a_{55} - a_{119}, 6 u_1 a_{110} + 6 u_2 a_{119} - a_{62} a_{92} + a_{62} a_{119} - 2 a_{63} a_{110}, 6 u_1 a_{92} \\
& + 6 u_2 a_{110} - 2 a_{62} a_{110} + a_{63} a_{92} - a_{63} a_{119}\}, [ \ ], [ \ ]
\end{aligned}$$

It's clear that not only does the Jacobi identities imply that  $g$  is decomposable, but moreover the unique solution is flat. Therefore we do not need to consider this case again in the next section.

## Section 2: decomposable $h$ -modules $g$ .

In this section we solve the Jacobi equations for decomposable  $\mathfrak{h}$ -modules  $\mathfrak{g}$ , and compute the Nijenhuis tensor of  $J$  on the resulting homogeneous space.

## Part 2.1: 5D isotropy $\mathfrak{P}$ .

```
> restart:with(DifferentialGeometry): with(Tensor): with(Tools):
  with(LieAlgebras):
```

```
h > dimM:=6;
```

*dimM:=6*

(62)

```
L1 > MrepMat := [Matrix(6, 6, {(1, 1) = 0, (1, 2) = -1, (1, 3) =
0, (1, 4) = 0, (1, 5) = 0, (1, 6) = 0, (2, 1) = 1, (2, 2) =
0, (2, 3) = 0, (2, 4) = 0, (2, 5) = 0, (2, 6) = 0, (3, 1) =
0, (3, 2) = 0, (3, 3) = 0, (3, 4) = -1, (3, 5) = 0, (3, 6)
= 0, (4, 1) = 0, (4, 2) = 0, (4, 3) = 1, (4, 4) = 0, (4, 5)
= 0, (4, 6) = 0, (5, 1) = 0, (5, 2) = 0, (5, 3) = 0, (5, 4)
= 0, (5, 5) = 0, (5, 6) = 2, (6, 1) = 0, (6, 2) = 0, (6, 3)
= 0, (6, 4) = 0, (6, 5) = -2, (6, 6) = 0}), Matrix(6, 6, {
(1, 1) = 1, (1, 2) = 0, (1, 3) = 0, (1, 4) = 0, (1, 5) = 0,
(1, 6) = 0, (2, 1) = 0, (2, 2) = 1, (2, 3) = 0, (2, 4) = 0,
(2, 5) = 0, (2, 6) = 0, (3, 1) = 0, (3, 2) = 0, (3, 3) =
-1, (3, 4) = 0, (3, 5) = 0, (3, 6) = 0, (4, 1) = 0, (4, 2)
= 0, (4, 3) = 0, (4, 4) = -1, (4, 5) = 0, (4, 6) = 0, (5,
1) = 0, (5, 2) = 0, (5, 3) = 0, (5, 4) = 0, (5, 5) = 0, (5,
6) = 0, (6, 1) = 0, (6, 2) = 0, (6, 3) = 0, (6, 4) = 0, (6,
5) = 0, (6, 6) = 0}), Matrix(6, 6, {(1, 1) = 0, (1, 2) = 0,
(1, 3) = 0, (1, 4) = 0, (1, 5) = 0, (1, 6) = 0, (2, 1) = 0,
(2, 2) = 0, (2, 3) = 0, (2, 4) = 0, (2, 5) = 0, (2, 6) = 0,
(3, 1) = 0, (3, 2) = 0, (3, 3) = 0, (3, 4) = 0, (3, 5) = 1,
(3, 6) = 0, (4, 1) = 0, (4, 2) = 0, (4, 3) = 0, (4, 4) = 0,
(4, 5) = 0, (4, 6) = 1, (5, 1) = -1, (5, 2) = 0, (5, 3) =
0, (5, 4) = 0, (5, 5) = 0, (5, 6) = 0, (6, 1) = 0, (6, 2) =
-1, (6, 3) = 0, (6, 4) = 0, (6, 5) = 0, (6, 6) = 0}),
Matrix(6, 6, {(1, 1) = 0, (1, 2) = 0, (1, 3) = 0, (1, 4) =
0, (1, 5) = 0, (1, 6) = 0, (2, 1) = 0, (2, 2) = 0, (2, 3) =
0, (2, 4) = 0, (2, 5) = 0, (2, 6) = 0, (3, 1) = 0, (3, 2) =
0, (3, 3) = 0, (3, 4) = 0, (3, 5) = 0, (3, 6) = -3, (4, 1)
= 0, (4, 2) = 0, (4, 3) = 0, (4, 4) = 0, (4, 5) = 3, (4, 6)
= 0, (5, 1) = 0, (5, 2) = -3, (5, 3) = 0, (5, 4) = 0, (5,
5) = 0, (5, 6) = 0, (6, 1) = 3, (6, 2) = 0, (6, 3) = 0, (6,
4) = 0, (6, 5) = 0, (6, 6) = 0}), Matrix(6, 6, {(1, 1) = 0,
(1, 2) = 0, (1, 3) = 0, (1, 4) = 0, (1, 5) = 0, (1, 6) = 0,
(2, 1) = 0, (2, 2) = 0, (2, 3) = 0, (2, 4) = 0, (2, 5) = 0,
(2, 6) = 0, (3, 1) = 0, (3, 2) = -6, (3, 3) = 0, (3, 4) =
0, (3, 5) = 0, (3, 6) = 0, (4, 1) = 6, (4, 2) = 0, (4, 3) =
0, (4, 4) = 0, (4, 5) = 0, (4, 6) = 0, (5, 1) = 0, (5, 2) =
0, (5, 3) = 0, (5, 4) = 0, (5, 5) = 0, (5, 6) = 0, (6, 1) =
0, (6, 2) = 0, (6, 3) = 0, (6, 4) = 0, (6, 5) = 0, (6, 6) =
0})]:
```

These  $6 \times 6$  matrices give the  $\mathfrak{h}$ -action on  $\mathfrak{m} = \mathfrak{g}/\mathfrak{h}$ . We explicitly build the module  $\mathfrak{g}$  as a direct sum.

```
V > DGsetup([seq(v||i,i=1..dimM)],m);
```

*frame name: m*

(63)

```
V > HData:=LieAlgebraData(MrepMat,h):DGsetup(HData);
                               Lie algebra: h
```

```
h > mrep:=Representation(h,m,MrepMat):
V > rho:=Adjoint(h,representationSpace=h):
L1 > rep:=DirectSumOfRepresentations([rho,mrep],g);
```

$$\begin{aligned} rep := e1 \rightarrow & \begin{bmatrix} 0 & 0 & 0 & 0 & 0 & 0 & 0 & 0 & 0 & 0 & 0 \\ 0 & 0 & 0 & 0 & 0 & 0 & 0 & 0 & 0 & 0 & 0 \\ 0 & 0 & 0 & -9 & 0 & 0 & 0 & 0 & 0 & 0 & 0 \\ 0 & 0 & 1 & 0 & 0 & 0 & 0 & 0 & 0 & 0 & 0 \\ 0 & 0 & 0 & 0 & 0 & 0 & 0 & 0 & 0 & 0 & 0 \\ 0 & 0 & 0 & 0 & 0 & 0 & -1 & 0 & 0 & 0 & 0 \\ 0 & 0 & 0 & 0 & 0 & 1 & 0 & 0 & 0 & 0 & 0 \\ 0 & 0 & 0 & 0 & 0 & 0 & 0 & 0 & -1 & 0 & 0 \\ 0 & 0 & 0 & 0 & 0 & 0 & 0 & 1 & 0 & 0 & 0 \\ 0 & 0 & 0 & 0 & 0 & 0 & 0 & 0 & 0 & 0 & 2 \\ 0 & 0 & 0 & 0 & 0 & 0 & 0 & 0 & 0 & -2 & 0 \end{bmatrix}, e2 \rightarrow \\ & \begin{bmatrix} 0 & 0 & 0 & 0 & 0 & 0 & 0 & 0 & 0 & 0 & 0 \\ 0 & 0 & 0 & 0 & 0 & 0 & 0 & 0 & 0 & 0 & 0 \\ 0 & 0 & -1 & 0 & 0 & 0 & 0 & 0 & 0 & 0 & 0 \\ 0 & 0 & 0 & -1 & 0 & 0 & 0 & 0 & 0 & 0 & 0 \\ 0 & 0 & 0 & 0 & -2 & 0 & 0 & 0 & 0 & 0 & 0 \\ 0 & 0 & 0 & 0 & 0 & 1 & 0 & 0 & 0 & 0 & 0 \\ 0 & 0 & 0 & 0 & 0 & 0 & 1 & 0 & 0 & 0 & 0 \\ 0 & 0 & 0 & 0 & 0 & 0 & 0 & -1 & 0 & 0 & 0 \\ 0 & 0 & 0 & 0 & 0 & 0 & 0 & 0 & -1 & 0 & 0 \\ 0 & 0 & 0 & 0 & 0 & 0 & 0 & 0 & 0 & 0 & 0 \\ 0 & 0 & 0 & 0 & 0 & 0 & 0 & 0 & 0 & 0 & 0 \end{bmatrix}, e3 \rightarrow \end{aligned} \quad (66)$$



$$\begin{bmatrix} 0 & 0 & 0 & 0 & 0 & 0 & 0 & 0 & 0 & 0 & 0 \\ 0 & 0 & 0 & 0 & 0 & 0 & 0 & 0 & 0 & 0 & 0 \\ 0 & 1 & 0 & 0 & 0 & 0 & 0 & 0 & 0 & 0 & 0 \\ -1 & 0 & 0 & 0 & 0 & 0 & 0 & 0 & 0 & 0 & 0 \\ 0 & 0 & 0 & 1 & 0 & 0 & 0 & 0 & 0 & 0 & 0 \\ 0 & 0 & 0 & 0 & 0 & 0 & 0 & 0 & 0 & 0 & 0 \\ 0 & 0 & 0 & 0 & 0 & 0 & 0 & 0 & 0 & 0 & 0 \\ 0 & 0 & 0 & 0 & 0 & 0 & 0 & 0 & 1 & 0 & 0 \\ 0 & 0 & 0 & 0 & 0 & 0 & 0 & 0 & 0 & 1 & 0 \\ 0 & 0 & 0 & 0 & 0 & -1 & 0 & 0 & 0 & 0 & 0 \\ 0 & 0 & 0 & 0 & 0 & 0 & -1 & 0 & 0 & 0 & 0 \end{bmatrix}, e4 \rightarrow \begin{bmatrix} 0 & 0 & 0 & 0 & 0 & 0 & 0 & 0 & 0 & 0 & 0 \\ 0 & 0 & 0 & 0 & 0 & 0 & 0 & 0 & 0 & 0 & 0 \\ 9 & 0 & 0 & 0 & 0 & 0 & 0 & 0 & 0 & 0 & 0 \\ 0 & 1 & 0 & 0 & 0 & 0 & 0 & 0 & 0 & 0 & 0 \\ 0 & 0 & -1 & 0 & 0 & 0 & 0 & 0 & 0 & 0 & 0 \\ 0 & 0 & 0 & 0 & 0 & 0 & 0 & 0 & 0 & 0 & 0 \\ 0 & 0 & 0 & 0 & 0 & 0 & 0 & 0 & 0 & 0 & 0 \\ 0 & 0 & 0 & 0 & 0 & 0 & 0 & 0 & 0 & -3 & 0 \\ 0 & 0 & 0 & 0 & 0 & 0 & 0 & 0 & 3 & 0 & 0 \\ 0 & 0 & 0 & 0 & 0 & 0 & -3 & 0 & 0 & 0 & 0 \\ 0 & 0 & 0 & 0 & 0 & 3 & 0 & 0 & 0 & 0 & 0 \end{bmatrix}$$

$$, e5 \rightarrow \begin{bmatrix} 0 & 0 & 0 & 0 & 0 & 0 & 0 & 0 & 0 & 0 & 0 \\ 0 & 0 & 0 & 0 & 0 & 0 & 0 & 0 & 0 & 0 & 0 \\ 0 & 0 & 0 & 0 & 0 & 0 & 0 & 0 & 0 & 0 & 0 \\ 0 & 0 & 0 & 0 & 0 & 0 & 0 & 0 & 0 & 0 & 0 \\ 0 & 2 & 0 & 0 & 0 & 0 & 0 & 0 & 0 & 0 & 0 \\ 0 & 0 & 0 & 0 & 0 & 0 & 0 & 0 & 0 & 0 & 0 \\ 0 & 0 & 0 & 0 & 0 & 0 & 0 & 0 & 0 & 0 & 0 \\ 0 & 0 & 0 & 0 & 0 & 0 & -6 & 0 & 0 & 0 & 0 \\ 0 & 0 & 0 & 0 & 0 & 6 & 0 & 0 & 0 & 0 & 0 \\ 0 & 0 & 0 & 0 & 0 & 0 & 0 & 0 & 0 & 0 & 0 \\ 0 & 0 & 0 & 0 & 0 & 0 & 0 & 0 & 0 & 0 & 0 \end{bmatrix}$$

Now we have the module  $g$ . The next step is to compute the space of invariant brackets.

**h** > **ChangeFrame(g);**

$h$

(67)

**L1** > **L2m:=GenerateForms([seq(dw| i,i=6..11)],2):L2mtg:=  
GenerateTensors([L2m,[seq(D\_w| i,i=1..11)])]):**

**L1** > **brackets:=Invariants(rep,L2mtg);**

$$\begin{aligned}
\text{brackets} := & \left[ -dw6 \otimes dw8 \otimes \partial_{w11} - dw6 \otimes dw9 \otimes \partial_{w10} + dw6 \otimes dw10 \otimes \partial_{w7} + dw6 \otimes dw11 \right. \\
& \otimes \partial_{w6} - dw7 \otimes dw8 \otimes \partial_{w10} + dw7 \otimes dw9 \otimes \partial_{w11} + dw7 \otimes dw10 \otimes \partial_{w6} - dw7 \otimes dw11 \\
& \otimes \partial_{w7} + dw8 \otimes dw6 \otimes \partial_{w11} + dw8 \otimes dw7 \otimes \partial_{w10} - dw8 \otimes dw10 \otimes \partial_{w9} - dw8 \otimes dw11 \\
& \otimes \partial_{w8} + dw9 \otimes dw6 \otimes \partial_{w10} - dw9 \otimes dw7 \otimes \partial_{w11} - dw9 \otimes dw10 \otimes \partial_{w8} + dw9 \otimes dw11 \\
& \left. \otimes \partial_{w9} - dw10 \otimes dw6 \otimes \partial_{w7} - dw10 \otimes dw7 \otimes \partial_{w6} + dw10 \otimes dw8 \otimes \partial_{w9} + dw10 \otimes dw9 \right]
\end{aligned}$$

(68)

$$\begin{aligned}
& \otimes \partial_{w8} - dw11 \otimes dw6 \otimes \partial_{w6} + dw11 \otimes dw7 \otimes \partial_{w7} + dw11 \otimes dw8 \otimes \partial_{w8} - dw11 \otimes dw9 \\
& \otimes \partial_{w9} - dw6 \otimes dw8 \otimes \partial_{w10} + dw6 \otimes dw9 \otimes \partial_{w11} + dw6 \otimes dw10 \otimes \partial_{w6} - dw6 \otimes dw11 \\
& \otimes \partial_{w7} + dw7 \otimes dw8 \otimes \partial_{w11} + dw7 \otimes dw9 \otimes \partial_{w10} - dw7 \otimes dw10 \otimes \partial_{w7} - dw7 \otimes dw11 \\
& \otimes \partial_{w6} + dw8 \otimes dw6 \otimes \partial_{w10} - dw8 \otimes dw7 \otimes \partial_{w11} - dw8 \otimes dw10 \otimes \partial_{w8} + dw8 \otimes dw11 \\
& \otimes \partial_{w9} - dw9 \otimes dw6 \otimes \partial_{w11} - dw9 \otimes dw7 \otimes \partial_{w10} + dw9 \otimes dw10 \otimes \partial_{w9} + dw9 \otimes dw11 \\
& \otimes \partial_{w8} - dw10 \otimes dw6 \otimes \partial_{w6} + dw10 \otimes dw7 \otimes \partial_{w7} + dw10 \otimes dw8 \otimes \partial_{w8} - dw10 \otimes dw9 \\
& \otimes \partial_{w9} + dw11 \otimes dw6 \otimes \partial_{w7} + dw11 \otimes dw7 \otimes \partial_{w6} - dw11 \otimes dw8 \otimes \partial_{w9} - dw11 \otimes dw9 \\
& \otimes \partial_{w8} ]
\end{aligned}$$

```
g > nops(brackets);
```

2

(69)

Since the space of invariant brackets is 2D, we know that it is precisely the J-complex span of the h-invariant algebraic Nijenhuis tensor (which takes values in m). Thus if this case satisfies the Jacobi identity, all other isotropies will also have the same solution. Moreover, this tensor is J-antilinear, and so will induce itself as the Nijenhuis tensor of J if it can be realized as a homogeneous space.

```
g > bracket:=evalDG(add(a||i*brackets[i],i=1..nops(brackets))):
g > repMat:=seq(ApplyRepresentation(rep,e||i),i=1..5):
g > ChangeFrame(g);
```

h

(70)

```
V80 > HTensor:=seq(convert(repMat[i],DGtensor,[[ "con_bas",
"cov_bas"],[]]),i=1..nops(repMat)):
V > A:=(x,y,z)->GetComponents(evalDG(ContractIndices(HTensor[x],
HTensor[y],[[2,1]])&minus ContractIndices(HTensor[y],HTensor
[x],[[2,1]])),HTensor)[z]:
V > B:=(x,y,z)->GetComponents(convert(evalDG(ContractIndices
(HTensor[x],D_w||y,[[2,1]])),DGvector),DGinfo(g,
"FrameBaseVectors"))[z]:
g > C:=(x,y,z)->GetComponents(convert(ContractIndices( evalDG
(D_w||x &t D_w||y), bracket,[[1,1],[2,2]]),DGvector),DGinfo
(g,"FrameBaseVectors"))[z]:
V > CH:=seq(seq([q||i,q||j]=add(A(i,j,k)*q||k,k=1..nops(repMat)
),i=j+1..nops(repMat)),j=1..nops(repMat)):
L2 > ChangeFrame(g);
```

g

(71)

```
V > CHM:=seq(seq([q||i,q||j]=add(B(i,j,k)*q||k,k=1..11),i=1..
nops(repMat)),j=6..11):
g > CM:=seq(seq([q||i,q||j]=add(C(i,j,k)*q||k,k=1..11),j=i+1.
.11),i=5..11):
V > KData:=LieAlgebraData([op(CH),op(CHM),op(CM)],seq(q||i,i=1..
nops(repMat)+dimM));
KData := [e1,e2]=0, [e1,e3]=e4, [e1,e4]=-9 e3, [e1,e5]=0, [e1,e6]=e7, [e1,e7]=
-e6, [e1,e8]=e9, [e1,e9]=-e8, [e1,e10]=-2 e11, [e1,e11]=2 e10, [e2,e3]=
-e3, [e2,e4]=-e4, [e2,e5]=-2 e5, [e2,e6]=e6, [e2,e7]=e7, [e2,e8]=-e8, [e2,
```

(72)

$e9] = -e9$ ,  $[e2, e10] = 0$ ,  $[e2, e11] = 0$ ,  $[e3, e4] = e5$ ,  $[e3, e5] = 0$ ,  $[e3, e6] = -e10$ ,  $[e3, e7] = -e11$ ,  $[e3, e8] = 0$ ,  $[e3, e9] = 0$ ,  $[e3, e10] = e8$ ,  $[e3, e11] = e9$ ,  $[e4, e5] = 0$ ,  $[e4, e6] = 3e11$ ,  $[e4, e7] = -3e10$ ,  $[e4, e8] = 0$ ,  $[e4, e9] = 0$ ,  $[e4, e10] = 3e9$ ,  $[e4, e11] = -3e8$ ,  $[e5, e6] = 6e9$ ,  $[e5, e7] = -6e8$ ,  $[e5, e8] = 0$ ,  $[e5, e9] = 0$ ,  $[e5, e10] = 0$ ,  $[e5, e11] = 0$ ,  $[e6, e7] = 0$ ,  $[e6, e8] = -a2e10 - a1e11$ ,  $[e6, e9] = -a1e10 + a2e11$ ,  $[e6, e10] = a2e6 + a1e7$ ,  $[e6, e11] = a1e6 - a2e7$ ,  $[e7, e8] = -a1e10 + a2e11$ ,  $[e7, e9] = a2e10 + a1e11$ ,  $[e7, e10] = a1e6 - a2e7$ ,  $[e7, e11] = -a2e6 - a1e7$ ,  $[e8, e9] = 0$ ,  $[e8, e10] = -a2e8 - a1e9$ ,  $[e8, e11] = -a1e8 + a2e9$ ,  $[e9, e10] = -a1e8 + a2e9$ ,  $[e9, e11] = a2e8 + a1e9$ ,  $[e10, e11] = 0$

These are the most general structure constants for  $\mathfrak{g}$ . Now we check the Jacobi identity.

```
L1 > DGsetup(KData);
```

*Lie algebra: L1*

(73)

```
L1 > Query({a1,a2},"Jacobi")[2];
```

$\{0, -2a1^2 - 2a2^2, 2a1^2 + 2a2^2\}$

(74)

It's clear that all non-flat solutions to the Jacobi equations are non-real.

## Part 2.2: 4D isotropy $\mathfrak{R}$ .

```
> restart:with(DifferentialGeometry): with(Tensor): with(Tools):
with(LieAlgebras):
```

```
h > dimM:=6;
```

*dimM:=6*

(75)

```
g > MrepMat := [Matrix(6, 6, {(1, 1) = u2, (1, 2) = -u1, (1, 3) = 0, (1, 4) = 0, (1, 5) = 0, (1, 6) = 0, (2, 1) = u1, (2, 2) = u2, (2, 3) = 0, (2, 4) = 0, (2, 5) = 0, (2, 6) = 0, (3, 1) = 0, (3, 2) = 0, (3, 3) = -u2, (3, 4) = -u1, (3, 5) = 0, (3, 6) = 0, (4, 1) = 0, (4, 2) = 0, (4, 3) = u1, (4, 4) = -u2, (4, 5) = 0, (4, 6) = 0, (5, 1) = 0, (5, 2) = 0, (5, 3) = 0, (5, 4) = 0, (5, 5) = 0, (5, 6) = 2*u1, (6, 1) = 0, (6, 2) = 0, (6, 3) = 0, (6, 4) = 0, (6, 5) = -2*u1, (6, 6) = 0}), Matrix(6, 6, {(1, 1) = 0, (1, 2) = 0, (1, 3) = 0, (1, 4) = 0, (1, 5) = 0, (1, 6) = 0, (2, 1) = 0, (2, 2) = 0, (2, 3) = 0, (2, 4) = 0, (2, 5) = 0, (2, 6) = 0, (3, 1) = 0, (3, 2) = 0, (3, 3) = 0, (3, 4) = 0, (3, 5) = 1, (3, 6) = 0, (4, 1) = 0, (4, 2) = 0, (4, 3) = 0, (4, 4) = 0, (4, 5) = 0, (4, 6) = 1, (5, 1) = -1, (5, 2) = 0, (5, 3) = 0, (5, 4) = 0, (5, 5) = 0, (5, 6) = 0, (6, 1) = 0, (6, 2) = -1, (6, 3) = 0, (6, 4) = 0, (6, 5) = 0, (6, 6) = 0}), Matrix(6, 6, {(1, 1) = 0, (1, 2) = 0, (1, 3) = 0, (1, 4) = 0, (1, 5) = 0, (1, 6) = 0, (2, 1) = 0, (2, 2) = 0, (2, 3) = 0, (2, 4) = 0, (2, 5) = 0, (2, 6) = 0, (3, 1) = 0, (3, 2) = 0, (3, 3) = 0, (3, 4) = 0, (3, 5) = 0, (3, 6) = -3, (4, 1) = 0, (4, 2) = 0, (4, 3) = 0, (4, 4) = 0, (4, 5) = 3, (4, 6) = 0, (5, 1) = 0, (5, 2) = -3, (5, 3) = 0, (5, 4) = 0, (5, 5) = 0, (5, 6) = 0, (6, 1) = 3, (6, 2) = 0, (6, 3) = 0, (6, 4) = 0, (6, 5) = 0, (6, 6) = 0}), Matrix(6, 6, {(1, 1) = 0, (1, 2) = 0, (1, 3) = 0, (1, 4) = 0, (1, 5) = 0, (1, 6) = 0, (2, 1) = 0, (2, 2) = 0, (2, 3) = 0, (2, 4) = 0, (2, 5) = 0, (2, 6) = 0, (3, 1) = 0, (3, 2) = 0, (3, 3) = 0, (3, 4) = 0, (3, 5) = 0, (3, 6) = 0, (4, 1) = 0, (4, 2) = 0, (4, 3) = 0, (4, 4) = 0, (4, 5) = 0, (4, 6) = 0, (5, 1) = 0, (5, 2) = 0, (5, 3) = 0, (5, 4) = 0, (5, 5) = 0, (5, 6) = 0, (6, 1) = 0, (6, 2) = 0, (6, 3) = 0, (6, 4) = 0, (6, 5) = 0, (6, 6) = 0})]
```

```

0, (1, 6) = 0, (2, 1) = 0, (2, 2) = 0, (2, 3) = 0, (2, 4) =
0, (2, 5) = 0, (2, 6) = 0, (3, 1) = 0, (3, 2) = -6, (3, 3) =
0, (3, 4) = 0, (3, 5) = 0, (3, 6) = 0, (4, 1) = 6, (4, 2) =
0, (4, 3) = 0, (4, 4) = 0, (4, 5) = 0, (4, 6) = 0, (5, 1) =
0, (5, 2) = 0, (5, 3) = 0, (5, 4) = 0, (5, 5) = 0, (5, 6) =
0, (6, 1) = 0, (6, 2) = 0, (6, 3) = 0, (6, 4) = 0, (6, 5) =
0, (6, 6) = 0}));

```

$$MrepMat := \begin{bmatrix} u2 & -u1 & 0 & 0 & 0 & 0 \\ u1 & u2 & 0 & 0 & 0 & 0 \\ 0 & 0 & -u2 & -u1 & 0 & 0 \\ 0 & 0 & u1 & -u2 & 0 & 0 \\ 0 & 0 & 0 & 0 & 0 & 2u1 \\ 0 & 0 & 0 & 0 & -2u1 & 0 \end{bmatrix}, \begin{bmatrix} 0 & 0 & 0 & 0 & 0 & 0 \\ 0 & 0 & 0 & 0 & 0 & 0 \\ 0 & 0 & 0 & 0 & 1 & 0 \\ 0 & 0 & 0 & 0 & 0 & 1 \\ -1 & 0 & 0 & 0 & 0 & 0 \\ 0 & -1 & 0 & 0 & 0 & 0 \end{bmatrix},$$

$$\begin{bmatrix} 0 & 0 & 0 & 0 & 0 & 0 \\ 0 & 0 & 0 & 0 & 0 & 0 \\ 0 & 0 & 0 & 0 & 0 & -3 \\ 0 & 0 & 0 & 0 & 3 & 0 \\ 0 & -3 & 0 & 0 & 0 & 0 \\ 3 & 0 & 0 & 0 & 0 & 0 \end{bmatrix}, \begin{bmatrix} 0 & 0 & 0 & 0 & 0 & 0 \\ 0 & 0 & 0 & 0 & 0 & 0 \\ 0 & -6 & 0 & 0 & 0 & 0 \\ 6 & 0 & 0 & 0 & 0 & 0 \\ 0 & 0 & 0 & 0 & 0 & 0 \\ 0 & 0 & 0 & 0 & 0 & 0 \end{bmatrix}$$

R is a one-parameter family of subalgebras of P. We parametrize them in terms of two parameters u1, u2, as this is easier to work with.

```

V > DGsetup([seq(v|i,i=1..dimM)],m);
frame name: m

```

```

m > DGsetup([seq(w|i,i=1..10)],g);
frame name: g

```

```

V > HData:=LieAlgebraData(MrepMat,h):DGsetup(HData);
Lie algebra: h

```

```

h > mrep:=Representation(h,m,MrepMat):

```

```

V > rho:=Adjoint(h,representationspace=h):

```

```

L1 > rep:=DirectSumOfRepresentations([rho,mrep],g):

```

Since there are parameters in the representation, the full system of equations for the invariant brackets is non-linear. Therefore we only solve those equations that are linear before going to the Jacobi identity.

```

h > ChangeFrame(g);
h

```

```

L1 > L2m:=GenerateForms([seq(dw|i,i=5..10)],2):L2mtg:=
GenerateTensors([L2m,[seq(D_w|i,i=1..10)]]):

```

```

g > G:=DGinfo(rep, "ObjectAttributes")[2,1,1]:conbasG:=DGinfo(G,
"FrameBaseVectors"):nG:=DGinfo(G, "LieAlgebraDimension")
:bracket_elements[0]:=evalDG(add(a[i]*L2mtg[i],i=1..nops
(L2mtg))):

```

```

g > image_elements[1]:=ApplyRepresentation(rep,conbasG[2],
bracket_elements[1-1]):
g > image_coefficients[1]:=DGinfo(image_elements[1],
"CoefficientSet")[1..30];
image_coefficients1 := {a11, a15, a16, a61, a65, a66, a91, a93, a95, a96, a99, a100, a101, a103, a105,
a106, a109, a110, a111, a115, a116, a121, a125, a126, a131, a133, a135, a136, a139, a140}
g > kernel_equations[1]:=solve(image_coefficients[1]):nops(%);
30
g > bracket_elements[1]:=DGsimplify(subs(kernel_equations[1],
bracket_elements[1-1])):

```

(81)

(82)

```

g > image_elements[2]:=ApplyRepresentation(rep,conbasG[2],
bracket_elements[2-1]):
g > image_coefficients[2]:=DGinfo(image_elements[2],
"CoefficientSet")[1..128];
image_coefficients2 := {a92, a102, a132, -a92, -a102, -a132, -a33 + a14, a33 - a14, -a35 - a19, a35
+ a19, -a36 - a20, a36 + a20, -a39 + a17, a39 - a17, -a40 + a18, a40 - a18, -a41 + a71,
-a45 + a75, -a46 + a76, -a71 + a41, -a75 + a45, -a76 + a46, -a83 + a64, a83 - a64, -a85
-a69, a85 + a69, -a86 - a70, a86 + a70, -a89 + a67, a89 - a67, -a90 + a68, a90 - a68, -a104
+ a13, a104 - a13, -a107 + a19, a107 - a19, -a108 + a20, a108 - a20, -a113 + a94, a113 - a94,
-a114 + a53, a114 - a53, -a117 + a59, a117 - a59, -a118 + a60, a118 - a60, -a119 - a55, -a119
+ a97, a119 + a55, a119 - a97, -a120 - a56, -a120 + a98, a120 + a56, a120 - a98, -a123 - a94,
a123 + a94, -a124 + a23, a124 - a23, -a127 + a29, a127 - a29, -a128 + a30, a128 - a30, -a129
-a25, -a129 - a97, a129 + a25, a129 + a97, -a130 - a26, -a130 - a98, a130 + a26, a130 + a98,
-a134 + a63, a134 - a63, -a137 + a69, a137 - a69, -a138 + a70, a138 - a70, -a141 + a21, -a141
-a51, a141 - a21, a141 + a51, -a145 + a25, -a145 - a55, a145 - a25, a145 + a55, -a146 + a26,
-a146 - a56, a146 - a26, a146 + a56, -a44 + a74 - a3, -a47 + a77 - a9, -a48 + a78 - a10,
-a49 + a79 + a5, -a50 + a80 + a6, -a74 + a44 + a3, -a77 + a47 + a9, -a78 + a48 + a10,
-a79 + a49 - a5, -a80 + a50 - a6, -a143 + a114 - a124, a143 + a124 - a114, -a144 - a43
+ a24, -a144 + a73 - a54, a144 + a43 - a24, a144 - a73 + a54, -a145 + a129 - a119, a145
+ a119 - a129, -a146 + a130 - a120, a146 + a120 - a130, -a147 - a49 + a27, -a147 + a79
-a57, a147 + a49 - a27, a147 - a79 + a57, -a148 - a50 + a28, -a148 + a80 - a58, a148 + a50
-a28, a148 - a80 + a58, -a149 + a45 + a29, -a149 - a75 - a59, -a149 + a117 - a127, a149
-a45 - a29, a149 + a75 + a59, a149 + a127 - a117, -a150 + a46 + a30, -a150 - a76 - a60,
-a150 + a118 - a128, a150 - a46 - a30, a150 + a76 + a60, a150 + a128 - a118}
g > kernel_equations[2]:=solve(image_coefficients[2]):nops(%);
96
g > bracket_elements[2]:=DGsimplify(subs(kernel_equations[2],
bracket_elements[2-1])):

```

(84)

```

g > image_elements[3]:=ApplyRepresentation(rep,conbasG[3],
bracket_elements[3-1]):
g > image_coefficients[3]:=DGinfo(image_elements[3],
"CoefficientSet")[1..2];
image_coefficients3 := {a112, a122}

```

(85)

```

g > kernel_equations[3]:=solve(image_coefficients[3]):nops(%);
2

```

(86)

```

g > bracket_elements[3]:=DGsimplify(subs(kernel_equations[3],
bracket_elements[3-1])):

```

```

g > image_elements[4]:=ApplyRepresentation(rep,conbasG[3],
bracket_elements[4-1]):
g > image_coefficients[4]:=DGinfo(image_elements[4],
"CoefficientSet")[7..56];
image_coefficients4 := {-3 a19 - 3 a128, 3 a19 + 3 a69, 3 a20 + 3 a70, 3 a20 - 3 a127, -3 a31

```

(87)

```

- 3 a81, -a32 - 3 a43, a32 + 3 a43, -3 a39 + 3 a50, 3 a39 - 3 a50, -3 a40 - 3 a49, -a42
+ 3 a33, a42 - 3 a33, 3 a49 + 3 a40, -3 a69 - 3 a19, 3 a69 - 3 a128, -3 a70 - 3 a20, 3 a70
+ 3 a127, -a72 - 3 a83, a72 + 3 a83, -3 a79 + 3 a90, 3 a79 - 3 a90, -3 a80 - 3 a89, 3 a81
+ 3 a31, -a82 + 3 a73, a82 - 3 a73, 3 a89 + 3 a80, -3 a104 - a52, 3 a104 + a52, -3 a114
+ a12, 3 a114 - a12, -3 a124 - a62, 3 a124 + a62, -3 a127 - 3 a70, 3 a127 - 3 a20, 3 a128
+ 3 a19, 3 a128 - 3 a69, -3 a134 + a22, 3 a134 - a22, -3 a34 - 3 a84 + a2, 3 a84 + 3 a34
- a2, -a142 - 3 a104 - 3 a134, a142 + 3 a134 + 3 a104, -3 a37 - 3 a87 + 3 a78 - 3 a48,
-3 a38 - 3 a88 - 3 a77 + 3 a47, -3 a39 - 3 a89 + 3 a50 - 3 a80, -3 a40 - 3 a90 - 3 a49
+ 3 a79, 3 a87 + 3 a37 + 3 a48 - 3 a78, 3 a88 + 3 a38 - 3 a47 + 3 a77, 3 a89 + 3 a39 + 3 a80
- 3 a50, 3 a90 + 3 a40 - 3 a79 + 3 a49}

```

```

g > kernel_equations[4]:=solve(image_coefficients[4]):nops(%);
44

```

(88)

```

g > bracket_elements[4]:=DGsimplify(subs(kernel_equations[4],
bracket_elements[4-1])):

```

```

g > image_elements[5]:=ApplyRepresentation(rep,conbasG[4],
bracket_elements[5-1]):
g > image_coefficients[5]:={op(DGinfo(image_elements[5],
"CoefficientSet")[5..8]),op(DGinfo(image_elements[5],
"CoefficientSet")[1..2])};

```

```

image_coefficients5 := {-6 a94, 6 a94, -6 a12 + 18 a124, -6 a104 - 6 a134, -18 a124 + 6 a12,
6 a134 + 6 a104}

```

(89)

```

g > kernel_equations[5]:=solve(image_coefficients[5]):nops(%);
5

```

(90)

```

g > bracket_elements[5]:=DGsimplify(subs(kernel_equations[5],
bracket_elements[5-1])):

```

```

g > image_elements[6]:=ApplyRepresentation(rep,conbasG[4],

```

```

    bracket_elements[6-1]):
g > image_coefficients[6]:=DGinfo(image_elements[6],
    "CoefficientSet");
image_coefficients6 := { -2 u2 a141, 2 u2 a141, -2 u2 a31 + 6 a124, 2 u2 a31 - 6 a124, -2 u2 a71
    + 6 a134, 2 u2 a71 - 6 a134, -2 u2 a1 - 2 a42 - 6 a83, 2 u2 a1 + 2 a42 + 6 a83 }

```

(91)

We check all further equations for invariant brackets, and note that they are non-linear. Thus the 5th solution set goes into Jacobi.

```

g > bracket:=bracket_elements[5]:
g > DGinfo(bracket,"CoefficientSet")[1..32];
{a1, a2, a4, a7, a8, a31, a34, a37, a38, a39, a42, a43, a44, a47, a48, a49, a69, a71, a74, a82, a83, a87, a88,
    a89, a90, a124, a127, a134, a141, a144, a147, a148}

```

(92)

There are still 32 parameters.

```

g > repMat:=seq(ApplyRepresentation(rep,e||i),i=1..4):
g > ChangeFrame(g);

```

*h*

(93)

```

V80 > HTensor:=seq(convert(repMat[i],DGtensor,[["con_bas",
    "cov_bas"],[]]),i=1..nops(repMat)):
V > A:=(x,y,z)->GetComponents(evalDG(ContractIndices(HTensor[x],
    HTensor[y],[[2,1]])&minus ContractIndices(HTensor[y],HTensor
    [x],[[2,1]])),HTensor)[z]:
V > B:=(x,y,z)->GetComponents(convert(evalDG(ContractIndices
    (HTensor[x],D_w||y,[[2,1]])),DGvector),DGinfo(g,
    "FrameBaseVectors"))[z]:
g > C:=(x,y,z)->GetComponents(convert(ContractIndices( evalDG
    (D_w||x &t D_w||y), bracket,[[1,1],[2,2]]),DGvector),DGinfo
    (g,"FrameBaseVectors"))[z]:
V > CH:=seq(seq([q||i,q||j]=add(A(i,j,k)*q||k,k=1..nops(MrepMat)
    ),i=j+1..nops(MrepMat)),j=1..nops(MrepMat)):
L2 > ChangeFrame(g);

```

*g*

(94)

```

V > CHM:=seq(seq([q||i,q||j]=add(B(i,j,k)*q||k,k=1..10),i=1..
    nops(MrepMat)),j=5..10):
g > CM:=seq(seq([q||i,q||j]=add(C(i,j,k)*q||k,k=1..10),j=i+1.
    .10),i=5..10):
V > KData:=LieAlgebraData([op(CH),op(CHM),op(CM)],seq(q||i,i=1..
    nops(MrepMat)+dimM));
KData := [e1, e2] = -u2 e2 + u1 e3, [e1, e3] = -9 u1 e2 - u2 e3, [e1, e4] = -2 u2 e4, [e1,
    e5] = u2 e5 + u1 e6, [e1, e6] = -u1 e5 + u2 e6, [e1, e7] = -u2 e7 + u1 e8, [e1, e8] =
    -u1 e7 - u2 e8, [e1, e9] = -2 u1 e10, [e1, e10] = 2 u1 e9, [e2, e3] = e4, [e2, e4] = 0,
    [e2, e5] = -e9, [e2, e6] = -e10, [e2, e7] = 0, [e2, e8] = 0, [e2, e9] = e7, [e2, e10] = e8,
    [e3, e4] = 0, [e3, e5] = 3 e10, [e3, e6] = -3 e9, [e3, e7] = 0, [e3, e8] = 0, [e3, e9] = 3 e8,
    [e3, e10] = -3 e7, [e4, e5] = 6 e8, [e4, e6] = -6 e7, [e4, e7] = 0, [e4, e8] = 0, [e4, e9
    ] = 0, [e4, e10] = 0, [e5, e6] = a1 e1 + a2 e2 - (-a74 + a44) e3 + a4 e4 + (-a90 + a49) e5 +

```

(95)

$$\begin{aligned}
& (a_{89} + a_{39}) e6 + a_7 e7 + a_8 e8 - (a_{88} + a_{38}) e9 + (a_{87} + a_{37}) e10, [e5, e7] = 3 a_{124} e2 \\
& - a_{134} e3 + \frac{a_{42}}{3} e4 + a_{39} e7 - a_{49} e8 - a_{69} e9 + a_{127} e10, [e5, e8] = a_{141} e1 + 3 a_{134} e2 \\
& + a_{124} e3 + (a_{144} + a_{43}) e4 + (a_{147} + a_{49}) e7 + (a_{148} + a_{39}) e8 + a_{127} e9 + a_{69} e10, [e5, e9] \\
& = a_{31} e1 - 3 a_{43} e2 + \frac{a_{42}}{3} e3 + a_{34} e4 + a_{69} e5 - a_{127} e6 + a_{37} e7 + a_{38} e8 + a_{39} e9 \\
& - a_{49} e10, [e5, e10] = a_{71} e1 + a_{42} e2 + a_{43} e3 + a_{44} e4 - a_{127} e5 - a_{69} e6 + a_{47} e7 \\
& + a_{48} e8 + a_{49} e9 + a_{39} e10, [e6, e7] = -a_{141} e1 + 3 a_{134} e2 + a_{124} e3 + \left(-a_{144} + \frac{a_{82}}{3}\right. \\
& \left.) e4 + \left(-a_{147} + a_{90}\right) e7 - \left(a_{148} + a_{89}\right) e8 + a_{127} e9 + a_{69} e10, [e6, e8] = -3 a_{124} e2 \\
& + a_{134} e3 + a_{83} e4 + a_{89} e7 + a_{90} e8 + a_{69} e9 - a_{127} e10, [e6, e9] = a_{71} e1 - 3 a_{83} e2 \\
& + \frac{a_{82}}{3} e3 + a_{74} e4 - a_{127} e5 - a_{69} e6 - \left(a_{88} + a_{38} - a_{47}\right) e7 + \left(a_{87} + a_{37} + a_{48}\right) e8 \\
& + a_{90} e9 - a_{89} e10, [e6, e10] = -a_{31} e1 + a_{82} e2 + a_{83} e3 + \left(\frac{a_2}{3} - a_{34}\right) e4 - a_{69} e5 \\
& + a_{127} e6 + a_{87} e7 + a_{88} e8 + a_{89} e9 + a_{90} e10, [e7, e8] = 0, [e7, e9] = -a_{134} e4 - a_{69} e7 \\
& + a_{127} e8, [e7, e10] = a_{124} e4 + a_{127} e7 + a_{69} e8, [e8, e9] = a_{124} e4 + a_{127} e7 + a_{69} e8, \\
& [e8, e10] = a_{134} e4 + a_{69} e7 - a_{127} e8, [e9, e10] = a_{141} e1 + a_{144} e4 + a_{147} e7 + a_{148} e8
\end{aligned}$$

These are the most general structure constants for g.

```
g > DGsetup(KData);
```

*Lie algebra: Ll*

(96)

```
g > jaceq:=Query({u1,u2,seq(a[i],i=1..300)},"Jacobi");
```

We may assume either u1=1 or u2=1.

```
g > use RealDomain in jacsol1:=solve(subs({u1=1},jaceq[2])); end;
jacsol1 := {u2=0, a1=0, a2=0, a4=a4, a7=0, a8=0, a31=0, a34=0, a37=a37, a38=a47, a39
=0, a42=0, a43=0, a44=0, a47=a47, a48=-a37, a49=0, a69=0, a71=0, a74=0, a82=0,
a83=0, a87=-a37, a88=-a47, a89=0, a90=0, a124=0, a127=0, a134=0, a141=0, a144=0,
a147=0, a148=0}
```

(97)

```
Ll > use RealDomain in jacsol2:=solve(subs({u2=1},jaceq[2]));
end;
```

*jacsol2 :=*

(98)

```
g > KData2:=subs({u1=1,op(jacsol1)},KData);
```

```
KData2 := [e1, e2]=e3, [e1, e3]=-9 e2, [e1, e4]=0, [e1, e5]=e6, [e1, e6]=-e5, [e1, e7
```

(99)



```

] = e8, [e1, e8] = -e7, [e1, e9] = -2 e10, [e1, e10] = 2 e9, [e2, e3] = e4, [e2, e4] = 0,
[e2, e5] = -e9, [e2, e6] = -e10, [e2, e7] = 0, [e2, e8] = 0, [e2, e9] = e7, [e2, e10] = e8,
[e3, e4] = 0, [e3, e5] = 3 e10, [e3, e6] = -3 e9, [e3, e7] = 0, [e3, e8] = 0, [e3, e9] = 3 e8,
[e3, e10] = -3 e7, [e4, e5] = 6 e8, [e4, e6] = -6 e7, [e4, e7] = 0, [e4, e8] = 0, [e4, e9]
] = 0, [e4, e10] = 0, [e5, e6] = a4 e4, [e5, e7] = 0, [e5, e8] = 0, [e5, e9] = a37 e7 + a47 e8,
[e5, e10] = a47 e7 - a37 e8, [e6, e7] = 0, [e6, e8] = 0, [e6, e9] = a47 e7 - a37 e8, [e6, e10]
] = -a37 e7 - a47 e8, [e7, e8] = 0, [e7, e9] = 0, [e7, e10] = 0, [e8, e9] = 0, [e8, e10] = 0,
[e9, e10] = 0

```

```
g > DGsetup(KData2);
```

*Lie algebra: L1*

(100)

```
g > Query("Jacobi");
```

*true*

(101)

We compute the Nijenhuis tensor by the Frolicher-Nijenhuis tensor bracket.

```
h > Jtensor:=evalDG(e5 &t theta6 - e6 &t theta5 + e7 &t theta8 -
e8 &t theta7 + e9 &t theta10 -e10 &t theta9);
```

*Jtensor := e5 ⊗ θ6 - e6 ⊗ θ5 + e7 ⊗ θ8 - e8 ⊗ θ7 + e9 ⊗ θ10 - e10 ⊗ θ9*

(102)

```
L1 > Pm:=evalDG(add(e|i &t theta|i,i=5..10));
```

*Pm := e5 ⊗ θ5 + e6 ⊗ θ6 + e7 ⊗ θ7 + e8 ⊗ θ8 + e9 ⊗ θ9 + e10 ⊗ θ10*

(103)

```
g > NJ:=TensorBrackets(Jtensor,Jtensor,"Frolicher-Nijenhuis");
```

```
g > DGImageSpace(x->ContractIndices(evalDG(Pm &t x),NJ,[[2,1],[3,
2],[4,3]]),GenerateTensors([[e5,e6,e7,e8,e9,e10],[e5,e6,e7,
e8,e9,e10]]));
```

*[ -8 a37 e7 - 8 a47 e8, -8 a47 e7 + 8 a37 e8 ]*

(104)

It's clear that the Nijenhuis tensor is degenerate, as its image is at most 2D.

### Part 2.3: 3D isotropy L2

```
> restart:with(DifferentialGeometry): with(Tensor): with(Tools):
with(LieAlgebras):
```

```
h > dimM:=6;
```

*dimM := 6*

(105)

```
g > MrepMat := [Matrix(6, 6, {(1, 1) = 0, (1, 2) = -1, (1, 3) =
0, (1, 4) = 0, (1, 5) = 0, (1, 6) = 0, (2, 1) = 1, (2, 2) =
0, (2, 3) = 0, (2, 4) = 0, (2, 5) = 0, (2, 6) = 0, (3, 1) =
0, (3, 2) = 0, (3, 3) = 0, (3, 4) = -1, (3, 5) = 0, (3, 6) =
0, (4, 1) = 0, (4, 2) = 0, (4, 3) = 1, (4, 4) = 0, (4, 5) =
0, (4, 6) = 0, (5, 1) = 0, (5, 2) = 0, (5, 3) = 0, (5, 4) =
0, (5, 5) = 0, (5, 6) = 2, (6, 1) = 0, (6, 2) = 0, (6, 3) =
0, (6, 4) = 0, (6, 5) = -2, (6, 6) = 0}), Matrix(6, 6, {(1,
1) = 1, (1, 2) = 0, (1, 3) = 0, (1, 4) = 0, (1, 5) = 0, (1,
6) = 0, (2, 1) = 0, (2, 2) = 1, (2, 3) = 0, (2, 4) = 0, (2,
5) = 0, (2, 6) = 0, (3, 1) = 0, (3, 2) = 0, (3, 3) = -1, (3,
4) = 0, (3, 5) = 0, (3, 6) = 0, (4, 1) = 0, (4, 2) = 0, (4,
```

```
3) = 0, (4, 4) = -1, (4, 5) = 0, (4, 6) = 0, (5, 1) = 0, (5,
2) = 0, (5, 3) = 0, (5, 4) = 0, (5, 5) = 0, (5, 6) = 0, (6,
1) = 0, (6, 2) = 0, (6, 3) = 0, (6, 4) = 0, (6, 5) = 0, (6,
6) = 0}}, Matrix(6, 6, {(1, 1) = 0, (1, 2) = 0, (1, 3) = 0,
(1, 4) = 0, (1, 5) = 0, (1, 6) = 0, (2, 1) = 0, (2, 2) = 0,
(2, 3) = 0, (2, 4) = 0, (2, 5) = 0, (2, 6) = 0, (3, 1) = 0,
(3, 2) = -6, (3, 3) = 0, (3, 4) = 0, (3, 5) = 0, (3, 6) = 0,
(4, 1) = 6, (4, 2) = 0, (4, 3) = 0, (4, 4) = 0, (4, 5) = 0,
(4, 6) = 0, (5, 1) = 0, (5, 2) = 0, (5, 3) = 0, (5, 4) = 0,
(5, 5) = 0, (5, 6) = 0, (6, 1) = 0, (6, 2) = 0, (6, 3) = 0,
(6, 4) = 0, (6, 5) = 0, (6, 6) = 0}]]:
```

Since there are no parameters in the Lie algebra or representation, this case is quite straightforward.

$$\mathbf{V} \rightarrow \text{DGsetup}([\text{seq}(\mathbf{v} \mid i, i=1..\dim \mathbf{M})], m);$$

(106)

$$\mathbf{m} > \text{DGsetup}([\text{seq}(\mathbf{w} \mid i, i=1..9)], g);$$

(107)

$$\mathbf{V} > \text{HData} := \text{LieAlgebraData}(\text{MrepMat}, h) : \text{DGsetup}(\text{HData});$$

*Lie algebra: h*

(108)

```
h > mrep:=Representation(h,m,MrepMat):
```

```
V > rho:=Adjoint(h,representationspace=h):
```

```
L1 > rep:=DirectSumOfRepresentations([rho,mrep],g);
```

[illegible]

$$\rightarrow \begin{bmatrix} 0 & 0 & 0 & 0 & 0 & 0 & 0 & 0 & 0 \\ 0 & 0 & 0 & 0 & 0 & 0 & 0 & 0 & 0 \\ 0 & 2 & 0 & 0 & 0 & 0 & 0 & 0 & 0 \\ 0 & 0 & 0 & 0 & 0 & 0 & 0 & 0 & 0 \\ 0 & 0 & 0 & 0 & 0 & 0 & 0 & 0 & 0 \\ 0 & 0 & 0 & 0 & -6 & 0 & 0 & 0 & 0 \\ 0 & 0 & 0 & 6 & 0 & 0 & 0 & 0 & 0 \\ 0 & 0 & 0 & 0 & 0 & 0 & 0 & 0 & 0 \\ 0 & 0 & 0 & 0 & 0 & 0 & 0 & 0 & 0 \end{bmatrix}$$

```
h > ChangeFrame(g);
```

*h* (110)

```
L1 > L2m:=GenerateForms([seq(dw|i,i=4..9)],2):L2mtg:=
GenerateTensors([L2m,[seq(D_w|i,i=1..9)])]:
L1 > brackets:=Invariants(rep,L2mtg):
L1 > nops(brackets);
```

6 (111)

The space of invariant brackets is 6D.

```
g > bracket:=evalDG(add(a||i*brackets[i],i=1..nops(brackets))):
g > repMat:=[seq(ApplyRepresentation(rep,e||i),i=1..3)]:
g > ChangeFrame(g);
```

*h* (112)

```
V80 > HTensor:=[seq(convert(repMat[i],DGtensor,[["con_bas",
"cov_bas"],[]]),i=1..nops(repMat))]:
V > A:=(x,y,z)->GetComponents(evalDG(ContractIndices(HTensor[x],
HTensor[y],[[2,1]])&minus ContractIndices(HTensor[y],HTensor
[x],[[2,1]])),HTensor)[z]:
V > B:=(x,y,z)->GetComponents(convert(evalDG(ContractIndices
(HTensor[x],D_w||y,[[2,1]])),DGvector),DGinfo(g,
"FrameBaseVectors"))[z]:
g > C:=(x,y,z)->GetComponents(convert(ContractIndices( evalDG
(D_w||x &t D_w||y), bracket,[[1,1],[2,2]]),DGvector),DGinfo
(g,"FrameBaseVectors"))[z]:
V > CH:=[seq(seq([q||i,q||j]=add(A(i,j,k)*q||k,k=1..nops(repMat)
),i=j+1..nops(repMat)),j=1..nops(repMat))]:
L2 > ChangeFrame(g);
```

*g* (113)

```
V > CHM:=[seq(seq([q||i,q||j]=add(B(i,j,k)*q||k,k=1..9),i=1..nops
(repMat)),j=4..9)]:
g > CM:=[seq(seq([q||i,q||j]=add(C(i,j,k)*q||k,k=1..9),j=i+1..9),
i=4..9)]:
V > KData:=LieAlgebraData([op(CH),op(CHM),op(CM)],[seq(q||i,i=1..
nops(repMat)+dimM)]);
```

*KData := [e1, e2]=0, [e1, e3]=0, [e1, e4]=e5, [e1, e5]=−e4, [e1, e6]=e7, [e1, e7]=*  
*−e6, [e1, e8]=−2e9, [e1, e9]=2e8, [e2, e3]=−2e3, [e2, e4]=e4, [e2, e5]=e5,*  
*[e2, e6]=−e6, [e2, e7]=−e7, [e2, e8]=0, [e2, e9]=0, [e3, e4]=6e7, [e3, e5]=*  
*−6e6, [e3, e6]=0, [e3, e7]=0, [e3, e8]=0, [e3, e9]=0, [e4, e5]=0, [e4, e6]=−a5e8*  
*−a4e9, [e4, e7]=−a6e1−a4e8+a5e9, [e4, e8]=a3e4+a2e5, [e4, e9]=a2e4*  
*−a3e5, [e5, e6]=a6e1−a4e8+a5e9, [e5, e7]=a5e8+a4e9, [e5, e8]=a2e4*  
*−a3e5, [e5, e9]=−a3e4−a2e5, [e6, e7]=0, [e6, e8]=−a3e6−a2e7, [e6, e9]=*  
*−a2e6+a3e7, [e7, e8]=−a2e6+a3e7, [e7, e9]=a3e6+a2e7, [e8, e9]=a1e1*

(114)

These are the most general structure constants for g.

```
L1 > DGsetup(KData);
```

*Lie algebra: L1* (115)

```
L1 > jaceq:=Query({seq(a||i,i=1..300)},"Jacobi");
h > jaceq[2];
{0, -a1 a4 + 2 a2 a6, a1 a4 - 2 a2 a6, -a1 a5 + 2 a3 a6, a1 a5 - 2 a3 a6, -2 a2 a5
+ 2 a3 a4, 2 a2 a5 - 2 a3 a4, -2 a2^2 - 2 a3^2 + a1, 2 a2^2 + 2 a3^2 - a1, -2 a2 a4
- 2 a3 a5 - a6, -2 a2 a4 - 2 a3 a5 + 2 a6, 2 a2 a4 + 2 a3 a5 - 2 a6, 2 a2 a4 + 2 a3 a5
+ a6}
```

(116)

```
h > sols:=solve(jaceq[2]);
sols := {a1 = 2 a2^2 + 2 a3^2, a2 = a2, a3 = a3, a4 = 0, a5 = 0, a6 = 0}, {a1 = 0, a2 = 0, a3 = 0, a4
= 0, a5 = a5, a6 = 0}, {a1 = 0, a2 = a2, a3 = RootOf(_Z^2 + 1) a2, a4 = a4, a5
= a4 RootOf(_Z^2 + 1), a6 = 0}
```

(117)

Only the first solution is non-flat and real.

```
h > KData2:=subs(sols[1],KData);
KData2 := [e1, e2]=0, [e1, e3]=0, [e1, e4]=e5, [e1, e5]=-e4, [e1, e6]=e7, [e1, e7]=
-e6, [e1, e8]=-2 e9, [e1, e9]=2 e8, [e2, e3]=-2 e3, [e2, e4]=e4, [e2, e5]=e5,
[e2, e6]=-e6, [e2, e7]=-e7, [e2, e8]=0, [e2, e9]=0, [e3, e4]=6 e7, [e3, e5]=
-6 e6, [e3, e6]=0, [e3, e7]=0, [e3, e8]=0, [e3, e9]=0, [e4, e5]=0, [e4, e6]=0, [e4,
e7]=0, [e4, e8]=a3 e4 + a2 e5, [e4, e9]=a2 e4 - a3 e5, [e5, e6]=0, [e5, e7]=0, [e5,
e8]=a2 e4 - a3 e5, [e5, e9]=-a3 e4 - a2 e5, [e6, e7]=0, [e6, e8]=-a3 e6 - a2 e7,
[e6, e9]=-a2 e6 + a3 e7, [e7, e8]=-a2 e6 + a3 e7, [e7, e9]=a3 e6 + a2 e7, [e8, e9
]=(2 a2^2 + 2 a3^2) e1
```

(118)

```
h > DGsetup(KData2);
Lie algebra: L1
```

(119)

```
L1 > Query("Jacobi");
true
```

(120)

```
h > LeviDecomposition();
[[e2, e3, e4, e5, e6, e7], [e1, e8, e9]]
```

(121)

Interestingly, g is not solvable, but has 3D Levi factor sl\_2.

```
h > Jtensor:=evalDG(e4 &t theta5 - e5 &t theta4 + e6 &t theta7 -
e7 &t theta6 + e8 &t theta9 -e9 &t theta8);
Jtensor := e4 ⊗ θ5 - e5 ⊗ θ4 + e6 ⊗ θ7 - e7 ⊗ θ6 + e8 ⊗ θ9 - e9 ⊗ θ8
```

(122)

```
L1 > Pm:=evalDG(add(e||i &t theta||i,i=4..9));
Pm := e4 ⊗ θ4 + e5 ⊗ θ5 + e6 ⊗ θ6 + e7 ⊗ θ7 + e8 ⊗ θ8 + e9 ⊗ θ9
```

(123)

```
L1 > NJ:=TensorBrackets(Jtensor,Jtensor,"Frolicher-Nijenhuis");
h > DGImageSpace(x->ContractIndices(evalDG(Pm &t x),NJ,[[2,1],[3,
2],[4,3]]),GenerateTensors([[e4,e5,e6,e7,e8,e9],[e4,e5,e6,e7,
e8,e9]]));
[-8 a3 e4 - 8 a2 e5, -8 a2 e4 + 8 a3 e5, 8 a3 e6 + 8 a2 e7, 8 a2 e6 - 8 a3 e7]
```

(124)

The image of the Nijenhuis tensor is at most 4D, so it is degenerate.

## Part 2.4: 3D isotropy L0

```
> restart:with(DifferentialGeometry): with(Tensor): with(Tools):
with(LieAlgebras):
```

```
h > dimM:=6;
```

*dimM:=6*

(125)

```
g > MrepMat := [Matrix(6, 6, {(1, 1) = 0, (1, 2) = 0, (1, 3) = 0,
(1, 4) = 0, (1, 5) = 0, (1, 6) = 0, (2, 1) = 0, (2, 2) = 0,
(2, 3) = 0, (2, 4) = 0, (2, 5) = 0, (2, 6) = 0, (3, 1) = 0,
(3, 2) = 0, (3, 3) = 0, (3, 4) = 0, (3, 5) = 1, (3, 6) = 0,
(4, 1) = 0, (4, 2) = 0, (4, 3) = 0, (4, 4) = 0, (4, 5) = 0,
(4, 6) = 1, (5, 1) = -1, (5, 2) = 0, (5, 3) = 0, (5, 4) = 0,
(5, 5) = 0, (5, 6) = 0, (6, 1) = 0, (6, 2) = -1, (6, 3) = 0,
(6, 4) = 0, (6, 5) = 0, (6, 6) = 0}), Matrix(6, 6, {(1, 1) =
0, (1, 2) = 0, (1, 3) = 0, (1, 4) = 0, (1, 5) = 0, (1, 6) =
0, (2, 1) = 0, (2, 2) = 0, (2, 3) = 0, (2, 4) = 0, (2, 5) =
0, (2, 6) = 0, (3, 1) = 0, (3, 2) = 0, (3, 3) = 0, (3, 4) =
0, (3, 5) = 0, (3, 6) = -3, (4, 1) = 0, (4, 2) = 0, (4, 3) =
0, (4, 4) = 0, (4, 5) = 3, (4, 6) = 0, (5, 1) = 0, (5, 2) =
-3, (5, 3) = 0, (5, 4) = 0, (5, 5) = 0, (5, 6) = 0, (6, 1) =
3, (6, 2) = 0, (6, 3) = 0, (6, 4) = 0, (6, 5) = 0, (6, 6) =
0}), Matrix(6, 6, {(1, 1) = 0, (1, 2) = 0, (1, 3) = 0, (1, 4) =
0, (1, 5) = 0, (1, 6) = 0, (2, 1) = 0, (2, 2) = 0, (2, 3) =
0, (2, 4) = 0, (2, 5) = 0, (2, 6) = 0, (3, 1) = 0, (3, 2) =
-6, (3, 3) = 0, (3, 4) = 0, (3, 5) = 0, (3, 6) = 0, (4, 1) =
6, (4, 2) = 0, (4, 3) = 0, (4, 4) = 0, (4, 5) = 0, (4, 6) =
0, (5, 1) = 0, (5, 2) = 0, (5, 3) = 0, (5, 4) = 0, (5, 5) =
0, (5, 6) = 0, (6, 1) = 0, (6, 2) = 0, (6, 3) = 0, (6, 4) =
0, (6, 5) = 0, (6, 6) = 0})]:
```

There are no parameters in the Lie algebra or representation.

```
m > DGsetup([seq(w||i,i=1..9)],g);
```

*frame name: g*

(126)

```
V > HData:=LieAlgebraData(MrepMat,h):DGsetup(HData);
```

*Lie algebra: h*

(127)

```
h > mrep:=Representation(h,m,MrepMat):
```

```
V > rho:=Adjoint(h,representationspace=h):
```

```
L1 > rep:=DirectSumOfRepresentations([rho,mrep],g);
```

$$rep := e1 \rightarrow \begin{bmatrix} 0 & 0 & 0 & 0 & 0 & 0 & 0 & 0 & 0 \\ 0 & 0 & 0 & 0 & 0 & 0 & 0 & 0 & 0 \\ 0 & 1 & 0 & 0 & 0 & 0 & 0 & 0 & 0 \\ 0 & 0 & 0 & 0 & 0 & 0 & 0 & 0 & 0 \\ 0 & 0 & 0 & 0 & 0 & 0 & 0 & 0 & 0 \\ 0 & 0 & 0 & 0 & 0 & 0 & 0 & 1 & 0 \\ 0 & 0 & 0 & 0 & 0 & 0 & 0 & 0 & 1 \\ 0 & 0 & 0 & -1 & 0 & 0 & 0 & 0 & 0 \\ 0 & 0 & 0 & 0 & -1 & 0 & 0 & 0 & 0 \end{bmatrix}, e2 \rightarrow \begin{bmatrix} 0 & 0 & 0 & 0 & 0 & 0 & 0 & 0 & 0 \\ 0 & 0 & 0 & 0 & 0 & 0 & 0 & 0 & 0 \\ -1 & 0 & 0 & 0 & 0 & 0 & 0 & 0 & 0 \\ 0 & 0 & 0 & 0 & 0 & 0 & 0 & 0 & 0 \\ 0 & 0 & 0 & 0 & 0 & 0 & 0 & 0 & 0 \\ 0 & 0 & 0 & 0 & 0 & 0 & 0 & 0 & -3 \\ 0 & 0 & 0 & 0 & 0 & 0 & 3 & 0 & 0 \\ 0 & 0 & 0 & 0 & -3 & 0 & 0 & 0 & 0 \\ 0 & 0 & 0 & 3 & 0 & 0 & 0 & 0 & 0 \end{bmatrix}, e3 \quad (128)$$

$$\rightarrow \begin{bmatrix} 0 & 0 & 0 & 0 & 0 & 0 & 0 & 0 & 0 \\ 0 & 0 & 0 & 0 & 0 & 0 & 0 & 0 & 0 \\ 0 & 0 & 0 & 0 & 0 & 0 & 0 & 0 & 0 \\ 0 & 0 & 0 & 0 & 0 & 0 & 0 & 0 & 0 \\ 0 & 0 & 0 & 0 & 0 & 0 & 0 & 0 & 0 \\ 0 & 0 & 0 & 0 & -6 & 0 & 0 & 0 & 0 \\ 0 & 0 & 0 & 6 & 0 & 0 & 0 & 0 & 0 \\ 0 & 0 & 0 & 0 & 0 & 0 & 0 & 0 & 0 \\ 0 & 0 & 0 & 0 & 0 & 0 & 0 & 0 & 0 \end{bmatrix}$$

```
h > ChangeFrame(g);
```

*h*

(129)

```
L1 > L2m:=GenerateForms([seq(dw| | i,i=4..9)],2):L2mtg:=  
GenerateTensors([L2m,[seq(D_w| | i,i=1..9)])]:
```

```
L1 > brackets:=Invariants(rep,L2mtg):
```

```
L1 > nops(brackets);
```

24

(130)

The space of invariant brackets is 24D.

```
g > bracket:=evalDG(add(a| | i*brackets[i],i=1..nops(brackets))):
```

```
g > repMat:=[seq(ApplyRepresentation(rep,e| | i),i=1..3)]:
```

```
g > ChangeFrame(g);
```

*h*

(131)

```
V80 > HTensor:=[seq(convert(repMat[i],DGtensor,[["con_bas",  
"cov_bas"],[]]),i=1..nops(repMat))]:
```

```
V > A:=(x,y,z)->GetComponents(evalDG(ContractIndices(HTensor[x],  
HTensor[y],[[2,1]])&minus ContractIndices(HTensor[y],HTensor  
[x],[[2,1]])),HTensor)[z]:
```

```
V > B:=(x,y,z)->GetComponents(convert(evalDG(ContractIndices  
(HTensor[x],D_w| | y,[[2,1]])),DGvector),DGinfo(g,  
"FrameBaseVectors"))[z]:
```

```
g > C:=(x,y,z)->GetComponents(convert(ContractIndices( evalDG  
(D_w| | x &t D_w| | y), bracket,[[1,1],[2,2]]),DGvector),DGinfo  
(g,"FrameBaseVectors"))[z]:
```

```
V > CH:=[seq(seq([q| | i,q| | j]=add(A(i,j,k)*q| | k,k=1..nops(repMat)  
) ,i=j+1..nops(repMat)),j=1..nops(repMat))]:
```

```
L2 > ChangeFrame(g);
```

*g*

(132)

```
V > CHM:=[seq(seq([q| | i,q| | j]=add(B(i,j,k)*q| | k,k=1..9),i=1..nops  
(repMat)),j=4..9)]:
```

```
g > CM:=[seq(seq([q| | i,q| | j]=add(C(i,j,k)*q| | k,k=1..9),j=i+1..9),  
i=4..9)]:
```

```
V > KData:=LieAlgebraData([op(CH),op(CHM),op(CM)],[seq(q| | i,i=1..  
nops(repMat)+dimM)]);
```

(133)

$$\begin{aligned}
KData := [e1, e2] = e3, [e1, e3] = 0, [e1, e4] = -e8, [e1, e5] = -e9, [e1, e6] = 0, [e1, e7] \\
= 0, [e1, e8] = e6, [e1, e9] = e7, [e2, e3] = 0, [e2, e4] = 3 e9, [e2, e5] = -3 e8, [e2, e6] \\
= 0, [e2, e7] = 0, [e2, e8] = 3 e7, [e2, e9] = -3 e6, [e3, e4] = 6 e7, [e3, e5] = -6 e6, \\
[e3, e6] = 0, [e3, e7] = 0, [e3, e8] = 0, [e3, e9] = 0, [e4, e5] = (3 a21 + 3 a10) e1 + (-a20 \\
+ a15) e2 + a24 e3 + (a17 - a6) e4 + (a16 + a7) e5 + a23 e6 + a22 e7 + (-a19 + a14) e8 \\
+ (-a18 + a13) e9, [e4, e6] = -a11 e3 + a16 e6 - a17 e7 - a5 e8 - a4 e9, [e4, e7] = \\
\left(\frac{a12}{3} + a3\right) e3 + (a17 + a2) e6 + (a16 + a1) e7 - a4 e8 + a5 e9, [e4, e8] = -a12 e1 \\
- a11 e2 + a21 e3 + a5 e4 + a4 e5 + (-a18 + a13 - a9) e6 - (-a19 + a14 + a8) e7 \\
+ a16 e8 - a17 e9, [e4, e9] = -3 a11 e1 + \frac{a12}{3} e2 + a20 e3 + a4 e4 - a5 e5 + a19 e6 \\
+ a18 e7 + a17 e8 + a16 e9, [e5, e6] = \left(\frac{a12}{3} - a3\right) e3 - (-a6 + a2) e6 - (a7 + a1) e7 \\
- a4 e8 + a5 e9, [e5, e7] = a11 e3 + a7 e6 + a6 e7 + a5 e8 + a4 e9, [e5, e8] = -3 a11 e1 \\
+ \frac{a12}{3} e2 + a15 e3 + a4 e4 - a5 e5 + a14 e6 + a13 e7 + a6 e8 - a7 e9, [e5, e9] \\
= a12 e1 + a11 e2 + a10 e3 - a5 e4 - a4 e5 + a9 e6 + a8 e7 + a7 e8 + a6 e9, [e6, e7] \\
= 0, [e6, e8] = -a5 e6 - a4 e7, [e6, e9] = -a4 e6 + a5 e7, [e7, e8] = -a4 e6 + a5 e7, \\
[e7, e9] = a5 e6 + a4 e7, [e8, e9] = a3 e3 + a2 e6 + a1 e7
\end{aligned} \tag{133}$$

These are the most general structure constants for g.

```
L1 > DGsetup(KData);
```

*Lie algebra: L1* (134)

```
h > jaceq:=Query({seq(a||i,i=1..300)}, "Jacobi");
h > complexsols:=solve(jaceq[2]);
h > nops({complexsols});
```

37 (135)

The solution families include complex structure constants. In spite of this, we compute the Nijenhuis tensor for all solutions (as it is difficult to find non-obvious real subfamilies of solutions). In those cases where a real subfamily exists, the Nijenhuis tensor will coincide.

```
h > for i from 1 to nops({complexsols}) do KD[i]:=subs
(complexsols[i],KData): end do:
h > Jtensor:=evalDG(e4 &t theta5 - e5 &t theta4 + e6 &t theta7 -
e7 &t theta6 + e8 &t theta9 -e9 &t theta8);
```

$$Jtensor := e4 \otimes \theta_5 - e5 \otimes \theta_4 + e6 \otimes \theta_7 - e7 \otimes \theta_6 + e8 \otimes \theta_9 - e9 \otimes \theta_8 \tag{136}$$

```
L1 > Pm:=evalDG(add(e||i &t theta||i,i=4..9));
```

$$Pm := e4 \otimes \theta_4 + e5 \otimes \theta_5 + e6 \otimes \theta_6 + e7 \otimes \theta_7 + e8 \otimes \theta_8 + e9 \otimes \theta_9 \tag{137}$$

```
L1 > for i from 1 to nops({complexsols}) do DGsetup(KD[i]):NJ[i]
:=TensorBrackets(Jtensor,Jtensor,"Frolicher-Nijenhuis");
end do:
h > for i from 1 to nops({complexsols}) do print(i);print
```

```
(DGImageSpace(x->ContractIndices(evalDG(Pm &t x),NJ[i],[[2,
1],[3,2],[4,3]]),GenerateTensors([[e4,e5,e6,e7,e8,e9],[e4,e5,
e6,e7,e8,e9]]))); end do:
```

1

$$\left[ \frac{1}{9 a l^2 + 24 a l a 7 + a^2 + 16 a 7^2} (4 (9 a l^2 a l 3 + 3 a l^2 a 9 + 21 a l a l 3 a 7 - 3 a l a l 4 a l 7 - 2 a l 4 a 2 a l + 9 a l a l 7 a 8 + 6 a l a 2 a 8 + 7 a l a 7 a 9 + 3 a l 3 a l 7 a 2 + 3 a l 3 a 2^2 + 12 a l 3 a 7^2 - 4 a l 4 a l 7 a 7 - 3 a l 4 a 2 a 7 + a l 7 a 2 a 9 + 12 a l 7 a 7 a 8 + a^2^2 a 9 + 9 a 2 a 7 a 8 + 4 a 7^2 a 9)) e 6 - \frac{1}{9 a l^2 + 24 a l a 7 + a^2 + 16 a 7^2} (4 (3 a l^2 a l 4 - 9 a l^2 a 8 + 9 a l a l 3 a l 7 + 6 a l a l 3 a 2 + 7 a l a l 4 a 7 + 3 a l a l 7 a 9 + 2 a l a 2 a 9 - 21 a l a 7 a 8 + 12 a l 3 a l 7 a 7 + 9 a l 3 a 2 a 7 + a l 4 a l 7 a 2 + a l 4 a 2^2 + 4 a l 4 a 7^2 - 3 a l 7 a 2 a 8 + 4 a l 7 a 7 a 9 - 3 a 2^2 a 8 + 3 a 2 a 7 a 9 - 12 a 7^2 a 8)) e 7, \right.$$

$$- \frac{1}{9 a l^2 + 24 a l a 7 + a^2 + 16 a 7^2} (4 (3 a l^2 a l 4 - 9 a l^2 a 8 + 9 a l a l 3 a l 7 + 6 a l a l 3 a 2 + 7 a l a l 4 a 7 + 3 a l a l 7 a 9 + 2 a l a 2 a 9 - 21 a l a 7 a 8 + 12 a l 3 a l 7 a 7 + 9 a l 3 a 2 a 7 + a l 4 a l 7 a 2 + a l 4 a 2^2 + 4 a l 4 a 7^2 - 3 a l 7 a 2 a 8 + 4 a l 7 a 7 a 9 - 3 a 2^2 a 8 + 3 a 2 a 7 a 9 - 12 a 7^2 a 8)) e 6$$

$$- \frac{1}{9 a l^2 + 24 a l a 7 + a^2 + 16 a 7^2} (4 (9 a l^2 a l 3 + 3 a l^2 a 9 + 21 a l a l 3 a 7 - 3 a l a l 4 a l 7 - 2 a l 4 a 2 a l + 9 a l a l 7 a 8 + 6 a l a 2 a 8 + 7 a l a 7 a 9 + 3 a l 3 a l 7 a 2 + 3 a l 3 a 2^2 + 12 a l 3 a 7^2 - 4 a l 4 a l 7 a 7 - 3 a l 4 a 2 a 7 + a l 7 a 2 a 9 + 12 a l 7 a 7 a 8 + a^2^2 a 9 + 9 a 2 a 7 a 8 + 4 a 7^2 a 9)) e 7]$$

2

$$[(4 a l 8 + 4 a 9) e 6 - (-4 a 8 + 4 a l 9) e 7, -(-4 a 8 + 4 a l 9) e 6 - (4 a l 8 + 4 a 9) e 7]$$

3

$$\left[ \frac{1}{a 7 (3 a l + 4 a 7)} (4 (3 a l a l 3 a 7 - 3 a l a l 4 a l 7 + 9 a l a l 7 a l 9 + a l a 7 a 9 - 9 a l 3 a l 7^2 + 3 a l 3 a 7^2 - 4 a l 4 a l 7 a 7 - 3 a l 7^2 a 9 + 12 a l 7 a l 9 a 7 + a 7^2 a 9)) e 6 \right.$$



$$\begin{aligned}
& - \frac{4 (a l a l 4 - 3 a l 9 a l + 3 a l 7 a l 3 + a l 4 a 7 + a l 7 a 9 - 3 a 7 a l 9)}{a 7} e 7, \\
& - \frac{4 (a l a l 4 - 3 a l 9 a l + 3 a l 7 a l 3 + a l 4 a 7 + a l 7 a 9 - 3 a 7 a l 9)}{a 7} e 6 \\
& - \frac{1}{a 7 (3 a l + 4 a 7)} (4 (3 a l a l 3 a 7 - 3 a l a l 4 a l 7 + 9 a l a l 7 a l 9 + a l a 7 a 9 \\
& - 9 a l 3 a l 7^2 + 3 a l 3 a 7^2 - 4 a l 4 a l 7 a 7 - 3 a l 7^2 a 9 + 12 a l 7 a l 9 a 7 + a 7^2 a 9)) e 7 \Big] \\
& 4
\end{aligned}$$

$$\begin{aligned}
& \Big[ - \frac{1}{a l (2 a l 7 + a 2)} (2 (a l^2 a l 4 - 2 a l^2 a l 9 - a l^2 a 8 + 4 a l 4 a l 7^2 + 8 a l 4 a l 7 a 2 \\
& + 4 a l 4 a 2^2 - 12 a l 7^2 a 8 - 4 a l 7 a l 9 a 2 - 20 a l 7 a 2 a 8 - 4 a l 9 a 2^2 - 8 a 2^2 a 8)) e 6 - \\
& \left( -4 a 8 + 4 a l 9 \right) e 7, - \left( -4 a 8 + 4 a l 9 \right) e 6 + \frac{1}{a l (2 a l 7 + a 2)} (2 (a l^2 a l 4 \\
& - 2 a l^2 a l 9 - a l^2 a 8 + 4 a l 4 a l 7^2 + 8 a l 4 a l 7 a 2 + 4 a l 4 a 2^2 - 12 a l 7^2 a 8 \\
& - 4 a l 7 a l 9 a 2 - 20 a l 7 a 2 a 8 - 4 a l 9 a 2^2 - 8 a 2^2 a 8)) e 7 \Big] \\
& 5
\end{aligned}$$

$$\begin{aligned}
& \Big[ \left( 4 a l 8 + 4 a 9 \right) e 6 \\
& + \frac{4 (a l^2 a l 4 - 3 a l^2 a l 9 + 3 a l a l 7 a l 8 + 3 a l a l 7 a 9 + a l 4 a l 7^2 - 3 a l 7^2 a l 9)}{3 a l 7^2} e 7, \\
& \frac{4 (a l^2 a l 4 - 3 a l^2 a l 9 + 3 a l a l 7 a l 8 + 3 a l a l 7 a 9 + a l 4 a l 7^2 - 3 a l 7^2 a l 9)}{3 a l 7^2} e 6 - \\
& \left( 4 a l 8 + 4 a 9 \right) e 7 \Big]
\end{aligned}$$

$$\begin{aligned}
& 6 \\
& \Big[ \left( 4 a l 8 + 4 a 9 \right) e 6 + \left( \frac{4 a l 4}{3} - 4 a l 9 \right) e 7, \left( \frac{4 a l 4}{3} - 4 a l 9 \right) e 6 - \left( 4 a l 8 + 4 a 9 \right) e 7 \Big] \\
& 7 \\
& [(4 a l 8 + 4 a 9) e 6 - (-4 a 8 + 4 a l 9) e 7, -(-4 a 8 + 4 a l 9) e 6 - (4 a l 8 + 4 a 9) e 7] \\
& 8
\end{aligned}$$

$$\begin{aligned}
& \Big[ - \frac{1}{3 a l + 4 a 7} (4 (RootOf(_Z^2 + 1) a l a l 4 - 3 RootOf(_Z^2 + 1) a l a l 9 + RootOf(_Z^2 \\
& + 1) a l 4 a 7 - 4 RootOf(_Z^2 + 1) a l 9 a 7 + RootOf(_Z^2 + 1) a 7 a 8 - 3 a l 3 a l - a 9 a l \\
& - 3 a 7 a l 3 - a 9 a 7)) e 6 - (-4 a 8 + 4 a l 9) e 7, - \left( -4 a 8 + 4 a l 9 \right) e 6 \\
& + \frac{1}{3 a l + 4 a 7} (4 (RootOf(_Z^2 + 1) a l a l 4 - 3 RootOf(_Z^2 + 1) a l a l 9
\end{aligned}$$

$$+ \text{RootOf}(\_Z^2 + 1) a14 a7 - 4 \text{RootOf}(\_Z^2 + 1) a19 a7 + \text{RootOf}(\_Z^2 + 1) a7 a8 - 3 a13 a1 - a9 a1 - 3 a7 a13 - a9 a7)) e7]$$

9

$$\left[ -\frac{1}{3(3a1 + 4a7)} (4(3 \text{RootOf}(\_Z^2 + 1) a1 a14 - 9 \text{RootOf}(\_Z^2 + 1) a1 a19 + 9 \text{RootOf}(\_Z^2 + 1) a13 a17 + 4 \text{RootOf}(\_Z^2 + 1) a14 a7 + 3 \text{RootOf}(\_Z^2 + 1) a17 a9 - 12 \text{RootOf}(\_Z^2 + 1) a19 a7 - 27 a13 a1 - 9 a9 a1 - 33 a7 a13 - 11 a9 a7)) e6 - \left( -\frac{4a14}{3} + 4 \text{RootOf}(\_Z^2 + 1) a13 + \frac{4 \text{RootOf}(\_Z^2 + 1) a9}{3} + 4 a19 \right) e7, -\left( -\frac{4a14}{3} + 4 \text{RootOf}(\_Z^2 + 1) a13 + \frac{4 \text{RootOf}(\_Z^2 + 1) a9}{3} + 4 a19 \right) e6 + \frac{1}{3(3a1 + 4a7)} (4(3 \text{RootOf}(\_Z^2 + 1) a1 a14 - 9 \text{RootOf}(\_Z^2 + 1) a1 a19 + 9 \text{RootOf}(\_Z^2 + 1) a13 a17 + 4 \text{RootOf}(\_Z^2 + 1) a14 a7 + 3 \text{RootOf}(\_Z^2 + 1) a17 a9 - 12 \text{RootOf}(\_Z^2 + 1) a19 a7 - 27 a13 a1 - 9 a9 a1 - 33 a7 a13 - 11 a9 a7)) e7]$$

10

$$\left[ \left( 4a18 + 4a9 \right) e6 - \left( -\frac{4a14}{3} + 4 \text{RootOf}(\_Z^2 + 1) a13 + \frac{4 \text{RootOf}(\_Z^2 + 1) a9}{3} + 4 a19 \right) e7, -\left( -\frac{4a14}{3} + 4 \text{RootOf}(\_Z^2 + 1) a13 + \frac{4 \text{RootOf}(\_Z^2 + 1) a9}{3} + 4 a19 \right) e6 - \left( 4a18 + 4a9 \right) e7 \right]$$

11

$$[(4a18 + 4a9) e6 - (-4a8 + 4a19) e7, -(-4a8 + 4a19) e6 - (4a18 + 4a9) e7]$$

12

$$[-(-4 \text{RootOf}(\_Z^2 + 1) a14 + 12 \text{RootOf}(\_Z^2 + 1) a8 + 12 a13 - 4 a18) e6 - (-4 a8 + 4 a19) e7, -(-4 a8 + 4 a19) e6 + (-4 \text{RootOf}(\_Z^2 + 1) a14 + 12 \text{RootOf}(\_Z^2 + 1) a8 + 12 a13 - 4 a18) e7]$$

13

$$\left[ \frac{1}{2 \text{RootOf}(\_Z^2 + 1) a7 - a2} (2(3 a13 \text{RootOf}(\_Z^2 + 1) a7 - a17 a14 \text{RootOf}(\_Z^2 + 1) + 3 \text{RootOf}(\_Z^2 + 1) a17 a8 - 2 a19 \text{RootOf}(\_Z^2 + 1) a2 + 2 a8 \text{RootOf}(\_Z^2 + 1) a2 + \text{RootOf}(\_Z^2 + 1) a7 a9 + 3 a17 a13 + a14 a7 + a17 a9 - 4 a7 a19 + a7 a8)) e6 - ($$

$$-4 a8 + 4 a19) e7, - \left( -4 a8 + 4 a19 \right) e6$$

$$- \frac{1}{2 \operatorname{RootOf}(\_Z^2 + 1) a7 - a2} (2 (3 a13 \operatorname{RootOf}(\_Z^2 + 1) a7 - a17 a14 \operatorname{RootOf}(\_Z^2 + 1) + 3 \operatorname{RootOf}(\_Z^2 + 1) a17 a8 - 2 a19 \operatorname{RootOf}(\_Z^2 + 1) a2 + 2 a8 \operatorname{RootOf}(\_Z^2 + 1) a2 + \operatorname{RootOf}(\_Z^2 + 1) a7 a9 + 3 a17 a13 + a14 a7 + a17 a9 - 4 a7 a19 + a7 a8) e7]$$

14

$$[(4 a18 + 4 a9) e6 - (-4 a8 + 4 a19) e7, -(-4 a8 + 4 a19) e6 - (4 a18 + 4 a9) e7]$$

15

$$[(4 a18 + 4 a9) e6 - (-4 a8 + 4 a19) e7, -(-4 a8 + 4 a19) e6 - (4 a18 + 4 a9) e7]$$

16

$$[4 \operatorname{RootOf}(\_Z^2 + 1) (a19 - a8) e6 - (-4 a8 + 4 a19) e7]$$

17

$$\left[ \left( 4 a18 + 4 a9 \right) e6 - \frac{1}{a2 (2 a1 + 3 a7)} (4 (3 a1^2 a13 - 3 a1^2 a18 - 2 a1^2 a9 + 6 a1 a13 a7 - 7 a1 a18 a7 - 5 a1 a7 a9 + 3 a13 a2^2 + 3 a13 a7^2 - a18 a2^2 - 4 a18 a7^2 - 3 a7^2 a9)) e7, - \frac{1}{a2 (2 a1 + 3 a7)} (4 (3 a1^2 a13 - 3 a1^2 a18 - 2 a1^2 a9 + 6 a1 a13 a7 - 7 a1 a18 a7 - 5 a1 a7 a9 + 3 a13 a2^2 + 3 a13 a7^2 - a18 a2^2 - 4 a18 a7^2 - 3 a7^2 a9)) e6 - \left( 4 a18 + 4 a9 \right) e7 \right]$$

18

$$\left[ \left( 4 a18 + 4 a9 \right) e6 - \frac{4 (a1 a14 - 3 a19 a1 + a14 a7 - 3 a7 a19)}{a7} e7, - \frac{4 (a1 a14 - 3 a19 a1 + a14 a7 - 3 a7 a19)}{a7} e6 - \left( 4 a18 + 4 a9 \right) e7 \right]$$

19

$$[(4 a18 + 4 a9) e6 - (-4 a8 + 4 a19) e7, -(-4 a8 + 4 a19) e6 - (4 a18 + 4 a9) e7]$$

20

[ ]

21

$$[(4 a18 + 4 a9) e6 - (-4 a8 + 4 a19) e7, -(-4 a8 + 4 a19) e6 - (4 a18 + 4 a9) e7]$$

22

$$[(4 a18 + 4 a9) e6 - (-4 a8 + 4 a19) e7, -(-4 a8 + 4 a19) e6 - (4 a18 + 4 a9) e7]$$

23

$$[(4 a18 + 4 a9) e6 - (-4 a8 + 4 a19) e7, -(-4 a8 + 4 a19) e6 - (4 a18 + 4 a9) e7]$$

24

$$\left[ -\frac{a14 a16^2 + a14 a6^2 - 3 a16^2 a8 - 4 a19 a6^2 + a6^2 a8}{a16 a6} e6 - \left( -4 a8 + 4 a19 \right) e7, - \left( -4 a8 + 4 a19 \right) e6 + \frac{a14 a16^2 + a14 a6^2 - 3 a16^2 a8 - 4 a19 a6^2 + a6^2 a8}{a16 a6} e7 \right]$$

25

$$[(4 a18 + 4 a9) e6 - (-4 a8 + 4 a19) e7, -(-4 a8 + 4 a19) e6 - (4 a18 + 4 a9) e7]$$

26

$$[(4 a18 + 4 a9) e6 - (-4 a8 + 4 a19) e7, -(-4 a8 + 4 a19) e6 - (4 a18 + 4 a9) e7]$$

27

$$[-4 \text{RootOf}(\_Z^2 + 1) (a19 - a8) e6 - (-4 a8 + 4 a19) e7]$$

28

$$[(4 a18 + 4 a9) e6 - (-4 a8 + 4 a19) e7, -(-4 a8 + 4 a19) e6 - (4 a18 + 4 a9) e7]$$

29

$$[(4 a18 + 4 a9) e6 - (-4 a8 + 4 a19) e7, -(-4 a8 + 4 a19) e6 - (4 a18 + 4 a9) e7]$$

30

$$\left[ \left( 4 a18 + 4 a9 \right) e6 + \frac{2 (a1^2 a14 - 3 a1^2 a19 + 2 a1 a18 a2 + 2 a1 a2 a9 + a14 a2^2 - 3 a19 a2^2)}{a2^2} e7, \frac{2 (a1^2 a14 - 3 a1^2 a19 + 2 a1 a18 a2 + 2 a1 a2 a9 + a14 a2^2 - 3 a19 a2^2)}{a2^2} e6 - \left( 4 a18 + 4 a9 \right) e7 \right]$$

31

$$\left[ \left( 4 a18 + 4 a9 \right) e6 + \frac{2 (a1^2 a14 - 3 a1^2 a19 + 2 a1 a18 a2 + 2 a1 a2 a9 + a14 a2^2 - 3 a19 a2^2)}{a2^2} e7, \frac{2 (a1^2 a14 - 3 a1^2 a19 + 2 a1 a18 a2 + 2 a1 a2 a9 + a14 a2^2 - 3 a19 a2^2)}{a2^2} e6 - \left( 4 a18 + 4 a9 \right) e7 \right]$$

32

$$[(4 a18 + 4 a9) e6 - (-4 a8 + 4 a19) e7, -(-4 a8 + 4 a19) e6 - (4 a18 + 4 a9) e7]$$

33

$$[(4 a18 + 4 a9) e6 - (-4 a8 + 4 a19) e7, -(-4 a8 + 4 a19) e6 - (4 a18 + 4 a9) e7]$$

34

$$[(4 a18 + 4 a9) e6 + 4 \text{RootOf}(\_Z^2 + 1) (a18 + a9) e7]$$

35

$$\frac{[(4 a18 + 4 a9) e6 + 4 \text{RootOf}(\_Z^2 + 1) (a18 + a9) e7]}{36}$$

$$\frac{[(4 a18 + 4 a9) e6 - 4 \text{RootOf}(\_Z^2 + 1) (a18 + a9) e7]}{37}$$

$$[8 a5 e8 + 8 \text{RootOf}(\_Z^2 + 1) a5 e9, -8 a5 e4 - 8 \text{RootOf}(\_Z^2 + 1) a5 e5 + 4 \text{RootOf}(\_Z^2 + 1) (a19 - a8) e6 - (-4 a8 + 4 a19) e7, 8 a5 e6 + 8 \text{RootOf}(\_Z^2 + 1) a5 e7] \quad (138)$$

We note that none of these Nijenhuis tensors (besides case 37, which has explicitly complex structure constants) have image which spans  $\mathfrak{m}$ . Hence they are degenerate.

```
L1 > realsols:=RealDomain[solve](jaceq[2]):
```

```
L1 > nops({realsols});
```

18

(139)

Maple finds 18 families of explicitly real structure constants, however it is difficult to ensure that this is exhaustive.
